# Supplementary material for: Nonlinear Diffusion and Decay of an Expanding Turbulent Blob
Source: arXiv:2505.22737 source file (2025-06-27)
Supplement: Supplementary file 1 [file supplemental.pdf]

# Nonlinear Diffusion and Decay of an Expanding Turbulent Blob
# Supplementary Information

Takumi Matsuzawa

*James Franck Institute and Department of Physics,
University of Chicago, Chicago, IL 60637, USA and*

*Present address: Laboratory of Atomic and Solid-State
Physics, Cornell University, Ithaca, NY, USA*

Minhui Zhu

*Department of Physics, University of Illinois at Urbana-Champaign,
Loomis Laboratory of Physics, 1110 West Green Street,
Urbana, Illinois 61801-3080, USA and*

*Data Science and Learning Division, Argonne National Laboratory, Lemont, Illinois 60439, USA*

Nigel Goldenfeld

*Department of Physics, University of California, San Diego,
9500 Gilman Drive, La Jolla, California 92093, USA*

William T.M. Irvine

*James Franck Institute and Department of Physics,
University of Chicago, Chicago, IL 60637, USA and*

*Enrico Fermi Institute, University of Chicago, Chicago, IL 60637, USA*

(Dated: May 30, 2025)

**CONTENTS**


I. Symbols 4

II. Theory: A Nonlinear Diffusion Model 6
A. History of phenomenological models 6
B. Minimal model based on Kolmogorov's similarity hypotheses 7
C. Special case assuming instantaneous eddy adaptation 8
1. Self-similar asymptotics 9
2. A heuristic calculation recovering 1st order perturbative RG 10
3. Sharp front and non-diffusive propagation 12
4. Energy decay 14
D. Generalized theory motivated by experimental observations 14
1. Approximately self-similar asymptotics 15
2. Zeroth order system 17
3. Behaviors in the approximately self-similar regime for delayed eddy adaptation 17

III. Simulations: Cell Dynamical System Method 20
A. Overview of the CDS method 20
B. CDS algorithm for the Kolmogorov-Barenblatt turbulent energy balance equation 21
C. Benchmark of the method 23
D. Boundary condition 24
E. Summary of CDS Simulations and corresponding parameters used 24

IV. Experiments 25
A. Experimental methods 25
1. Flow chamber 25
2. Actuation 25
3. PIV experiments 27
4. Logarithmic triggering to capture decay 28
B. Summary of experimental runs 30
C. Data analysis 31
1. Analysis pipeline 31
2. Velocity fluctuations and convergence of mean flow 32
3. Virtual Origin Determination 33
4. Estimation of dissipation rate 34

V. Nonlinear Diffusion of a Turbulent Blob 38
A. Spatiotemporal evolution of the turbulent energy on a two-dimensional slice 38
B. Evolution of the second moment of the turbulent kinetic energy 39
C. Evolution of the azimuthally averaged turbulent kinetic energy front shape 41
D. $\dot{R}_{\text{blob}} - q$ scaling 43
E. Energy decay: capturing the effects of persistent inhomogeneity by decreasing the value of $c_0$ 44

VI. Dimensionless dissipation rate: comparison with literature values 47

VII. Turbulence Generated by a Single Oscillating Grid 48
A. Temporal evolution 48
B. Energy decay and integral length scale 48

C. Turbulence statistics 48

VIII. Supplementary Movies 52
Video 1: Expansion of a small turbulent blob ($Re_\lambda = 60$): energy 52
Video 2: Expansion of a small turbulent blob ($Re_\lambda = 60$): enstrophy 52
Video 3: Evolution of rescaled energy spectrum during decay (Large blob, $Re_\lambda = 203$) 52
Video 4: Decay of a large turbulent blob ($Re_\lambda = 203$): energy 52
Video 5: Decay of a large turbulent blob ($Re_\lambda = 203$): enstrophy 53
Video 6: Decomposition of energy and enstrophy into mean and fluctuating components (Large blob, $Re_\lambda = 203$) 53
Video 7: Spatiotemporal evolution of mean flow energy (Large Blob, $Re_\lambda = 203$) 53
Video 8: Pathline visualization of a decaying turbulent blob (Large blob, $Re_\lambda = 203$) 53
Video 9: Decay of turbulence initiated by a double oscillating grid ($Re_\lambda = 185$): energy 54
Video 10: Decay of turbulence initiated by a double oscillating grid ($Re_\lambda = 185$): enstrophy 54
Video 11: Decomposition of energy and enstrophy fields into mean flow and fluctuations (Double oscillating grid, $Re_\lambda = 185$) 54
Video 12: Evolution of rescaled energy spectrum during decay (Double oscillating grid, $Re_\lambda = 185$) 55
Video 13: Spatiotemporal evolution of mean flow energy (Double oscillating grid, $Re_\lambda = 185$) 55
Video 14: Spatiotemporal evolution of mean flow energy (Single oscillating grid, $Re_\lambda = 95$) 55
Video 15: 3D pathline visualization of an expanding and decaying turbulent blob (small blob, $Re_\lambda = 60$) 55

References 56

## I. SYMBOLS

In this subsection we summarize the symbols and conventions used in the main text and SI. In reporting experimental measurements, we define an ensemble average of n experimental runs as:

$$\langle U_i \rangle_{\mathrm{n}}(x_j,t) = \frac{1}{\mathrm{n}} \sum_{k=1}^{\mathrm{n}} U_i^{(k)}(x_j,t). \tag{1}$$

Here $U_i^{(k)}(x_j,t)$ refers to the measured velocity field of the $k$-th run of an experiment conducted with the same conditions.

We denote a spatial average by a subscript $\mathbf{x}$:

$$\langle U_i \rangle_{\mathbf{x}}(t) = \frac{1}{\mathcal{V}} \int_{\mathcal{V}} U_i(x_j,t) d^n x_j \tag{2}$$

where $n$ matches the number of dimensions of the measurement and $\mathcal{V}$ represents the entire domain being averaged over. For example, a radial profile is obtained by averaging over polar and azimuthal angles. Using the bracket notation, this is expressed as follows:

$$\langle U_i \rangle_{\theta\phi}(r,t) = \frac{1}{4\pi} \int_0^{\pi} \int_0^{2\pi} U_i(r,\theta',\phi',t) r^2 \sin\theta' d\theta' d\phi' \tag{3}$$

The above averaging procedures can be combined. For instance, the ensemble averaged radial profile of an expanding turbulent blob (main Figure 5) corresponds to: $q(r,t) = \langle q \rangle_{\theta\phi\mathrm{n}}(r,t)$.

We define the mean flow as the ensemble-averaged flow where the ensemble is generated by repeating the experiment under identical conditions. The turbulent velocity field $u_i(x_j,t)$, is then given by:

$$u_i(x_j,t) = U_i(x_j,t) - \langle U_i \rangle_{\mathrm{n}}(x_j,t). \tag{4}$$

TABLE I: Nomenclature

| | **Basics** |
|---|---|
| $Re$ | Reynolds number, $Re = u'\ell/\nu$ |
| $Re_\lambda$ | Taylor Reynolds number, $Re_\lambda = u'\lambda/\nu$ |
| $d$ | Spatial dimension |
| $t$ | Time |
| $t_0$ | Virtual origin (time) |
| $U_i$ | The $i$-th component of a velocity field |
| $U_{\mathrm{rms}}$ | RMS velocity, $U_{\mathrm{rms}} = (1/d)\sqrt{U_i U_i}$ for $i = 1, ..., d$ |
| $u_i$ | The $i$-th component of a fluctuating velocity field, or a velocity field in a general context |
| $u'$ | One-component fluctuating RMS velocity, $u' = (1/d)\sqrt{u_i u_i}$ for $i = 1, ..., d$ |
| $\Omega_i$ | the $i$-th component of a vorticity field |
| $\omega_i$ | The $i$-th component of a vorticity of a fluctuating velocity field, or vorticity of a general velocity field |
| $\rho$ | Density of a fluid |
| $\nu$ | Kinematic viscosity |
| $x, y, z$ | Cartesian coordinates |
| $r, \theta, \phi$ | Spherical coordinates |
| $\vec{\kappa}, \kappa_i$ | Wavenumber |
| | **Symbols** |

| | |
|---|---|
| $\langle A\rangle_{\mathrm{n}}$ | Ensemble average of $A$, |
| $\langle A\rangle_{\mathbf{x}}$ | Spatial average of $A(x_i)$, $\langle A\rangle_{\mathbf{x}} = \frac{1}{V}\int_{\mathcal{V}} A(x_i)dV$ |
| $\langle A\rangle_{\phi}$ | Azimuthal average of $A(r,\theta,\phi)$ in spherical coordinates, $\langle A\rangle_{\phi} = \frac{1}{2\pi}\int_0^{2\pi} A(r,\theta,\phi)r^2\sin\theta d\phi$ |
| $\langle A\rangle_{\theta}$ | Polar average of $A(r,\theta,\phi)$ in spherical coordinates, $\langle A\rangle_{\theta} = \frac{1}{\pi}\int_0^{\pi} A(r,\theta,\phi)r^2\sin\theta d\theta$ |

**Theory**

| | |
|---|---|
| $q$ | Turbulent energy density |
| $Q$ | Total turbulent energy |
| $Q_a$ | Total turbulent energy at $t=0$ |
| $h$ | Front position |
| $a$ | Front position at $t=0$; $h(t=0)=a$ |
| $c_0$ | Dimensionless transport coefficient |
| $\ell$ | Integral length scale |
| $\alpha$ | Ratio of $\ell$ and $h$ under instantaneous eddy adaptation assumption: $\ell = \alpha h$ |
| $\beta$ | $\beta = 2/(d+4)$ |
| $\gamma$ | Exponent of growth of integral length scale, $\ell \sim t^{\gamma}$ |
| $\epsilon$ | Dissipation rate |
| $\epsilon_0$ | Dimensionless dissipation coefficient |
| $\kappa_q$ | Diffusion coefficient |
| $\theta$ | $\theta = 2/(d+2)$ |
| $\vartheta$ | Exponent for $h$ under delayed eddy adaptation assumption $\vartheta = \beta(1+\gamma)$ |

**Experiments: Experimental methods**

| | |
|---|---|
| $A$ | Forcing amplitude (stroke length) |
| $D_{\mathrm{box}}$ | Diameter of a hole on the top face of the experimental chamber |
| $D_{\mathrm{grid}}$ | Diameter of a circular grid |
| $D_o$ | Diameter of an orifice |
| $D_p$ | Diameter of a piston |
| $L/D$ | Formation number of a vortex ring [1] |
| $L_{\mathrm{box}}$ | Width of an experimental chamber |
| $M$ | Mesh size of a grid |
| $f$ | Forcing frequency |
| $\ell_{\mathrm{sep}}$ | Separation length between the grids |
| $v_{\mathrm{eff}}$ | Effective stroke velocity [2] |
| $\Delta$ | Temporal interval that is used in PIV experiments |

**Experiments: Data analysis**

| | |
|---|---|
| $D_{LL}(r,t)$ | Second-order longitudinal structure function |
| $E(\kappa,t)$ | 3D energy spectrum |
| $E_{ij}(\kappa_1,t)$ | One-dimensional turbulent energy spectrum along $x_1$ |
| $\mathcal{E}$ | Raw energy, $\frac{1}{2}U_iU_i$ ($i=1,2$ for PIV measurements). |
| $\overline{\mathcal{E}}$ | Mean flow energy, $\frac{1}{2}\langle U_i\rangle\langle U_i\rangle$ |
| $\ell$ | Integral length scale, $\ell = (3\pi/4)\int \kappa^{-1}E(\kappa,t)d\kappa/\int E(\kappa,t)d\kappa$ |
| $n$ | Decay exponent of turbulent energy: : $\langle q\rangle_{\mathbf{x},\mathrm{n}}(t) = c(t-t_0)^n$ |
| $q$ | Fluctuating energy, $\frac{1}{2}u_iu_i$ |
| $\overline{r}, r_1, r_2$ | Coefficient of determination of linear regression |
| $t_a, t_b$ | Fit region for linear regression; $t_a < t_b$ |
| $t_0$ | Virtual origin for turbulent energy: $\langle q\rangle_{\mathbf{x},\mathrm{n}}(t) = c(t-t_0)^n$ |
| $\epsilon$ | Dissipation rate |
| $\epsilon_{E_{11}}$ | Dissipation rate obtained by fitting an energy spectrum |
| $\epsilon_{D_{LL}}$ | Dissipation rate obtained by fitting a structure function |
| $\epsilon_{dq/dt}$ | Dissipation rate obtained through turbulent energy $\langle q\rangle_{\mathbf{x},n}$ |
| $\epsilon_{s_{ij}}$ | Dissipation rate obtained through a rate-of-strain tensor |
| $\eta$ | Kolmogorov length scale, $\eta = (\nu^3/\epsilon)^{1/4}$ |

| | |
|---|---|
| $\lambda$ | Taylor microscale, $\lambda = \sqrt{15\nu u'^2/\epsilon}$ |

| | **Nonlinear Diffusion of a Turbulent Blob** |
|---|---|
| $R_{\rm blob}$ | Characteristic blob radius, $R_{\rm blob} = \int r^4 \langle q \rangle_{\theta\phi,\rm n}(r,t)dr / \int r^2 \langle q \rangle_{\theta\phi,\rm n}(r,t)dr$ |
| $q_0$ | Turbulent energy within the central region of the blob |
| $\delta q_1$ | Contributions to the rate of change of turbulent energy $q$ from transport |
| $\delta q_2$ | Contributions to the rate of change of turbulent energy $q$ from dissipation |
| $\gamma$ | Exponent of growth of integral length scale, $\ell \sim t^\gamma$ |

## II. THEORY: A NONLINEAR DIFFUSION MODEL

In this section, we give a detailed formulation of the theoretical model for the decay and propagation of a turbulent blob. We begin by reviewing the history of modeling fully developed turbulence using minimal PDEs. We begin by examining a special case that assume instantaneous eddy adaptation to the expanding turbulence domain ($\ell = \alpha h$), and extend previous work on the analytical properties and asymptotic behavior of the model from the 1D case to an arbitrary dimension $d$. Next, motivated by experimental observations, we develop a generalized model that moves beyond the instantaneous adaptation assumption and conduct the detailed asymptotic analysis when $\ell$ follows a general power-law scaling asymptotically. Finally, we present the cell dynamical system (CDS) method used in this paper, an efficient and accurate numerical method for simulating this family of models.

### A. History of phenomenological models

In 1942, Kolmogorov pioneered the idea that large-scale motion in fully developed turbulence could be described by mean-field partial differential equations (PDEs) [3]. He proposed a system of kinetic equations for the fluctuating turbulent energy, $b \equiv \sum_i u_i^2/3$ where $i$ denotes Cartesian component and $u_i$ is the $i$-th component of the velocity fluctuation (note that later we will define a slightly different normalization of the fluctuation kinetic energy $q = 3b/2$ in our notation), and for a mean frequency $\omega$ proportional to $b^{1/2}/\ell$:

$$\frac{D\bar{v}_i}{Dt} = F_i - \frac{\partial}{\partial x_i}\left(\frac{\bar{p}}{\rho} + b\right) + A\sum_j \frac{\partial}{\partial x_j}\left[\frac{b}{\omega}\left(\frac{\partial \bar{v}_i}{\partial x_j} + \frac{\partial \bar{v}_j}{\partial x_i}\right)\right], \tag{5}$$

$$\frac{D\omega}{Dt} = -\frac{7}{11}\omega^2 + A'\sum_j \frac{\partial}{\partial x_j}\left[\frac{b}{\omega}\frac{\partial \omega}{\partial x_j}\right], \tag{6}$$

$$\frac{Db}{Dt} = -b\omega + \frac{1}{3}A\frac{b}{\omega}\epsilon + A''\sum_j \frac{\partial}{\partial x_j}\left[\frac{b}{\omega}\frac{\partial b}{\partial x_j}\right]. \tag{7}$$

Notice that Eq. (6) and (7) are independent of $\bar{v}$, forming a closure by themselves. Therefore, we treat them as a two-equation model for the turbulent energy field.

Despite this elegant formulation, Kolmogorov acknowledged the challenge of solving two coupled PDEs both with spatial and temporal dependence. Subsequently, various PDEs have been proposed for turbulence modeling [4–8], generally adhering to the principles laid out by Kolmogorov.

In the 1980s, Barenblatt *et al.* [9–11] investigated the self-similarity and other analytical properties of two possible models for an isolated turbulence patch spreading freely in 1D. One of these models is the two-equation "$b-\epsilon$" model (or $q-\epsilon$), a coupled system of the turbulent energy density and the dissipation rate:

$$\partial_t b = \alpha \partial_z \left[ \frac{b^2}{\epsilon} \partial_z b \right] - \epsilon$$
$$\partial_t \epsilon = \beta \partial_z \left[ \frac{b^2}{\epsilon} \partial_z \epsilon \right] - \gamma \frac{\epsilon^2}{b}. \tag{8}$$

The other model is the one-equation "$b-\ell$" model (or $q-\ell$):

$$\partial_t b = \partial_z (\ell \sqrt{b} \partial_z b) - c_1 \frac{b^{3/2}}{\ell} \tag{9}$$

This one-equation model can also be derived from the energy balance equation in the two-equation model by assuming that $\epsilon \propto b^{3/2}/\ell$, which is the turbulence dissipation relation. Although the one-equation model has a simpler form, it leaves the length scale $\ell$ undetermined. In order to close the "$b-\ell$" model, Barenblatt *et al.* made a straightforward assumption to determine $\ell$ from the instantaneous distribution of turbulent energy, achieving the lowest closure among all models. His closure was that $\ell$ is proportional to the instantaneous linear dimension of the turbulence region. Building on this lineage, the "$b-\ell$" model serves as the starting point of our turbulence blob theory, which ultimately extends beyond the assumption mentioned above.

There are two comments that we wish to make about Eq. (9). First, the model leads to predictions for the propagation of turbulence that scale with power laws that cannot be deduced by simple dimensional considerations: what Barenblatt calls intermediate asymptotics of the second kind [9–11]. These were shown to be anomalous dimensions in a renormalization group theory [12]. We discuss this in more detail in Sec. II C.

Second, in the case of homogeneous turbulence, Eq. (9) predicts that the turbulent kinetic energy will decay in time with a power law given by setting all spatial derivatives to zero in Eq. (9), yielding:

$$q(t) \sim t^{-2}. \tag{10}$$

We note that in homogeneous isotropic turbulence, the RMS vorticity $\omega$ is related to $q(t)$ via: [13]

$$\frac{dq}{dt} = -\nu\omega^2 \propto -\frac{q^{3/2}}{\ell}, \tag{11}$$

leading to a prediction for the vorticity decay:

$$\omega \sim t^{-3/2} \tag{12}$$

under the assumption that $\ell$ is time-independent. This prediction was subsequently verified in pioneering experiments in superfluid helium [14].

### B. Minimal model based on Kolmogorov's similarity hypotheses

Rooted in Kolmogorov's seminal work [3] and comprehensively studied by Barenblatt *et al.* [9–11], a minimal one-equation model for the large-scale dynamics of an isolated free turbulent blob consists of a transport term and a dissipation term:

$$\partial_t q = \nabla \cdot (\kappa_q \nabla q) - \epsilon \tag{13}$$

where $\kappa_q$ is the diffusion coefficient and $\epsilon$ the energy dissipation rate. The second Kolmogorov similarity hypothesis states that in fully developed turbulence, the momentum exchange coefficient and the dissipation rate only depend on the local turbulent energy density $q$ and the integral length scale $\ell$, and are thus independent of viscosity. Given the dimensions of each variable:

$$[q] = L^2T^{-2},\ [\epsilon] = L^2T^{-3},\ [\kappa_q] = L^2T^{-1},\ [\ell] = L,\ [r] = L,\ [t] = T, \tag{14}$$

we can then obtain the turbulent energy diffusion and turbulence dissipation relations by dimensional analysis:

$$\kappa_q = c_0\ell\sqrt{q},\ \epsilon = \epsilon_0\frac{q^{3/2}}{\ell} \tag{15}$$

where $c_0$ and $\epsilon_0$ are dimensionless parameters that moderate the strength of transport and dissipation respectively.

Assuming the large eddies at a given time dominate the behavior of the turbulent blob, we can ignore the spatial dependence in $\ell$, treating it as a global kinetic quantity. This leads to the governing equation, a nonlinear turbulent energy balance equation with coefficients that are explicitly time-dependent:

$$\partial_t q = \frac{2}{3}c_0\ell(t)\,\nabla^2 q^{3/2} - \epsilon_0\frac{q^{3/2}}{\ell(t)} \tag{16}$$

which we refer to as the *Kolmogorov-Barenblatt turbulent energy balance model*. This nonlinear diffusion term rapidly evens out gradients in turbulent kinetic energy. An initially concentrated blob with an asymmetrical shape, with then rapidly assume a spherically symmetric shape as it expands in free space. Consequently, we focus on a spherically symmetric distribution in the asymptotic regime, and reduce Eq. (16) to a radial form. For an arbitrary dimension $d$:

$$\partial_t q = c_0\ell\left[\frac{d-1}{r}\sqrt{q}\,\partial_r q + \frac{(\partial_r q)^2}{2\sqrt{q}} + \sqrt{q}\,\partial_r^2 q\right] - \epsilon_0\frac{q^{3/2}}{\ell}. \tag{17}$$

This radial distribution features a sharp front and a non-diffusive propagating behavior, resulting from the nonlinear transport term $\nabla^2 q^{3/2}$.

### C. Special case assuming instantaneous eddy adaptation

To close this one-equation model, Barenblatt *et al.* made a further assumption that $\ell(t) = \alpha h(t)$, where $\alpha$ is a dimensionless constant to be determined by experiment [9, 10] and $h(t)$ is the location of the front, measured from the center of the turbulent blob. Under this assumption, the governing equation becomes:

$$\partial_t q = \frac{2}{3}c_0\alpha h(t)\,\nabla^2 q^{3/2} - \epsilon_0\frac{q^{3/2}}{\alpha h(t)}. \tag{18}$$

which under the assumption of spherical symmetry becomes:

$$\partial_t q = c_0\alpha h(t)\left[\frac{d-1}{r}\sqrt{q}\,\partial_r q + \frac{(\partial_r q)^2}{2\sqrt{q}} + \sqrt{q}\,\partial_r^2 q\right] - \epsilon_0\frac{q^{3/2}}{\alpha h(t)} \tag{19}$$

Physically, the assumption $\ell(t) = \alpha h(t)$ implies that the largest eddies instantaneously adjust to changes in the size of the turbulence region. This elegant closure inspired extensive physics and

mathematical investigations [11, 12, 15–17]. For the rest of this chapter, we call this assumption the **instantaneous eddy adaptation** assumption.

Later, we will see that this assumption $\ell = \alpha h(t)$ does not hold in our experiment. Nonetheless, the qualitative predictions, such as the sharp front and the non-diffusive propagating behavior, are preserved. Specifically, the similarity analysis [11] and perturbative renormalization group solution [12] offer valuable insights for understanding more complex scenarios that become less analytically tractable once the assumptions are relaxed. We thus first present the theory under this assumption and in the process extend the 1D results from previous works to an arbitrary spatial dimension $d$.

### 1. *Self-similar asymptotics*

We first perform dimensional analysis to derive a dimensionless form of the problem. We define the total turbulent energy $Q(t)$ as:

$$Q(t) \equiv \int d^d\boldsymbol{x}\, q(\boldsymbol{x},t) = \int_0^{h(t)} \Omega_d\, q(r,t)\, r^{d-1} dr, \quad \text{where } \Omega_d = \frac{2\pi^{d/2}}{\Gamma(d/2)} \tag{20}$$

At $t=0$, we adopt the initial conditions $h(0)=a$ and $Q(0)=Q_a$ with dimensions:

$$[h] = [a] = L,\ [Q] = [Q_a] = L^{d+2}T^{-2}. \tag{21}$$

Denoting $\theta \equiv 2/(d+2)$ for convenience, we construct dimensionless quantities

$$\Pi \equiv \frac{qt^{\theta d}}{Q_a^\theta},\ \Pi_1 \equiv \frac{r}{Q_a^{\theta/2}t^\theta},\ \Pi_2 \equiv \frac{a}{Q_a^{\theta/2}t^\theta},\ \Pi_3 \equiv \alpha,\ \Pi_4 \equiv c_0,\ \Pi_5 \equiv \epsilon_0 \tag{22}$$

and rewrite the solution $q(r,t)$ with a dimensionless function $f_q$:

$$\Pi = f_q(\Pi_1,\Pi_2,\Pi_3,\Pi_4,\Pi_5) \quad \Rightarrow \quad q(r,t) = \frac{Q_a^\theta}{t^{\theta d}} f_q\left(\frac{r}{Q_a^{\theta/2}t^\theta}, \frac{a}{Q_a^{\theta/2}t^\theta}, \alpha, c_0, \epsilon_0\right) \tag{23}$$

Similarly for the blob front location $h(t)$, we have:

$$h(t) = Q_a^{\theta/2}t^\theta f_h\left(\frac{a}{Q_a^{\theta/2}t^\theta}, \alpha, c_0, \epsilon_0\right). \tag{24}$$

When $\epsilon_0 = 0$, in the large time asymptotics $Q_a^{\theta/2}t^\theta \gg a$, simply taking the limit $\Pi_2 \to 0$ yields the asymptotic solution. This solution exhibits self-similar dynamics with power-law scaling in time that can be easily read from Eq. (23) and (24), indicating *complete self-similarity.* However, when $\epsilon_0 > 0$, the limits $\lim\limits_{\Pi_2\to 0} f_q$ and $\lim\limits_{\Pi_2\to 0} f_h$ are not well-defined, introducing a singularity that breaks complete self-similarity. Despite this, Eq. (19) retains *incomplete self-similarity*, where the time $t$ appears the scaling functions with nontrivial anomalous dimensions.

From the mathematical point of view, if Eq. (19) has a self-similar asymptotic solution, we can rewrite the solution as $q(r,t) \equiv \phi(t)f(\xi)$, where $\xi = r/h(t)$. Plugging this back into Eq. (19), we obtain

$$-\frac{\dot{h}}{h}\phi \cdot \xi f'(\xi) + \dot{\phi}\cdot f = c_0\alpha\frac{\phi^{3/2}}{h}\cdot\left[\frac{d-1}{\xi}\sqrt{f}f' + \frac{(f')^2}{2\sqrt{f}} + \sqrt{f}f''\right] - \frac{\epsilon_0}{\alpha}\frac{\phi^{3/2}}{h}\cdot f^{3/2}. \tag{25}$$

with power-law scaling functions $h(t) \to A_0 t^{\bar{\theta}}$ and $\phi(t) \to A_0^2 t^{2(\bar{\theta}-1)}$, the explicitly time-dependent coefficients in Eq. (25) cancel out leaving a nonlinear ordinary differential equation (ODE) for $f(\xi)$:

$$-\bar{\theta}\xi f' + 2(\bar{\theta}-1)f = c_0\alpha\left[\frac{d-1}{\xi}\sqrt{f}f' + \frac{(f')^2}{2\sqrt{f}} + \sqrt{f}f''\right] - \frac{\epsilon_0}{\alpha}f^{3/2}. \tag{26}$$

The successful reduction to an ODE indicates that even with dissipation, the long-time asymptotics is self-similar with power-law scaling, though the scaling exponents are not obtainable by dimensional analysis. The value of the scaling exponent $\bar{\theta}$ is obtained by numerically solving a nonlinear eigenvalue problem. Rescaling $f \to \bar{f}/\alpha^2$, we can easily see $\bar{\theta}$ depends only on $\frac{\epsilon_0}{c_0\alpha^2}$ for a given dimension $d$:

$$\begin{gathered}-\bar{\theta}\xi \bar{f}' + 2(\bar{\theta}-1)\bar{f} = \left[\frac{d-1}{\xi}\sqrt{\bar{f}}\bar{f}' + \frac{(\bar{f}')^2}{2\sqrt{\bar{f}}} + \sqrt{\bar{f}}\bar{f}''\right] - \frac{\epsilon_0}{c_0\alpha^2}\bar{f}^{3/2} \\ \bar{f}'(0) = 0, \quad \bar{f}(1) = 0.\end{gathered} \tag{27}$$

We numerically solve for $\bar{\theta}$ using a shooting method, and plot the result for three spatial dimensions in Supplementary Figure 1. A rigorous proof for the existence of the similarity solution and other analytical properties can be found in [15, 17].

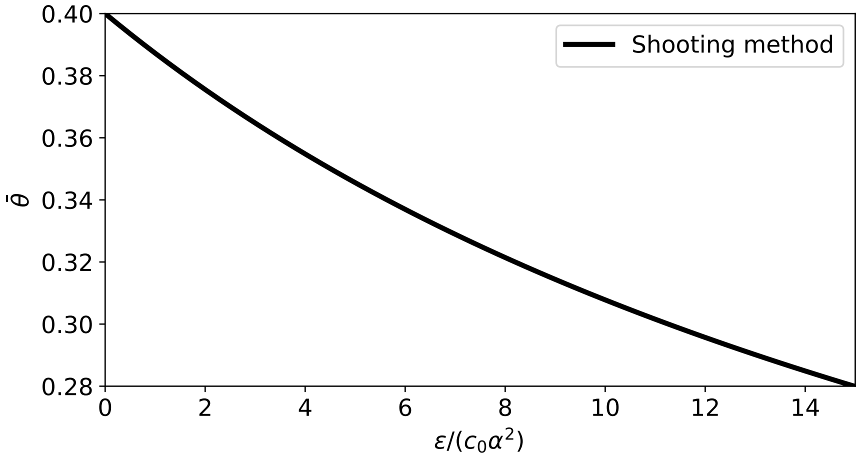


FIG. 1. **Scaling exponent of $h(t)$ in 3D only depends on the ratio $\frac{\epsilon}{c_0\alpha^2}$.** The deviation from 0.4 is an anomalous dimension as a result of the perturbation.

### 2. *A heuristic calculation recovering 1st order perturbative RG*

A perturbative approach to finding the asymptotic solution in 1D was given by Chen *et al.* using the renormalization group (RG) method [12]. Here, we use a "quick and dirty" heuristic calculation to find the asymptotic solution in an dimensions $d$, whose results reproduce the first order RG calculation [18, 19]. In this approach, we consider Eq. (19) as a perturbation theory, and assume an adiabatic process when the dissipation term is small.

In the unperturbed case, where $\epsilon_0 = 0$, the total energy is conserved:

$$\frac{dQ}{dt} = 0, \quad Q(t) = Q_a. \tag{28}$$

The unperturbed/zeroth order equation is

$$\partial_t q_0 = c_0 \alpha h_0(t) \left[ \frac{d-1}{r} \sqrt{q_0}\, \partial_r q_0 + \frac{(\partial_r q_0)^2}{2\sqrt{q_0}} + \sqrt{q_0}\, \partial_r^2 q_0 \right]. \tag{29}$$

We assume a compact initial profile,

$$q_0(r, 0) \propto \left[ 1 - \left( \frac{r}{a} \right)^2 \right]_+^2, \tag{30}$$

where $[g]_+ \equiv g \cdot \Theta(g)$ and $\Theta(x)$ is the Heaviside step function. After normalization, the initial condition can be written as

$$q_0(r, 0) = \frac{Q_a}{\Omega_d I_d a^d} \left[ 1 - \left( \frac{r}{a} \right)^2 \right]_+^2, \tag{31}$$

where $I_d$ is a constant:

$$I_d = \int_0^1 (1 - x^2)^2 x^{d-1} dx = \frac{8}{d(d+2)(d+4)}. \tag{32}$$

The exact zeroth order solution is

$$\begin{aligned} q_0(r, t) &= \frac{Q_a}{h_0^d} \left( \frac{\theta}{4c_0\alpha} \right)^2 \lambda_d^{2/\theta} \left[ 1 - \left( \frac{r}{h_0} \right)^2 \right]_+^2 = \frac{Q_a}{\Omega_d I_d h_0^d} \left[ 1 - \left( \frac{r}{h_0} \right)^2 \right]_+^2 \\ h_0(t) &= \left( \lambda_d^{1/\theta} Q_a^{1/2} t + a^{1/\theta} \right)^\theta, \end{aligned} \tag{33}$$

where $\lambda_d$ is a dimensionless coefficient defined such that $h_0(t) \sim \lambda_d Q_a^{\theta/2} t^\theta$ as $t \to +\infty$:

$$\lambda_d \equiv \left[ 4\theta^{-1} (\Omega_d I_d)^{-1/2} c_0 \alpha \right]^\theta. \tag{34}$$

Now we turn on the dissipation term as a perturbation where $\epsilon_0 > 0$. Assuming an adiabatic loss for the total energy $Q$, the solutions retain the same functional forms, except the constant $Q_a$ is replaced with a time-dependent function $Q(t)$:

$$\begin{aligned} q(r, t) &= \frac{Q(t)}{h^d} \left( \frac{\theta}{4c_0\alpha} \right)^2 \lambda_d^{2/\theta} \left[ 1 - \left( \frac{r}{h(t)} \right)^2 \right]_+^2 \\ h(t) &= \left[ \lambda_d^{1/\theta} Q^{1/2}(t)\, t + a^{1/\theta} \right]^\theta \end{aligned} \tag{35}$$

Integrating both sides of Eq. (19) over space, we obtain a time-evolution equation for $Q$:

$$\begin{aligned} \frac{dQ}{dt} &= -\frac{\epsilon_0}{\alpha h} \int q^{3/2} d^d\mathbf{r} \\ &= -\frac{3\theta}{2(d+6)} \frac{\epsilon_0}{c_0\alpha^2} \frac{\lambda_d^{1/\theta} Q^{3/2}}{\lambda_d^{1/\theta} Q^{1/2} t + a^{1/\theta}} \end{aligned} \tag{36}$$

where we plug in the adiabatic forms (35) for $h(t)$ and $q(t)$. When $t \to +\infty$, Eq. (36) is reduced to the asymptotic form:

$$\frac{dQ}{dt} = -\frac{3\theta}{2(d+6)} \frac{\epsilon_0}{c_0\alpha^2} \frac{Q}{t} \quad \Rightarrow \quad Q \to Q_0 \left( \frac{t}{t_0} \right)^{-\frac{3\theta}{2(d+6)} \frac{\epsilon_0}{c_0\alpha^2}} \sim t^{-\frac{3\theta}{2(d+6)} \frac{\epsilon_0}{c_0\alpha^2}}. \tag{37}$$

Subsequently,

$$
\begin{aligned}
h(t) &\to \lambda_d Q^{\theta/2} t^{\theta} \sim t^{\theta - \frac{3\theta^2}{4(d+6)} \frac{\epsilon_0}{c_0 \alpha^2}} \\
q(r,t) &\to \frac{Q}{h^d} \left(\frac{\theta}{4c_0\alpha}\right)^2 \lambda_d^{2/\theta} \left[1 - \left(\frac{r}{h}\right)^2\right]_+^2 \sim t^{-d\theta - \frac{3\theta^2}{2(d+6)} \frac{\epsilon_0}{c_0\alpha^2}} \left[1 - \left(\frac{r}{h}\right)^2\right]_+^2 .
\end{aligned}
\tag{38}
$$

In 3D, the long-time asymptotics obtained through the heuristic calculation are:

$$
\begin{aligned}
h(t) &\to \lambda_d Q^{1/5} t^{2/5} \sim t^{\frac{2}{5} - \frac{\epsilon_0}{75 c_0 \alpha^2}} \\
q(r,t) &\to \frac{Q}{h^3} \left(\frac{1}{10c_0\alpha}\right)^2 \lambda_d^5 \left[1 - \left(\frac{r}{h}\right)^2\right]_+^2 \sim t^{-\frac{6}{5} - \frac{2\epsilon_0}{75 c_0\alpha^2}} \left[1 - \left(\frac{r}{h}\right)^2\right]_+^2 ,
\end{aligned}
\tag{39}
$$

showing explicitly the anomalous dimension in the scaling decay of the energy.

This calculation is based on an adiabaticity assumption, and is in fact the leading asymptotics in a systematic renormalization group approach to the perturbation theory, with higher order terms representing systematic corrections to the adiabaticity assumption. The leading order calculation suffices for the purposes of interpreting the experimental data.

### 3. *Sharp front and non-diffusive propagation*

One of the most interesting qualitative predictions of the theory is that there is a sharp front separating the laminar and turbulent phases during their coexistence. We spent a significant effort to verify this prediction in our experiment. The earlier experiments of Smith *et al.* [14, 20] did succeed to observe such a sharp front, but in an indirect way and in superfluid helium.

We focus now on the spatial shape of the asymptotic self-similar solution (38). At any time $t$, the shape of the energy profile in the leading-order approximation has a sharp front at $h(t)$ where $q$ drops to zero

$$
q(r,t) \propto \left[1 - \left(\frac{r}{h(t)}\right)^2\right]_+^2 + \mathcal{O}\left(\frac{a}{h(t)}\right), \tag{40}
$$

where the expansion is regular in the long-time asymptotic regime when $h(t) \gg a$ [12]. The sharpness of the front is a direct consequence of eddy diffusivity: a transport term $\nabla^2 q^m$ is associated with a self-similar profile shape $[1-\xi^2]_+^{\frac{1}{m-1}}$ ($m = 3/2$ in our case). When $m > 1$, this front propagates in a non-diffusive manner, meaning the front location $h(t)$ is finite at any time if the initial data is finite in space. In contrast, when $m = 1$ (the case of linear diffusion), the self-similar profile becomes Gaussian, and there is instantaneous propagation of a Gaussian tail to arbitrary distances.

The sharp-front solution is a strong dynamic attractor. When starting from an arbitrary localized initial distribution, the system's behavior over time gravitates towards this self-similar solution. Even when starting with a tail, the system tends to sharpen up the front through evolution, as seen in Supplementary Figure 2.

The formation of a persistent sharp front can have a profound influence on engineering and real-life scenarios such as climate modeling, aerodynamics engineering and flight safety; airplanes may expect to encounter sharp fronts between smooth and "clear air turbulence", and thus there will be no warning signals when the plane crosses such a front, generating a potentially dangerous situation for passengers.

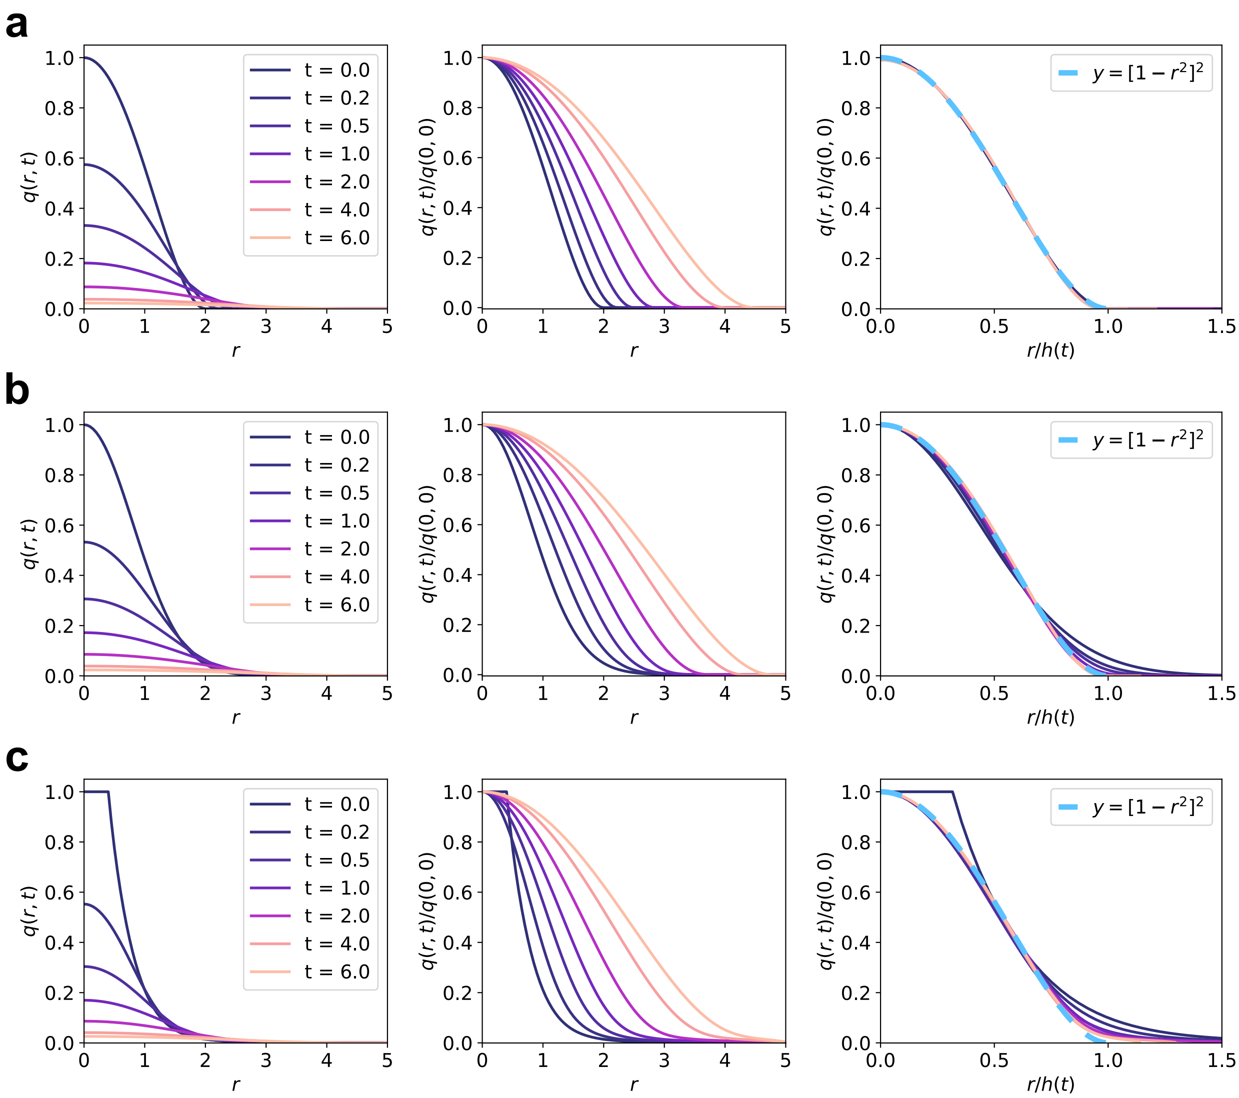


FIG. 2. **Numerical simulations show the formation of a self-similar sharp front profile under the instantaneous eddy assumption with different ICs.** For all three simulation, $\alpha = 0.3$, $c_0 = 1.0$, $\epsilon_0 = 1.0$. The first column captures the propagation process along with spatially inhomogeneous decay. To enhance the front behaviour, $q(r,t)$ at each time step is normalized by the respective central density $q(0,t)$, yielding the rescaled distribution $q(r,t)/q(0,t)$ in the center column. In the last column, further dynamical rescaling of the spatial coordinate $r$ by the front location $h(t)$ yields a scaling collapse to the sharp-front self-similar solution. The three simulations use the following ICs, respectively: (**a**) Compact support IC: $q(r,0) = \left[1 - \left(\frac{r}{2}\right)^2\right]_+^2$ (**b**) Gaussian distribution IC: $q(r,0) = e^{-\frac{r^2}{1.3}}$ (**c**) Power-law tail IC: $q(r,0) = 1$ when $r \leq 0.4$; $q(r,0) = \left(\frac{r+0.3}{0.7}\right)^{-4}$ when $r > 0.4$.

For an arbitrary symmetrical initial distribution, the front position $h$ is extracted by defining a threshold fraction $p$ of the maximum value of $q(r)$ and its corresponding position $h_p$:

$$\left[1 - \left(\frac{h_p}{h}\right)^2\right]^2 \equiv p \quad \Rightarrow \quad h = \frac{h_p}{\sqrt{1 - \sqrt{p}}}. \tag{41}$$

In analyzing the data with a tail, we typically take $p = 0.3$.

### 4. *Energy decay*

In order to compare the experimental data with theoretical predictions, we define the spatial average of the turbulent energy as

$$\langle q\rangle_{\mathbf{x}} \equiv \langle q(\mathbf{x},t)\rangle_{\mathbf{x}} \equiv \frac{\int_V d^d\mathbf{x}\, q(\mathbf{x},t)}{V} \tag{42}$$

where $V$ is the volume of the turbulence blob. For a 3D free-expanding blob, we calculate the asymptotic scaling of its average energy from Eq. (39):

$$\langle q(\mathbf{x},t)\rangle_{\mathbf{x}} \sim t^{-\frac{6}{5}-\frac{2\epsilon_0}{75c_0\alpha^2}} \tag{43}$$

## D. Generalized theory motivated by experimental observations

In the large blob experiment, we observe $\ell \sim t^{0.16}$ with an estimated error in the exponent of 0.04 (see Supplementary Figure 3). The instantaneous eddy adaptation assumption states that $\ell(t) \sim h(t) \sim t^{\bar{\theta}}$, and $\bar{\theta} = 0.16\pm0.04$ corresponds to $\frac{\epsilon_0}{c_0\alpha^2}$ being in the range $40-122$, according to the numerical calculation in Supplementary Figure 1. On the other hand, experimental measurements provide loose bounds for $\alpha = \ell/h$ between $0.3-0.6$, $\epsilon_0 = 0.88\pm0.10$, and $c_0 = 1.20\pm0.11$, resulting in an upper bound for $\frac{\epsilon_0}{c_0\alpha^2}$ around 10. These two independent ways of estimating $\frac{\epsilon_0}{c_0\alpha^2}$ from the same experiment give results differing by an order of magnitude, indicating self-inconsistency. Therefore, the instantaneous eddy adaptation assumption ($\ell = \alpha h$) is *not valid* in our experiment.

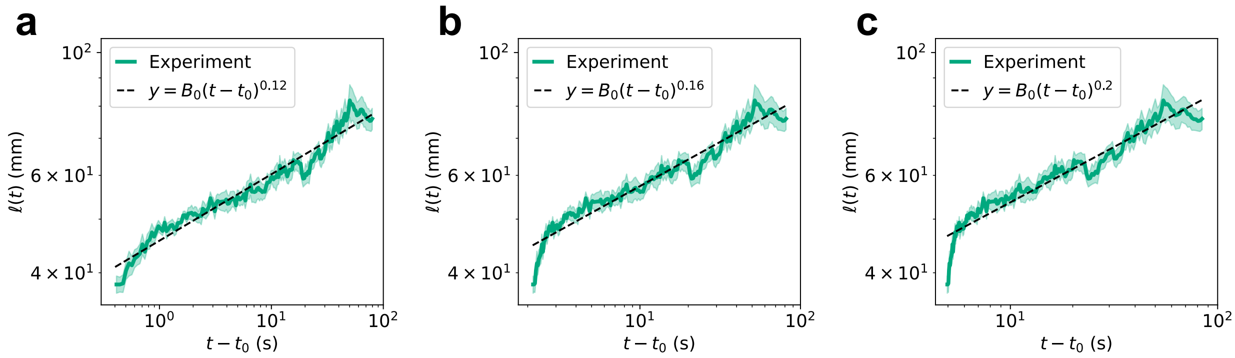


FIG. 3. **Experiment measurement of $\ell$ in the high Re blob experiment shows a power-law growth around $t^{0.16}$.** We qualitatively show the goodness of fitting of $\ell$ with different exponents, where the data of $\ell$ is from the high Re blob experiment from 0.4 s (expansion starts) to 80 s ($\ell$ saturates). (**a**) $\gamma = 0.12$, $B_0 = 45.7$, $t_0 = 0$ s (**b**) $\gamma = 0.16$, $B_0 = 39.7$, $t_0 = -1.75$ s (**c**) $\gamma = 0.2$, $B_0 = 33.8$, $t_0 = -4.55$ s.

There is currently no theory that provides a definitive growth law for the integral length scale. The growth mechanism of $\ell$ involves microscopic details of vortex interactions, which are beyond the scope of a mean-field model. In light of this, we return to the more general equation of motion (Eq. 16) without the instantaneous eddy adaptation assumption:

$$\partial_t q = \frac{2}{3}c_0\,\ell(t)\,\nabla^2 q^{3/2} - \epsilon_0\frac{q^{3/2}}{\ell(t)}$$

and its spherically symmetric form (Eq. 17):

$$\partial_t q = c_0\,\ell(t)\,\left[\frac{d-1}{r}\sqrt{q}\,\partial_r q + \frac{(\partial_r q)^2}{2\sqrt{q}} + \sqrt{q}\,\partial_r^2 q\right] - \epsilon_0 \frac{q^{3/2}}{\ell(t)}.$$

and investigate the asymptotics for a general time-dependent $\ell(t)$ supplied as an exogeneous factor.

### 1. *Approximately self-similar asymptotics*

For an analytical analysis of the asymptotics, we assume a power-law growth $\ell \sim t^\gamma$. Later in numerical simulations of the experiment, we supply the dynamical data of $\ell$ extracted from the experiment. We note that because the size of eddies is bounded by the blob itself, we should always have $\ell(t) \leq 2h(t)$.

Returning to the step above in which we turn on the perturbation $\epsilon_0 > 0$, we note that without the proportionality between $h$ and $\ell$, the dissipation term seems poised to break the self-similar nonlinear propagation in the zeroth order solution. This is indeed the case as we now show by contradiction. Assuming self-similarity exists, the asymptotic solution can be again can rewritten as $q(r,t) \equiv \phi(t) f(\xi)$, where $\xi = r/h(t)$. Plugging back into Eq. (17), we obtain

$$-\frac{\dot{h}}{h}\phi \cdot \xi f'(\xi) + \dot{\phi}\cdot f = c_0 \frac{\ell}{h^2}\phi^{3/2} \cdot \left[\frac{d-1}{\xi}\sqrt{f}f' + \frac{(f')^2}{2\sqrt{f}} + \sqrt{f}f''\right] - \epsilon_0 \frac{1}{\ell}\phi^{3/2} \cdot f^{3/2} \tag{44}$$

Notice that the explicitly time-dependent coefficients on the right hand side are $\frac{\ell}{h^2}\phi^{3/2}$ and $\frac{1}{\ell}\phi^{3/2}$. These cancel if and only if $\ell$ and $h$ are proportional, as in the special case $\ell = \alpha h$; otherwise, this self-similarity by rescaling is broken.

We note however, that from the initial condition to the intermediate asymptotic regime, the full system still exhibits a strong tendency to flow towards an approximately self-similar solution. We demonstrate this approximate self-similarity through a numerical simulation with different initial conditions, as shown in Supplementary Figure 4. By dynamically scaling the profile $q(r,t)$ with the front location $h(t)$ and the central density $q(0,t)$, the curves nearly collapse onto each other after moving beyond the early transient regime.

The behavior of the system can be divided into three temporal stages: the early transient from the initial condition, the intermediate asymptotics near an approximately self-similar solution, and a very long-time regime dependent on the relationship between $h$ and $\ell$. As $t \to \infty$, if $h(t)/\ell(t) \ll 1$, the dissipation term will become less and less relevant [21] and the system gets attracted to a fixed point of self-similar propagation (however this is not physical because the largest eddy cannot be bigger than the blob!). Conversely, if $h(t)/\ell(t) \gg 1$, indicating a delay for the eddies to adjust to the expanding blob boundary, which we will refer to as **delayed eddy adaptation**, the system increasingly deviates from the self-similar form, transitioning to dissipation-dominated dynamics while $h$ continues to grow. A comparison of the self-similarity under different model assumptions is summarized in Table II.

In the large blob experiment, the observed $\ell(t) \sim t^{0.16}$ favors the latter case of delayed eddy adaptation, which possesses the most complicated long-time asymptotics. Fortunately, the effect of this delay on self-similarity is very weak in the intermediate asymptotic regime and becomes prominent only at very long times even for $\epsilon_0 \sim \mathcal{O}(1)$.

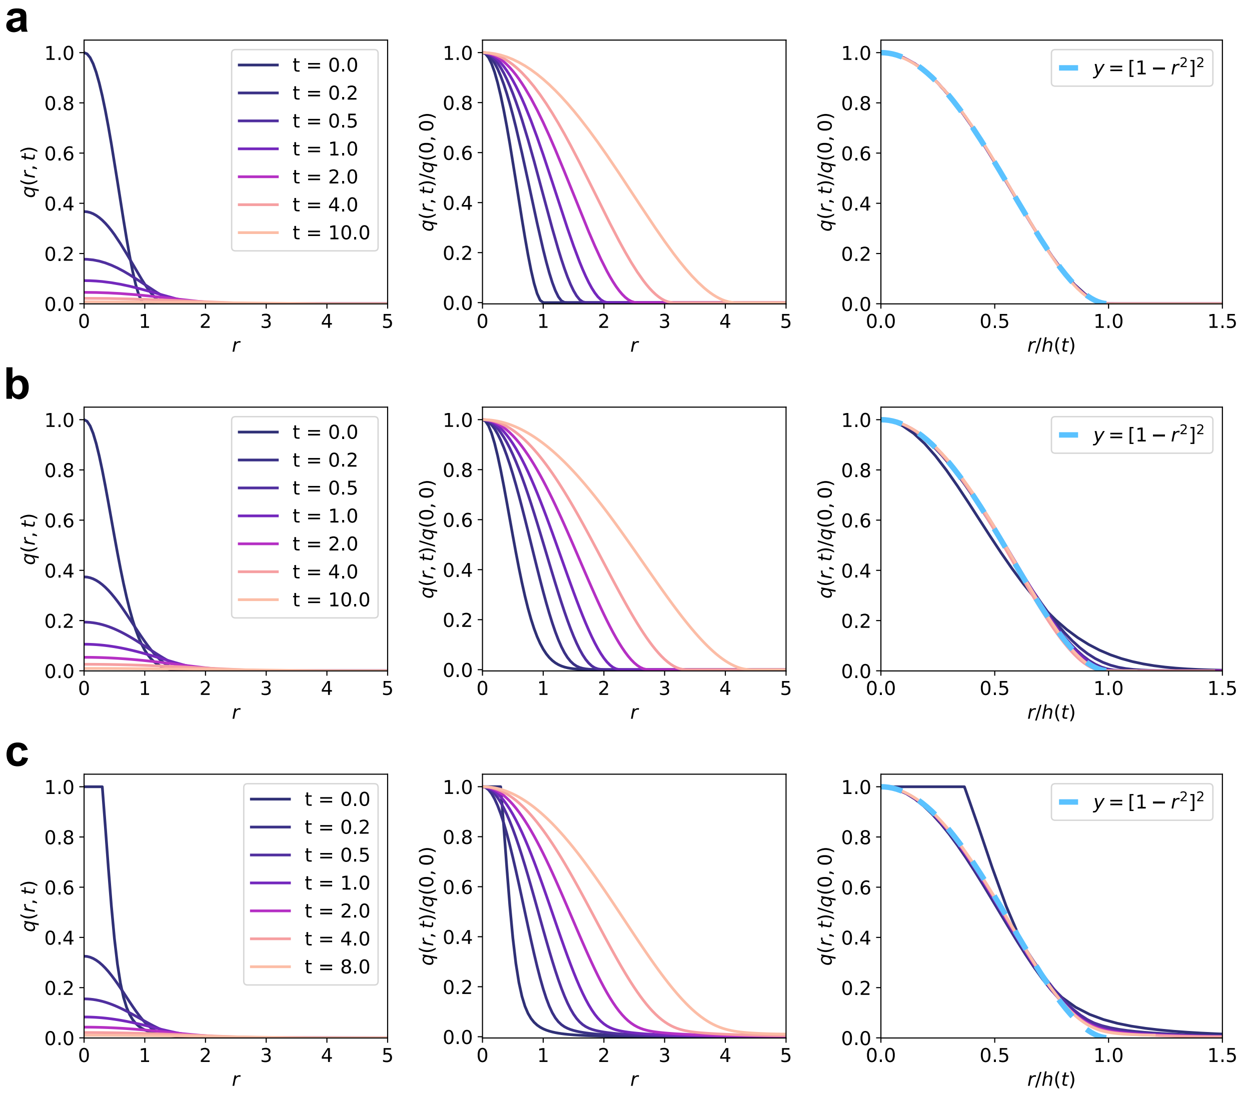


FIG. 4. **Numerical simulations show approximate self-similarity in the delayed eddy assumption case.** For all three simulations, $\gamma = 0.16$, $c_0 = 1.0$, $\epsilon_0 = 0.5$. The first column captures the propagation process along with spatially inhomogeneous decay. To enhance the front behaviour, $q(r,t)$ at each time step is normalized by the respective central density $q(0,t)$, yielding the rescaled distribution $q(r,t)/q(0,t)$ in the center column. In the last column, further dynamical rescaling of the spatial coordinate $r$ by the front location $h(t)$ yields a scaling collapse close to the sharp-front self-similar solution. The three simulations use the following ICs, respectively: (**a**) Compact support IC: $q(r,0) = \left[1 - r^2\right]_+^2$ (**b**) Gaussian distribution IC: $q(r,0) = e^{-\frac{r^2}{0.4}}$ (**c**) Power-law tail IC: $q(r,0) = 1$ when $r \leq 0.3$; $q(r,0) = \left(\frac{r+0.2}{0.5}\right)^{-4}$ when $r > 0.3$.

<table>
<tr><th colspan="2">Model assumptions</th><th>Intermediate asymptotics</th><th>Very long time</th></tr>
<tr><td>$\epsilon_0 = 0$</td><td>Porous medium equation</td><td colspan="2">Complete self-similarity</td></tr>
<tr><td rowspan="3">$\epsilon_0 > 0$</td><td>$\ell = \alpha h$:<br>Instantaneous eddy adaptation</td><td colspan="2">Incomplete self-similarity</td></tr>
<tr><td>$\ell/h \gg 1$</td><td rowspan="2">Approximate self-similarity</td><td>Converge to a self-similar propagation</td></tr>
<tr><td>$\ell/h \ll 1$:<br>Delayed eddy adaptation (large blob experiment)</td><td>Crossover into dissipation dominance</td></tr>
</table>

TABLE II. Self-similarity analysis under different assumptions

### 2. *Zeroth order system*

When $\epsilon_0 = 0$, the zeroth order equation is a porous medium equation with a time dependent coefficient:

$$\begin{aligned} \partial_t q_0 &= \frac{2}{3} c_0 \, \ell(t) \, \nabla^2 q_0^{3/2} \\ &= c_0 \, \ell(t) \, \left[ \frac{d-1}{r} \sqrt{q_0} \, \partial_r q_0 + \frac{(\partial_r q)^2}{2\sqrt{q_0}} + \sqrt{q_0} \, \partial_r^2 q_0 \right] \end{aligned} \tag{45}$$

If $\ell(t)$ is given, the self-similar solution can then be found exactly:

$$q_0(r, \tau) = A_1 \tau^{-\beta d} \left[ 1 - A_2 \frac{r^2}{\tau^{2\beta}} \right]_+^2 , \tag{46}$$

where $\tau \equiv \int^t \ell(t) dt$, $A_1$ and $A_2$ are dimensional constants depending on the initial conditions, and $\beta \equiv 2/(d+4)$ [22]. In the power-law case $\ell \sim t^\gamma$, we have the asymptotic scalings

$$h_0(t) \sim t^{\beta(1+\gamma)} \sim t^{\vartheta} \tag{47}$$

$$q_0(r, t) \sim t^{-d\vartheta} \left[ 1 - \left( \frac{r}{h} \right)^2 \right]_+^2 \tag{48}$$

$$\vartheta \equiv \beta(1+\gamma) \tag{49}$$

where for convenience we have defined a new exponent $\vartheta$ governing the time dependence of the zeroth order solution $h_0(t)$. When $d = 3$,

$$\begin{aligned} h_0(t) &\sim t^{\frac{2}{7}(1+\gamma)} \\ q_0(r, t) &\sim t^{-\frac{6}{7}(1+\gamma)} \left[ 1 - \left( \frac{r}{h} \right)^2 \right]_+^2 \\ \langle q(\mathbf{x}, t) \rangle_{\mathbf{x}} &\sim t^{-\frac{6}{7}(1+\gamma)} \end{aligned} \tag{50}$$

### 3. *Behaviors in the approximately self-similar regime for delayed eddy adaptation*

In this approximately self-similar regime, the sharp front formation and non-diffusive propagation are preserved, as demonstrated in Supplementary Figure 4 with various initial conditions.

Even though the long-time asymptotic behavior of $h(t)$ is not exactly power-law, its functional form empirically closely resembles a power-law scaling $t^{\bar{\vartheta}}$ in the regime of interest, as shown in the blue curves in Supplementary Figure 5. Here, the empirical power-law exponent $\bar{\vartheta}$ is smaller than $\vartheta$ and the magnitude of deviation depends on both $\gamma$ and $\epsilon_0/c_0$, analogous to the negative anomalous dimension in the instantaneous eddy adaptation case. The details of $h(t)$ depend on initial conditions as well the nature of the crossover regime. But for the regime of interest, $\epsilon_0/c_0 \sim \mathcal{O}(1)$ and $\gamma \gtrsim 0.16$, this deviation is small.

The decay of the average energy $\langle q(\mathbf{x}, t)\rangle_{\mathbf{x}}$ deviates away from a power-law growth more significantly, as the dissipation with $q^{3/2}$ in it has a more direct impact on high $q$ values. Crossover behaviours of $\langle q(\mathbf{x}, t)\rangle_{\mathbf{x}}$ are shown in the red curves in Supplementary Figure 5.

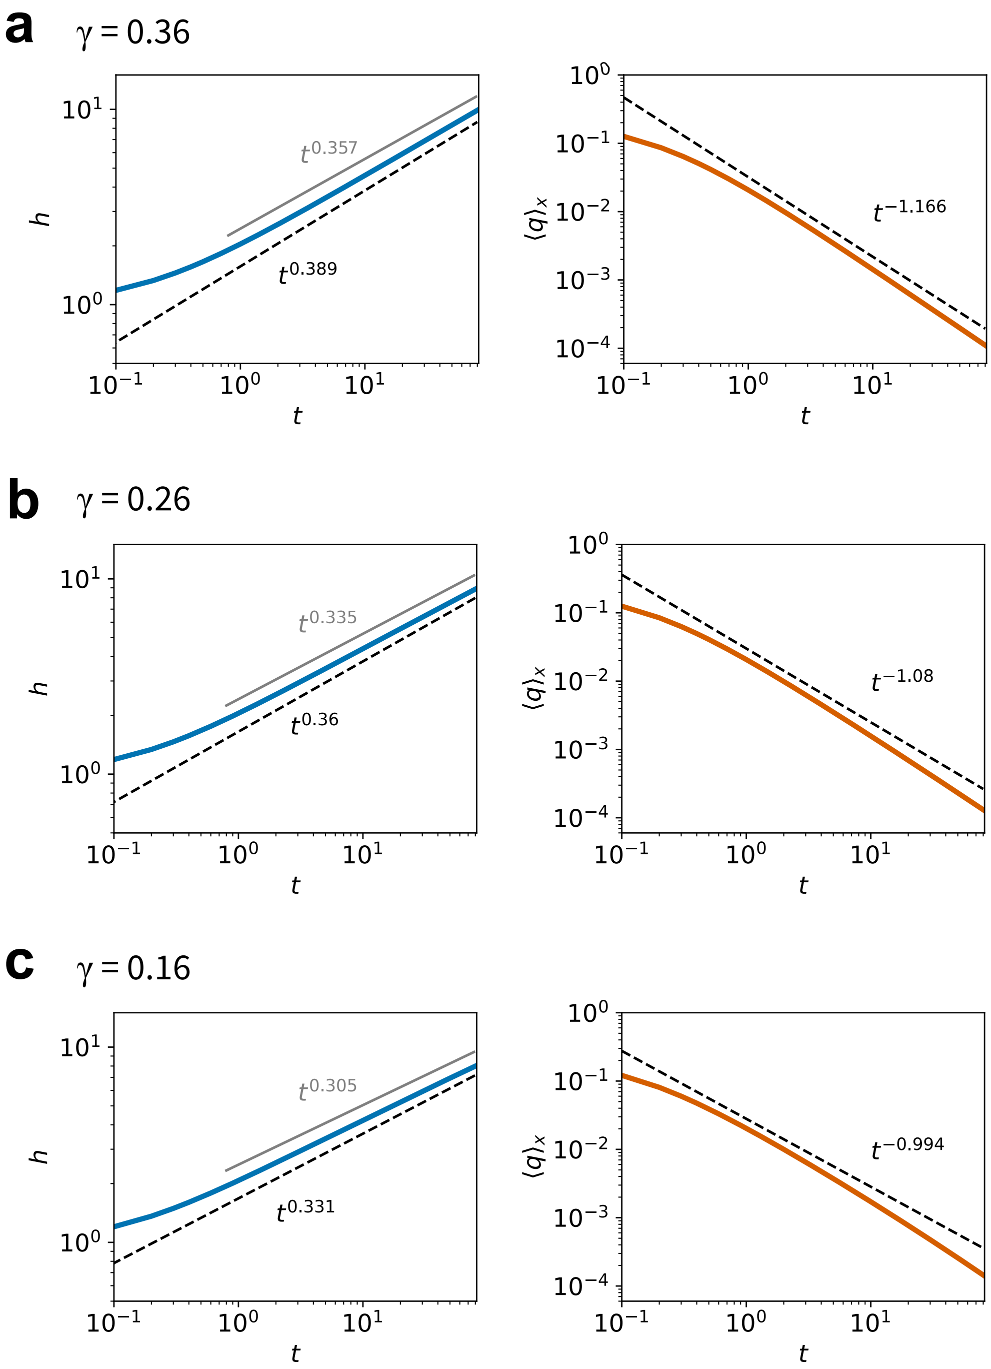


FIG. 5. **Time evolution of the front location $h(t)$ and the average energy $\langle q(\mathbf{x},t)\rangle_{\mathbf{x}}$ for various values of $\gamma$.** For all simulations, $c_0 = 1.0$, $\epsilon_0 = 0.5$, and $\ell = (t + 0.5^{1/\gamma})^{\gamma}$. For each $\gamma$, the blue curve represents $h(t)$ in the simulation, and the gray solid line is an empirical fit of $h(t)$ to a power law at later times. The red curve represents $\langle q(\mathbf{x},t)\rangle_{\mathbf{x}}$. The black dashed lines represent the zeroth-order power law ($h_0 \sim t^{\vartheta}$, $\langle q_0(\mathbf{x},t)\rangle_{\mathbf{x}} \sim t^{-3\vartheta}$ respectively, for this $\gamma$). The values of $\gamma$ are chosen to represent different levels of eddy adaptation delay: (**a**) $\gamma = 0.38$ (**b**) $\gamma = 0.26$ (**c**) $\gamma = 0.16$.

## III. SIMULATIONS: CELL DYNAMICAL SYSTEM METHOD

For more complex initial and boundary conditions, a numerical approach is necessary. We adopt the cell dynamical system (CDS) method which is well suited for creating accurate and efficient spatio-temporal simulations of nonlinear diffusion equations. In this section, we give a additional details of the CDS method discussed in main Figure 5b.

### A. Overview of the CDS method

In our partial differential equation (PDE) model Eq. (16), the evolution of the turbulent energy profile $q(\mathbf{x}, t)$ is governed by two primary mechanisms: an in-place dissipation term $-\epsilon_0 q^{3/2}/\ell$ and a spatial transport term involving the Laplacian $c_0\ell\,\nabla^2(q^{3/2})$. Both terms are highly nonlinear and depend on a dynamically varying global quantity, $\ell(t)$.

To effectively simulate these nonlinear dynamics, we employ a split-step numerical approach, known as the cell dynamical systems (CDS) method [23]. The CDS method has been used to efficiently and accurately simulate other non-equilibrium growth and pattern formation processes ranging from the scaling laws encountered in the kinetics of phase separation [24, 25], the superfluid [26, 27] and superconducting [28] transitions, liquid crystal ordering [29], and the extraordinarily complex spatial patterns that emerge from flow depositional processes at geothermal hot springs [30–32] demonstrating its versatility and effectiveness. Unlike direct PDE discretization, the CDS method treats the space as a lattice of discrete cells. Time evolution is simulated via an injective discrete map that has the same fixed points as the physical problem or its formulation as a differential equation. The map is chosen to be injective and can even be the exact map describing the onsite dynamics a time increment $\Delta t$ into the future, neglecting the diffusion or other spatial derivative terms.

The dynamics on different cells are coupled together by a non-local operator that takes the place of the usual Taylor series representation of the Laplacian (e.g. to order $(\Delta x)^2$). For this, a discrete spatial coupling map is constructed to preserve the isotropy of the Laplacian to a high order [33].

Overall this approach has several benefits over conventional methods. First, it is designed to have the same fixed point structure as the physical problem, and so will be expected to recapitulate the dynamics on large scales. The dynamics on small scales (of order the correlation length) is not universal; however, since there is no guarantee that conventional differential equations based on Landau theory are accurate on small scales, we see no point in trying to make this level of description more accurate. Second, because all maps are injective, the method is topologically stable and large $\Delta t$ and $\Delta x$ can be used, without introducing new instabilities. The philosophy behind this method is based on renormalization group universality, and it has been directly tested in a non-trivial example related to the physics of flow depositional landscapes at geothermal hot springs [30]. Third, the coding of the method is very simple and short, and the programs run very fast, displaying impressive performance relative to alternatives in the problems posed by the propagation of turbulence.

Another split-step algorithm for PDEs involving both spatial derivatives and nonlinear terms is the pseudo-spectral method. While the pseudo-spectral method perfectly preserves the isotropy of the Laplacian and is often faster, it requires periodic boundary conditions, which becomes problematic when simulating a turbulence blob that will eventually fill up the box. In contrast, the CDS method does not have this restriction since it directly operates in real space.

### B. CDS algorithm for the Kolmogorov-Barenblatt turbulent energy balance equation

In our implementation, the energy field $q(\mathbf{x},t)$ is discretized into cells with spacing $\Delta x$. As illustrated in Fig 6a, a single CDS temporal update step for our governing equation Eq. (16) is given by

$$q(\mathbf{x},t+\Delta t) = q(\mathbf{x},t)\left[1+\frac{\epsilon_0 \Delta t}{2\ell(t)}\sqrt{q(\mathbf{x},t)}\right]^{-2} + \Delta t\cdot\frac{2}{3}c_0\,\ell(t)\cdot\hat{L}_{\mathrm{iso}}\left[q^{3/2}(\mathbf{x},t)\right]. \tag{51}$$

The first term is an onsite map derived from a direct integration of the local dissipation dynamics

$$\frac{dq}{dt} = -\epsilon_0\frac{q^{3/2}}{\ell(t)} \Rightarrow \int_{q(\mathbf{x},t)}^{q_1(\mathbf{x},t+\Delta t)}\frac{dq}{q^{3/2}} = -\epsilon_0\frac{\Delta t}{\ell(t)}$$
$$\Rightarrow q_1(\mathbf{x},t+\Delta t) = q(\mathbf{x},t)\left[1+\frac{\epsilon_0\Delta t}{2\ell(t)}\sqrt{q(\mathbf{x},t)}\right]^{-2}. \tag{52}$$

The second term is a coupling map to update the transport term using an isotropic Laplacian. The isotropic Laplacian can be simulated with a linear combination of neighbouring sites, where the selection of weights in this linear combination is carefully determined to preserve the isotropic symmetry of the Laplacian. Denoting $\psi = q^{2/3}(\mathbf{x},t)$, the isotropic Laplacian is given by:

$$\hat{L}_{\mathrm{iso}}\left[q^{3/2}(\mathbf{x},t)\right] = \sum C_1\cdot\psi_{i1} + \sum C_2\cdot\psi_{i2} + \sum C_3\cdot\psi_{i3} - C_0\cdot\psi_i, \tag{53}$$

where $C_1 = 16/36$, $C_2 = 4/36$, $C_3 = 1/36$ and $C_0 = 152/36$ are used in 3D simulations. This map is referred to as the D3Q27 lattice model in [34] and achieves spectral isotropy on the order of $\mathcal{O}(k^4)$.

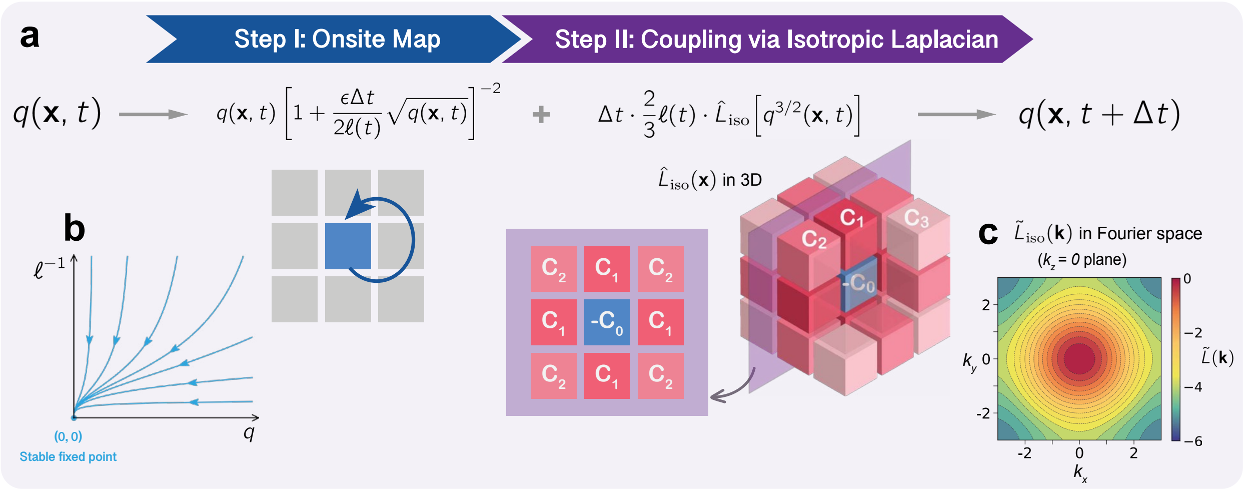


FIG. 6. **Schematic illustration of one time update of the split-step CDS method for simulating the nonlinear turbulence model.** (**a**) The onsite map is obtained from an exact integration of the dissipation term. The coupling step utilizes a 3D isotropic Laplacian to directly simulate the transport behavior through inter-cell interactions. (**b**) The onsite map converges to a stable fixed point. (**c**) Spectral isotropy of the D3Q27 lattice model, the isotropic Laplacian used in our simulations [34].

We note here some additional benefits of the CDS approach over traditional numerical approaches. Notably, the onsite map's fixed point is independent of the discretization process. For the

coupling map, comparing to finite difference methods, the isotropic Laplacian preserves rotational symmetry, resulting in an accurate and stable computational scheme. This effectively mitigates the oscillation artifacts at a moving sharp front typically seen with finite difference methods [35], especially in higher dimension. Moreover, the implementation of the CDS method is both simpler and more straightforward than that of advanced approaches, such as adaptive mesh refinement [36] and finite volume [35]. It exhibits a remarkable insensitivity to discretization resolution, enhancing space efficiency. The usage a small stencil facilitates high parallelizability, significantly accelerating computation especially for high-dimensional simulations.

### C. Benchmark of the method

We test the effectiveness of the CDS method by using it to simulate the Kolmogorov-Barenblatt turbulent energy balance equation in the case of instantaneous eddy adaptation ($\ell = \alpha h$), Eq. (18), for which we have analytical solutions to compare with. We do so in a 3D infinite system with a compact support for the initial condition $q(r,0) = q_0 \left[1 - \left(\frac{r}{h_0}\right)^2\right]_+^2$. We find that when $\epsilon_0 = 0$, the simulation results agree exactly with the analytical solution. With non-zero dissipation $\epsilon_0 \in [0, 0.2]$, the evolution of the profile agrees with the 1st order perturbative RG solution reasonably well; As shown in Supplementary Figure 7, by extracting the time exponents of $h(t)$, we find the exponent $\bar{\theta}$ is in agreement with the exact numerical calculation.

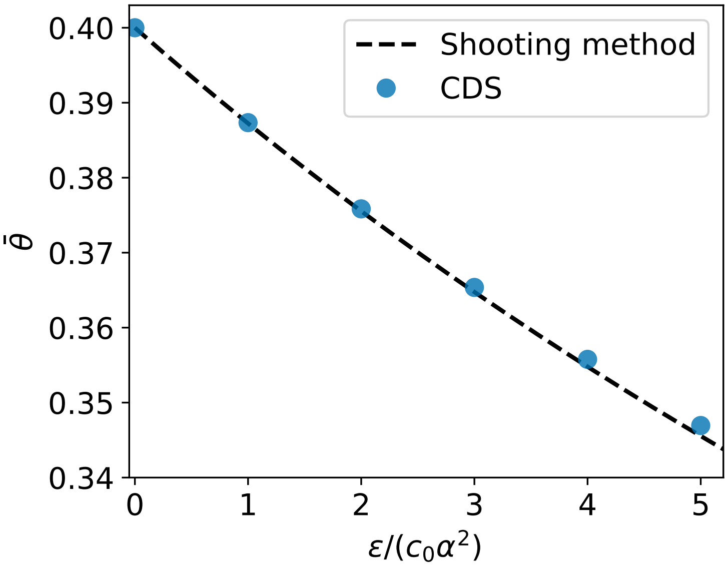


FIG. 7. **CDS simulation accurately predicts the growth exponent of $h(t)$, compared with the exact numerical method.** Exact numerical results are obtained using a shooting method from the eigenvalue problem (as solved in Supplementary Figure 1). In the CDS simulation, for each value of $\frac{\epsilon}{c_0\alpha^2}$, we run a 3D spatiotemporal simulation, extract the front location $h(t)$ and then determine $\bar{\theta}$ using the virtual origin method.

We conclude that the CDS method is well suited to solving the nonlinear Kolmogorov-Barenblatt turbulent energy balance equation in free space.

### D. Boundary condition

For a finite system such as our experimental blob, a boundary condition is required. We adopt a partially absorbing boundary condition. In particular, we define a coefficient $p_{\text{abs}}$, such that when executing the coupling map of the CDS simulation, the next neighbour out of the boundary is padded with $(1 - p_{\text{abs}})\psi_0$, i.e., $p_{\text{abs}}$ represents the percentage of flux lost/absorbed when reflected from the wall.

### E. Summary of CDS Simulations and corresponding parameters used

This section summarizes the cell dynamical system (CDS) simulations performed in this study. Initial conditions were extracted from instantaneous 2D turbulent velocity fields measured in the experiments. A short waiting period was typically introduced prior to simulation onset to eliminate residual bias from the flow-driving mechanism. Partially absorbing boundary conditions were used throughout (see §III D).

TABLE III. **Transport and dissipation parameters used in CDS simulations**

| Corresponding Experimental Dataset[1] | Description | Initial Condition | Integral lengthscale, $\ell(t)$ | $c_0$ | $\epsilon_0$ |
|---|---|---|---|---|---|
| Dataset 1 | Vortex ring collision (*small* turbulent blob) | $q(\mathbf{x}, t = 0.85\,\text{s})$ from experiments[2] | $0.1L_{\text{box}}(t - t_0)^{0.38}$ for $t - t_0 < 25\,\text{s}$ | 1.2[3] | 0.88[4] |
| Dataset 2 | Vortex ring collision (*large* turbulent blob, fast transport) | $q(\mathbf{x}, t = 0.4\,\text{s})$ from experiments[1] | $0.1L_{\text{box}}(t - t_0)^{0.16}$ for $t - t_0 < 80\,\text{s}$, $0.25L_{\text{box}}$ otherwise | 1.2[2,4] | 0.88[4] |
| Dataset 2 | Vortex ring collision (*large* turbulent blob, slow transport) | $q(\mathbf{x}, t = 0.5\,\text{s})$ from experiments[1] | $0.1L_{\text{box}}(t - t_0)^{0.16}$ for $t - t_0 < 80\,\text{s}$, $0.25L_{\text{box}}$ otherwise | 0.001[3,5] | 0.88[4] |
| Dataset 5 | Double oscillating grid | $q(\mathbf{x}, t = 0.003\,\text{s})$ from experiments[2] | $0.25L_{\text{box}}$ | 1.07 | 1.2[4] |

[1] See Table VI for experimental details about corresponding datasets.
[2] The experiment provides only a 2D turbulent energy field. The simulation box was constructed by rotating the 2D velocity field about the central axis and padding the remainder with nearest-neighbor values. Note that the initial condition is a single time snapshot, not an ensemble-averaged field.
[3] See main Figure 5c. Extracted from the propagating dynamics.
[4] See main Figure 4b. Extracted from the energy decay during late times.
[5] See main Figure 2c for energy decay curves compared with experimental data.

## IV. EXPERIMENTS

### A. Experimental methods

In this section we describe the experimental flow chamber geometry, the flow actuation and imaging methods.

#### 1. Flow chamber

All experiments are performed in a 3D-printed, cubic chamber suspended in a water-filled tank. The corners of the chamber are truncated and replaced with triangular facets designed to accommodate interchangeable custom orifices that are magnetically attached (see Supplementary Figure 8).

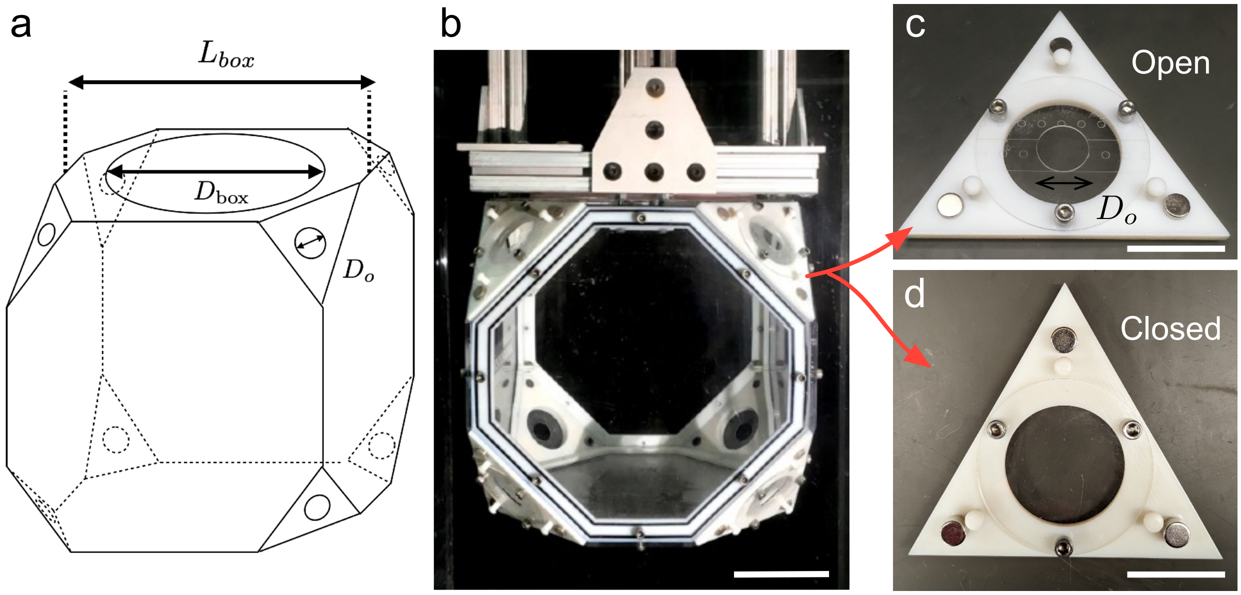


FIG. 8. **Geometry of the flow chamber.** (**a**) Schematic of the experimental chamber is shown. (**b**) The experimental chamber consists of a 3D-printed frame and six acrylic faces. The scale bar represents 100 mm. (**c**) A 3D-printed "holster" is magnetically attached to each truncated surface of the chamber. A circular, acrylic plate with an orifice may be attached to enable generation of a vortex ring at each site. (**d**) Alternatively, a circular plate is attached to confine the flow in the chamber. The scale bars in (c) and (d) represent 50 mm.

#### 2. Actuation

We generate turbulence in the same flow chamber by three methods

1. Oscillating a single grid inside the chamber (with the orifices closed)

2. Oscillating a double-grid inside the chamber (with the orifices closed)

3. Actuating a large circular section at the top of the chamber (with the orifices open) to generate incoming vortices.

The physical dimensions of the grids and the chamber are listed in Table IV. Results from the double-grid and vortex actuation are discussed in the main text. Data generated using a Single-grid is reported only in the SI.

*The single acrylic grid* is actuated with a sinusoidal drive (Supplementary Figure 9a). This method is known to create a turbulent front in a pipe for superfluid [14]. The grid is prepared by laser-cutting an acrylic plate with thickness of 1/4" =6.35mm into a circular shape with a diameter of $D_{\mathrm{grid}} = 200$ mm (Supplementary Figure 9d). The mesh size $M$ is 12.5 mm (Supplementary Figure 9e). Because we drive the grid near the upper surface of the chamber, it generates a downward mean flow.

*The double acrylic grid.* To create a turbulent region, with as small a mean flow as possible, we added a second grid and oscillate the two grids connected together by aluminum rods (Supplementary Figure 9b). These two grids are separated by $\ell_{\mathrm{sep}}$=210 mm (Supplementary Figure 9f).

*Vortex ring actuation.* Our third method of actuation consists of repeatedly colliding vortex rings in the chamber (Supplementary Figure 9c). When vortex rings are fired at a sufficiently high rate, this method creates a steady, isolated blob of turbulence, sitting in a quiescent environment [2]. Vortex rings are created by lifting an acrylic piston ($D_p = 12.7$ mm, Supplementary Figure 9h) through the upper surface of the chamber, which withdraws fluid through circular apertures, allowing boundary layers to roll up.

TABLE IV. **Dimensions for single oscillating grid and double oscillating grid experiments**

| Component | Length (mm) |
|---|---|
| Width of the experimental chamber, $L_{\mathrm{box}}$ | 351.0 |
| Diameter of the circular grid, $D_{\mathrm{grid}}$ | 200.0 |
| Mesh size, $M$ | 12.5 |
| Thickness of the grid | 8.2 |
| Vertical separation between the grids, $l_{\mathrm{sep}}$ | 210.0 |
| Solidity | 34% |

The orifice and piston diameters used to generate the large and small turbulent blobs reported in the main text are summarized in Table V.

TABLE V. **Dimensions for generating large vs. small turbulent blobs**

| Component | Large blob settings ($R_{\mathrm{blob}} \approx 60$ mm) Length (mm) | Small blob settings ($R_{\mathrm{blob}} \approx 40$ mm) Length (mm) |
|---|---|---|
| Width of the experimental chamber, $L_{\mathrm{box}}$ | 351.0 | 351.0 |
| Piston diameter, $D_p$ | 160.0 | 56.7 |
| Orifice diameter, $D_o$ | 25.6 | 12.8 |

In all cases, we actuate using an electric linear actuator (STA2510S, Copley Controls Corp) to drive the system. Both the actuation span and velocity are programmable and managed via a data acquisition board (PCI-6251, National Instruments). To monitor the piston's motion with sub-millimeter precision, we employ a transmissive optical encoder (EM2, US Digital). Supplementary Figures 9g-h illustrate the average profiles of the sinusoidal and sawtooth drives used in our experiments.

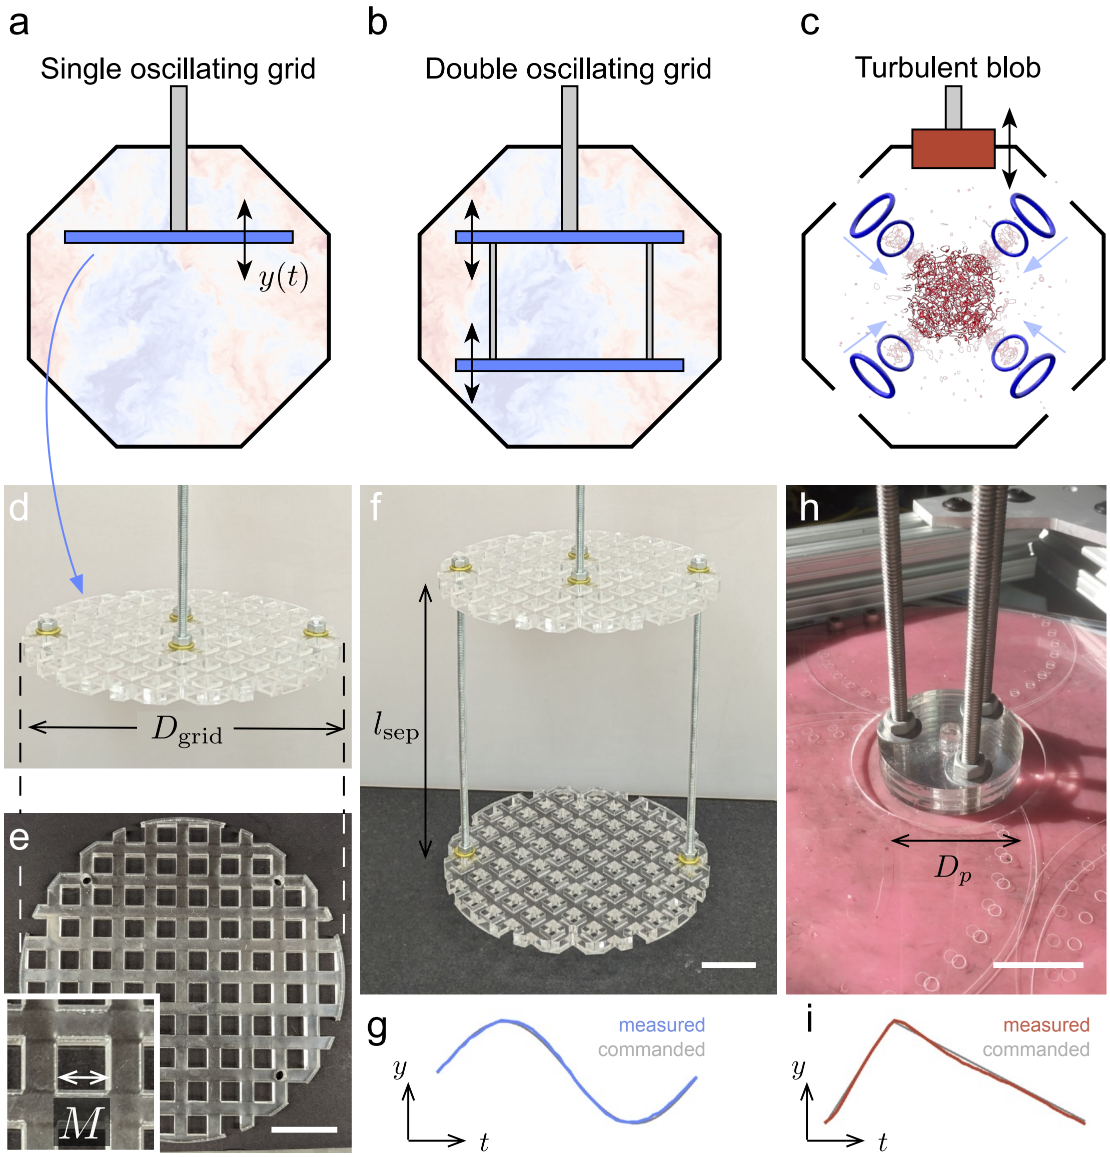


FIG. 9. **Three methods of actuation to generate turbulence in a flow chamber:** (**a**) A single oscillating grid (**b**) Double oscillating grids (**c**) Repeated collision of vortex rings. (**d-e**) An circular, acrylic grid with square meshes is used to set up flows in the experiments. (**f**) Two identical grids are bolted together with a separation distance $l_{\text{sep}}$ of 210 mm for the experiments involving the double oscillating grids. (**g**) Both single and double grids are driven by a sinusoidal signal in a closed chamber. The blue curve show the measured amplitude. (**h**) To create vortex rings, an acrylic, cylindrical piston used to withdraw fluid into the chamber through circular orifices. (**i**) A sawtooth profile is used to generate vortex rings repeatedly. The scale bars in (e), (f), and (h) represent 40 mm.

### *3. PIV experiments*

To perform Particle Imaging Velocimetry, we first suspend fluorescent particles (fluorescent red, $d = 100\ \mu m, \rho = 0.995$ g/cm$^3$, Cospheric LLC) in water by gradually adding them while the solution is being stirred. The solution is then injected into the chamber using a syringe. We create a laser sheet with an Nd:YLF pulsed laser ($\lambda = 526.5$ nm, Photonics Industries International, Inc). and a cylindrical lens to fluoresce the particles at the peak emission wavelength at 630 nm. We

image using a high-speed camera (VEO640L or VEO4k 990L, Vision Research) at the adequate frame rate, ranging from 250 to 2000 Hz. To suppress the background originated from the laser sheet, we use a high-pass filter to eliminate the light below $\lambda = 540$ nm. The frame rate and the interrogation window size are chosen so that a "quarter rule"[37] is always satisfied for the fastest motion in the flow.

#### 4. *Logarithmic triggering to capture decay*

Measuring the decay of turbulent energy is challenging because the temporal and spatial scales in the turbulent flow drastically change during the process. To overcome this challenge, we take images with a decreasing frame rate while turbulence decays. We design the timing between image acquisitions by guessing the decay rate of the turbulent intensity and choosing timing such that a root-mean-square displacement of tracer particles would remain constant. We base the guess based on the common assumption that turbulent kinetic energy decays as a power law, meaning

$$q = c(t - t_0)^n$$

for $t > t_0$ with an energy decay exponent $n \leq -1$ and virtual origin $t_0$ [38, 39]. If the energy decays with a single power law, the interval $\Delta(t)$, required to preserve a root-mean-square displacement $d$, is obtained by solving

$$\int_t^{t+\Delta(t)} U_{\rm rms}(t')dt' = d. \tag{54}$$

This leads to

$$\Delta(t) = \begin{cases} (t-t_0)\exp\left(\frac{d}{\sqrt{2c}} - 1\right) & (m = 0 \Leftrightarrow n = -2), \\ (t-t_0)\left[\left(1 + \frac{md}{\sqrt{2c}}\frac{1}{(t-t_0)^m}\right)^{\frac{1}{m}} - 1\right] & (m \neq 0 \Leftrightarrow n \neq -2), \end{cases} \tag{55}$$

where $m = n/2 + 1$. It is insightful to note that that the long-time asymptotics of Eq. 55 is given by

$$\Delta(t) \sim (t - t_0)^{(1-m)} = (t - t_0)^{\frac{n}{2}} \tag{56}$$

for any decay exponent $n$, provided $t - t_0 < (-md/\sqrt{2c})^{1/m}$. This bound on $t - t_0$ originates from the fact that Eq. 54 would not be satisfied if the velocity decayed too fast. Even in case of the accelerating behavior, Eq. 55 remains valid as long as $t - t_0 > 0$.

Starting with an initial time $t_1$, Eq. 55 generates a sequence of time points maintaining the motion's displacement: $\{t_k \mid t_k = t_1 + \sum_{j=1}^{k-1}\Delta(t_j),\ \forall\ k \in \mathbb{N},\ k > 1\}$, including $t_1$ itself. An emphasis is placed on the case $n = -2$, where the time interval $\Delta(t)$ is proportional to $(t - t_0)$. It can be readily shown that $\log t_k - \log t_{k-1} = \log(1 + c) = \text{const.}$ for any $k > 1$. This property makes the logarithmic time scale $\tau \equiv \log t$ a natural choice for visualizing dynamics. Given that the turbulence under study partially or fully decays with the $n = -2$ power law, we present a *log movie* as an effective means to visualize the flow.

This methodology of the log movie can be generalized for any phenomenon that evolves over time following a power law, ranging from gravity waves to critical phenomena. For each dynamics, there exists a way to scale time in which the time scale of the apparent dynamics remains the same. Consider a ball in free fall under gravity. Thanks to our internal clocks, an observer on the ground would perceive this as increasing speed. However, if our internal clocks were broken, we

might perceive the motion as ballistic. Mathematically, we seek a function $\tau(t)$ that satisfies the condition $\tau(t_{k+1}) - \tau(t_k)$= const. By Taylor-expanding $\tau(t_{k+1}) = \tau(t_k + \Delta(t_k))$, we find

$$\tau(t) \sim \begin{cases} \log(t - t_0) & (m = 0 \Leftrightarrow n = -2), \\ (t - t_0)^m & (m \neq 0 \Leftrightarrow n \neq -2). \end{cases} \tag{57}$$

In this scaled time $\tau$, the power-law dynamics becomes ballistic. Moreover, one can apply this methodology to the spatial scale, ensuring the apparent dynamics remains unchanged throughout self-similar evolution.

Supplementary Figure 10a-b illustrate the progression of the frame rate adopted to capture the decay of turbulence. The acquisition scheme lasts for 1050 seconds (= 17.5 minutes), and consists of three parts. First, the camera is triggered at a constant frame rate for approximately one second. The exact duration of this part depends on the choice of virtual origin $t_0$, and the initial root-mean-square velocity. Subsequent triggering timings are determined by using Eq. 55 for $n = -2$. Once the frame rate reaches the minimal value supported by the timing box, $f_{\min}$, indicated by a dashed line in Supplementary Figure 10a, we fix the frame rate at $f_{\min}$.

We have tested the triggering schemes that correspond to different values of the decay exponent $n$, ranging from -1 to -3, and obtained a velocity field with a similar quality after performing PIV. Deviation of the measured power law from the adopted $n$ results in the particle motion to be either accelerated or decelerated. In such a case, the particle displacement per frame may exceed the dynamic range of the PIV capability, leading to the inaccurate extraction of a velocity field. For all flow measurements we report, we ensured that average particle displacement per frame falls in the dynamic range, specifically, between the noise floor (< 1px) and the half of the interrogation window size, $W/2 = 16$px.

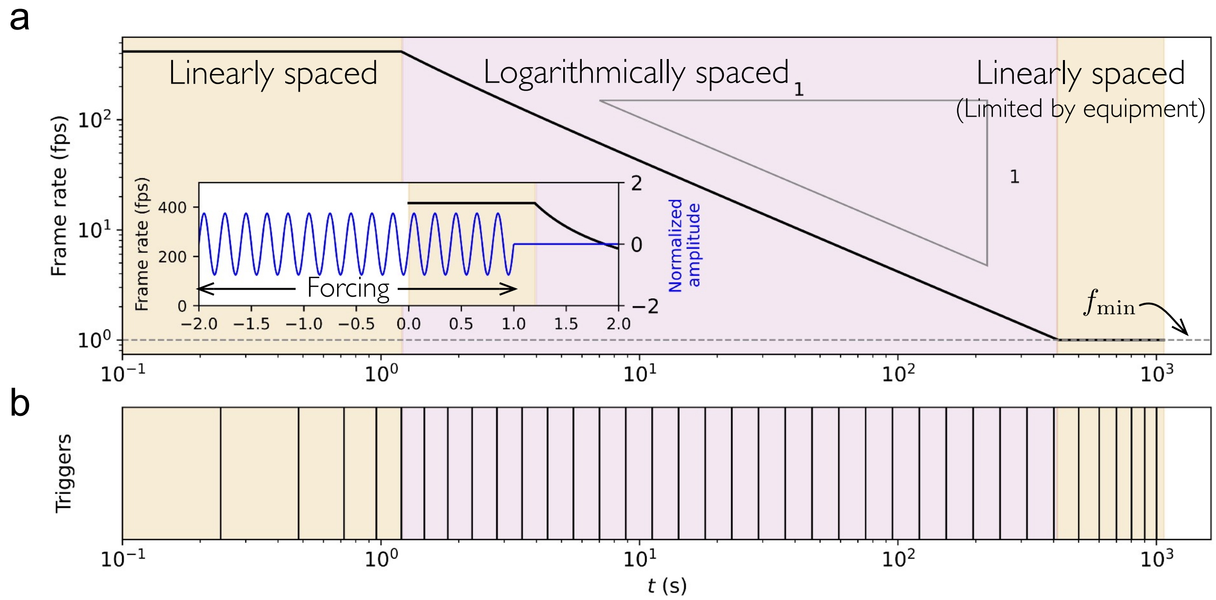


FIG. 10. **A customized triggering scheme applied to capture the decelerating dynamics** (**a**)The frame rate of the high-speed camera is progressively decreased as the dynamics slows down. (**b**) The lines indicate the time points at which the camera is triggered. For clarity, only 1% of the triggers are shown. Within each interval, the high-speed camera is triggered 100 times.

## B. Summary of experimental runs

Three types of experiments were performed for this study. The first captured the full decay over 17 minutes using the logarithmic triggering scheme described in §IV A 4. The second recorded the first 10–25 seconds of decay at a constant frame rate (500–2000 fps), focusing on the early expansion phase. The third captured the expansion process of turbulent blobs in 3D using particle tracking velocimetry (PTV) [40]. Table VI summarizes the experimental conditions.

TABLE VI. **Summary of experimental parameters**.

| Label | Method | Forcing protocol | $\mathrm{Re}_L$ | $\mathrm{Re}_\lambda$ | $n$[a] | Recording method |
|---|---|---|---|---|---|---|
| Dataset 1 | Vortex ring collision (A *small* turbulent blob) | Sawtooth, 20% duty cycle $(A, V_p, f)$=(11.2 mm, 200 mm/s, 5 Hz) | 3,600 | 60 | 10 | 2D PIV, Constant sequence |
| Dataset 2 | Vortex ring collision (A *large* turbulent blob) | Sawtooth, 20% duty cycle $(A, V_p, f)$=(10.5 mm, 200 mms/s, 5 Hz) | 15,400 | 203 | 21 | 2D PIV, Logarithmic sequence |
| Dataset 3 | Vortex ring collision (A *large* turbulent blob) | Sawtooth, 20% duty cycle $(A, V_p, f)$=(11.2 mm, 200 mm/s, 5 Hz) | 15,400 | 203 | 1 | 3D PTV, Constant frame rate |
| Dataset 4 | Vortex ring collision (A *small* turbulent blob) | Sawtooth, 20% duty cycle $(A, V_p, f)$=(11.2 mm, 200 mm/s, 5 Hz) | 3,600 | 60 | 1 | 3D PTV, Constant frame rate |
| Dataset 5 | Double oscillating grid | $y(t) = A\sin(2\pi f t)$ $(A, f)$=(18 mm, 5 Hz) | 10,100 | 185 | 10 | 2D PIV, Logarithmic sequence |
| Dataset 6 | Single oscillating grid | $y(t) = A\sin(2\pi f t)$ $(A, f)$=(18 mm, 5 Hz) | 5,300 | 95 | 10 | 2D PIV, Logarithmic sequence |

[a] The number of recordings collected for ensemble averaging and Reynolds decomposition of the velocity field

### C. Data analysis

#### *1. Analysis pipeline*

In this study, we report quantities averaged over space, time, and ensemble. The order in which these averages are taken can be important in some cases. Supplementary Figure 11 outlines the computational pipeline and specifies how each reported quantity, referenced in figures and supplementary movies, was computed. All analyses begin with velocity fields obtained from 2D PIV or 3D PTV, which often contain noise and missing vectors. We remove extreme outliers by thresholding, apply a $3 \times 3$ or $5 \times 5$ median filter to suppress spurious values, and pad missing vectors using local averages. The resulting filtered field is used to compute quantities such as kinetic energy and vorticity. Velocity gradients, including vorticity, are computed by smoothing with a Savitzky-Golay filter, followed by taking a central difference. This pre-processing is applied because even median-filtered PIV data contains substantial noise for estimating the velocity gradients.

We perform a Reynolds decomposition to separate the velocity field into a mean flow and turbulent fluctuations (see §IV C 2). The mean flow yields mean flow energy and vorticity, distinct from the raw energy and raw vorticity fields. Fluctuating components, which differ across realizations, are used to compute quantities such as turbulent kinetic energy, turbulent vorticity, the 3D energy spectrum, the second-order structure function, and the integral length scale.

To compute blob expansion rates compare with the predictions of the non-linear diffusion model, we apply ensemble averaging and the analyze the ensemble averaged spatial evolution of the fluctuating turbulent energy. For turbulent energy decay, we first compute spatially averaged turbulent energy in each realization and then take the ensemble average. We note that the order of spatial and ensemble averaging has little effect in our data. For composite quantities such as the dissipation rate, $\epsilon \sim q^{3/2}/\ell$, the choice of averaging order is not obvious. While $\langle \langle q^{3/2} \rangle_{\mathbf{x}}(t)/\ell(t) \rangle_{\mathrm{n}}$ may appear to be proportional to $\langle \epsilon \rangle_{\mathrm{n}}(t)$, the $\ell$ values are derived from instantaneous 2D snapshots of the velocity field and may not reflect the full turbulent structure. In practice, using $\langle \ell \rangle_{\mathrm{n}}(t)$ instead yields more statistically meaningful estimates, and the resulting $\langle q^{3/2} \rangle_{\mathbf{x},\mathrm{n}}(t)/\langle \ell \rangle_{\mathrm{n}}(t)$ is more robust and interpretable.

*2. Velocity fluctuations and convergence of mean flow*

For steady flows, the temporally averaged flow is conventionally adopted as the mean flow. However, this approach is unsuitable for unsteady flows, where the mean flow evolves spatially and temporally. In this study, we define the mean flow as the flow averaged over multiple replicas. The fluctuating velocity field, $u_i(x_j, t)$, is then computed as

$$u_i(x_j, t) = U_i(x_j, t) - \langle U_i \rangle_{\mathrm{n}}(x_j, t). \tag{58}$$

With a sufficiently large number of samples, the ensemble-averaged flow eliminates fluctuations across different runs, yielding a converged mean flow. Supplementary Figure 12a-c show the mean flow energy, $\overline{\mathcal{E}} = (1/2)\langle \mathbf{U} \rangle \cdot \langle \mathbf{U} \rangle$ for all types of flows presented in this paper. As visible by inspection of Figure 12a-c, an average over $n = 6$ realizations looks visually similar to an average over $n = 10$ realization, suggesting the mean flow measurement has converged. Further quantitative evidence is provided by the energy spectrum of the mean flow, shown in Supplementary Figure 12d-f.

SI Movies 7, 13, and 14 illustrate the time evolution of the mean flow for different datasets: the large turbulent blob (Dataset 2), the double oscillating grid (Dataset 5), and the single oscillating grid (Dataset 6).

### 3. *Virtual Origin Determination*

Our measurements indicate that the decay of the kinetic energy of the fluctuating component of the flow follows a power law after an initial transient period, described as $\langle q \rangle_{\mathbf{x},\mathrm{n}}(t) = A(t - t_0)^n$. The determination of the virtual origin $t_0$ strongly affects the estimation of the exponent $n$. To eliminate subjective bias, we employ the following procedure, summarized below. For convenience we define the coefficient of determination $r \equiv 1 - \frac{\mathrm{RSS}}{\mathrm{TSS}}$ where RSS is the residual sum of squares, $\mathrm{RSS} = \sum(y - y_{\mathrm{pred}})^2$, and TSS is the total sum of squares, $\mathrm{TSS} = \sum(y - y_{\mathrm{mean}})^2$. A poor fit may result in a negative value of $r$.

Consider a quantity $x$ that decays according to a power law with an exponent $n$:

1. Define the region of interest for fitting, $[t_a, t_b]$.
2. Split the region into two subregions with equal numbers of data points. Using the logarithmic triggering scheme described in §IV A 4, these subregions are $[t_a, t_m]$ and $[t_m, t_b]$, where $t_m = \sqrt{t_a \cdot t_b}$.
3. Initialize the exponent, $n = n_0$.
4. Perform linear regression of $y = x^{1/n_0}(t)$ for the first subregion and compute the coefficient of determination, $r_1$.
5. Perform linear regression of $y = x^{1/n_0}(t)$ for the second subregion and compute the coefficient of determination, $r_2$.
6. Compute the mean coefficient of determination:

$$\overline{r} \equiv \frac{r_1 + r_2}{2}.$$

7. Repeat Steps 3–6 for a range of possible $n$.
8. Identify the value of $n$ that maximizes $\overline{r}$.
9. Determine the virtual origin $t_0$ as the $x$-intercept of $x^{1/n}(t)$.

The highest mean coefficient of determination is $\overline{r} = 1.0$, indicating the best fit.

This cross-validation method depends on the chosen region for the fit, $[t_a, t_b]$. We report the decay exponent $n$ and virtual origin $t_0$ corresponding to the highest $\overline{r}$ after varying this range. The results are summarized in Table VII.

TABLE VII. **Best optimized decay exponent $n$ and virtual origin $t_0$ for different experimental setups, determined using the cross-validation method.** The fitting region ($[t_a, t_b]$) and the mean coefficient of determination $\overline{r}$ are also reported.

| Experiment | $n$ | $t_0$ (s) | $t_a$ (s) | $t_b$ (s) | $\overline{r}$ |
|---|---|---|---|---|---|
| Single oscillating grid | -2.06 | -1.63 | 5 | 660 | 0.97 |
| Double oscillating grid | -2.04 | -2.72 | 2 | 660 | 0.96 |
| Vortex ring collision, large blob | -1.32 | -0.15 | 0 | 90 | 0.96 |
| Vortex ring collision, small blob | -1.10 | -1.5 | 0 | 25 | 0.96 |

We argue that the fluctuating energy decay of the double-grid experiment can be adequately fitted with a single power law, whereas the energy decay of the large turbulent blob cannot. Qualitatively, two distinct decay regimes can be observed, as shown in main Figure 2a. Furthermore, the mean coefficient of determination $\overline{r}$ provides quantitative evidence. Table VIII demonstrates that $\overline{r}$ decreases as late-time data are included in the fit.

TABLE VIII. **Incorrectly estimated $n$ and virtual origin $t_0$ for different experimental setups yield a poor mean coefficient of determination $\bar{r}$.**

| Experiment | $n$ | $t_0$ (s) | $t_a$ (s) | $t_b$ (s) | $\bar{r}$ |
|---|---|---|---|---|---|
| Vortex ring collision, large blob (optimized) | -1.32 | -0.15 | 0 | 90 | 0.96 |
| Vortex ring collision, large blob (suboptimal) | -1.71 | -2.81 | 0 | 500 | 0.81 |
| Vortex ring collision, large blob (suboptimal) | -1.76 | -3.70 | 0 | 700 | 0.77 |

### 4. *Estimation of dissipation rate*

Measuring the dissipation rate in turbulence accurately using PIV is challenging. Reference [41] investigated five methods to estimate the dissipation rate from PIV data of zero-mean, gaseous turbulence. They concluded that using the second-order structure function is most robust; however, this method assumes that the flow is turbulent with a substantially large inertial sub-range present. In addition to their findings, our previous work [2] demonstrates that median filtering with a small kernel ($3 \times 3$ px$^2$) greatly improves the estimation combined with the method using the second-order structure function. This method, however, is bound to fail when the turbulence is unsteady and its inertial subrange shrinks.

In this section we present the results of the application of three distinct methods to compute the dissipation rate $\epsilon$ from our high magnification 2D PIV data:

1. The **direct method using the average turbulent energy density**

$$\epsilon_{dq/dt} = -\left\langle \frac{d\langle q\rangle_{\mathbf{x}}(t)}{dt} \right\rangle_n . \tag{59}$$

   In this method, we first average the fluctuating energy $q(\mathbf{x}, t)$ over the field of view, then take its derivative with respect to time, and finally average over the ensemble.

2. The **direct method using the rate-of-strain tensor**:

$$\epsilon_{s_{ij}} = 6\nu\langle(\partial_1 u_1)^2 + (\partial_2 u_2)^2 + (\partial_2 u_1)(\partial_1 u_2)\rangle_{\mathbf{x},\mathrm{n}}. \tag{60}$$

   In this method, we first apply the Savitzky-Golay filter to the PIV velocity fields, then compute the spatial derivative using the central difference method, and finally average over space and ensemble.

3. For the **spectral method**, we find $\epsilon_E$ such that the rescaled three-dimensional energy spectrum $E'(\kappa')$ fits to the universal profile. To obtain this universal profile, we compute $E'_{\mathrm{ref}}(\kappa') = -\kappa' \frac{d}{d\kappa'}\left(\frac{1}{2}E'_{11,\mathrm{ref}}(\kappa') + E'_{22,\mathrm{ref}}(\kappa')\right)$ [42] from a collection of the wind tunnel data in [43]. Here $E'(\kappa')$ denotes the rescaled spectrum function $E'(\kappa') = E(\kappa')/(\epsilon\nu^5)^{1/4}$, and $\kappa' = \kappa\eta = \kappa(\nu^3/\epsilon)^{1/4}$. Instead of using the wind tunnel data, one may also compare the experimental energy spectrum to that from direct numerical simulations of isotropic turbulence available in the Johns Hopkins Turbulence Database [44]. In this method, we identify $\epsilon_E$ by minimizing the difference $|E'(\kappa', t) - E'_{\mathrm{ref}}(\kappa')|$.

4. For the **second-order structure function method**, we adopt a similar approach as the spectral method using the rescaled structure function. The structure function $D_{LL}(r,t) = \langle\delta u^2\rangle/\langle u_i^2\rangle$ is rescaled as $r \to r' = r/\eta$ and $D_{LL} \to D'_{LL} = D_{LL}/(\epsilon r)^{2/3}$ where $\delta u(\vec{x}, r, t) = u_i(\vec{x}+r\hat{x}_i, t) - u_i(\vec{x}, t)$. We then find $\epsilon_{D_{LL}}$ that minimizes the difference function $|D'_{LL}(r', t) - D'_{LL,\mathrm{ref}}(r')|$.

Supplementary Figure 14 shows the dissipation rates estimated by each method for blob and double oscillating grid.

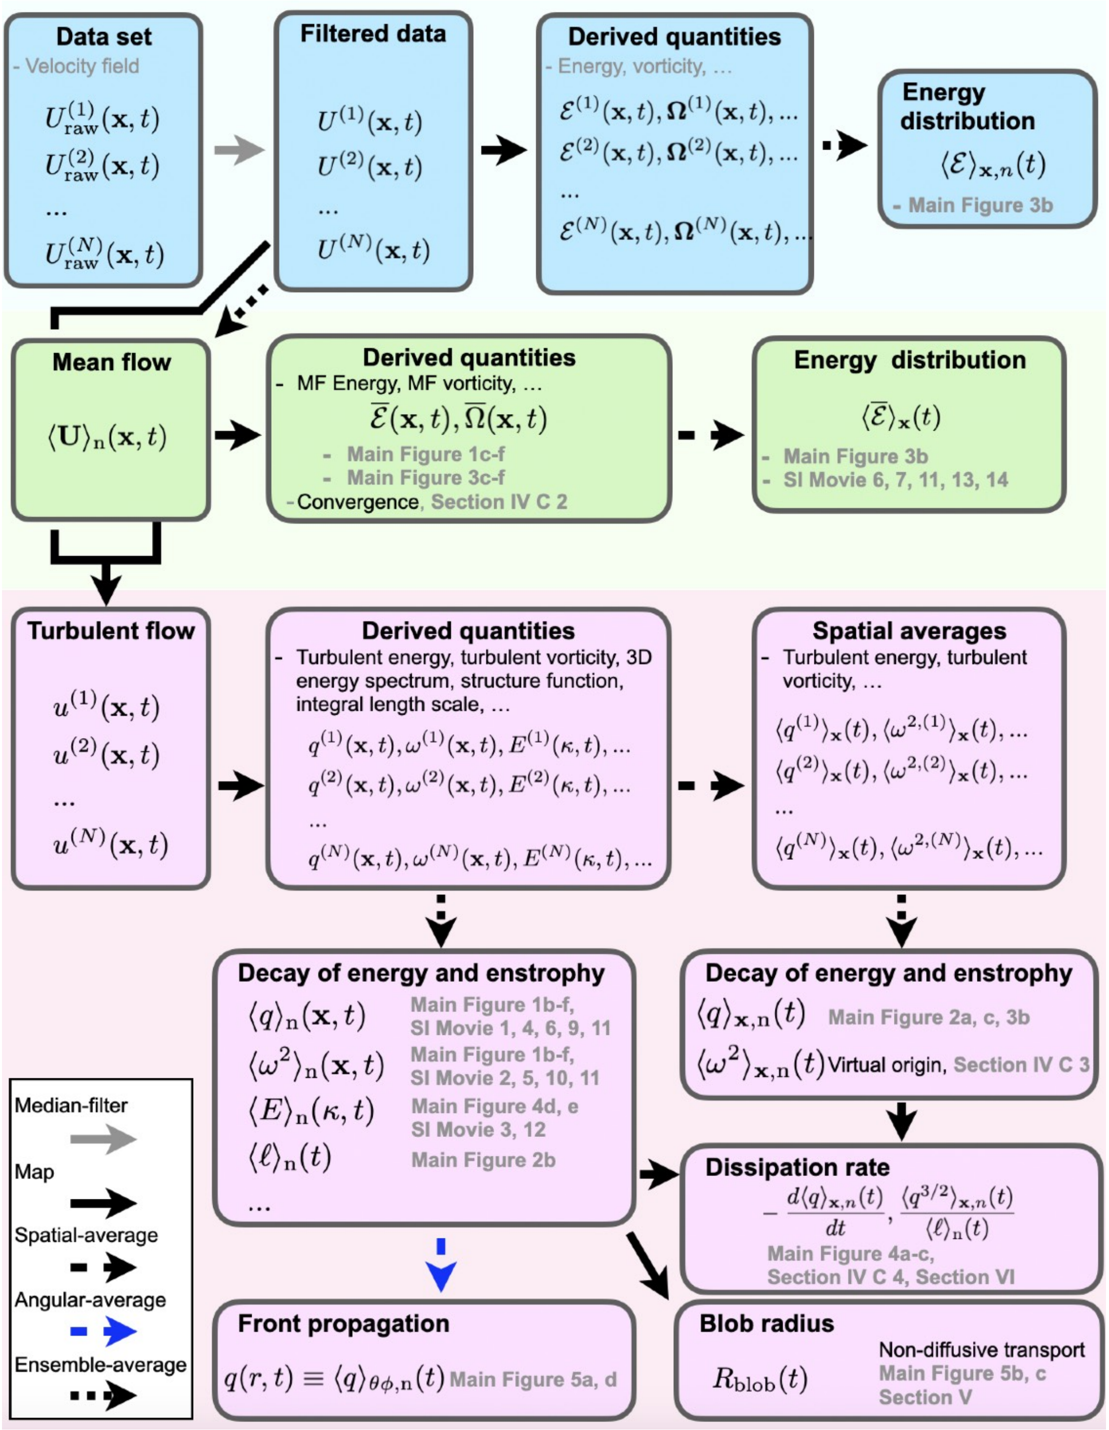


FIG. 11. **Schematic representation of the analysis pipeline used to compute key quantities in this study.** This flowchart outlines the steps for processing raw velocity data, extracting mean and fluctuating components, and deriving quantities such as energy, vorticity, dissipation rate, and other turbulence metrics.

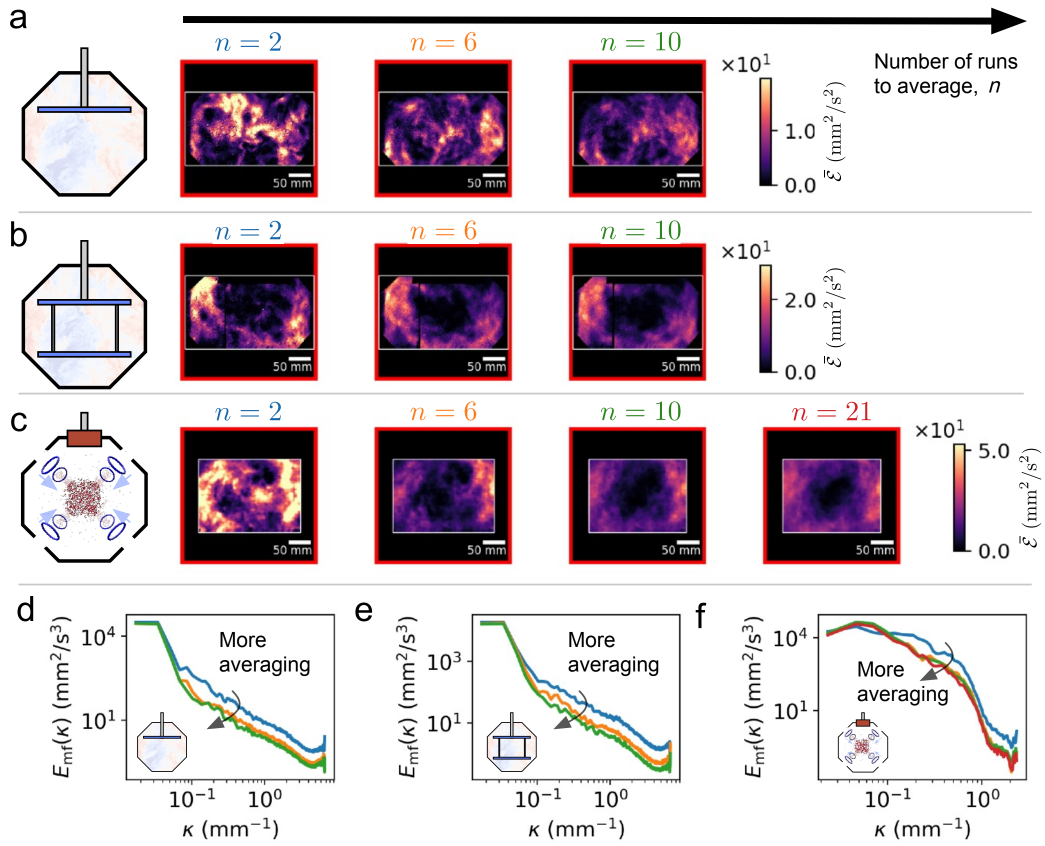


FIG. 12. **Averaging sufficiently many samples results in a converged, time-varying mean flow for each setup.** The mean-flow energy during the decay shows the convergence as more samples are put into averaging for each setup: **(a)** single oscillating grid, **(b)** double oscillating grid, **(c)** turbulent blob. **(d-f)** Energy spectra of the mean flow field for each setup also display the convergence. (d) Single oscillating grid. (e) Double oscillating grid. (f) Turbulent blob. The colors in d-f correspond to the number of realizations used to average, namely $n = 2$ (blue), $n = 6$ (orange), $n = 10$ (green), and $n = 21$ (red).

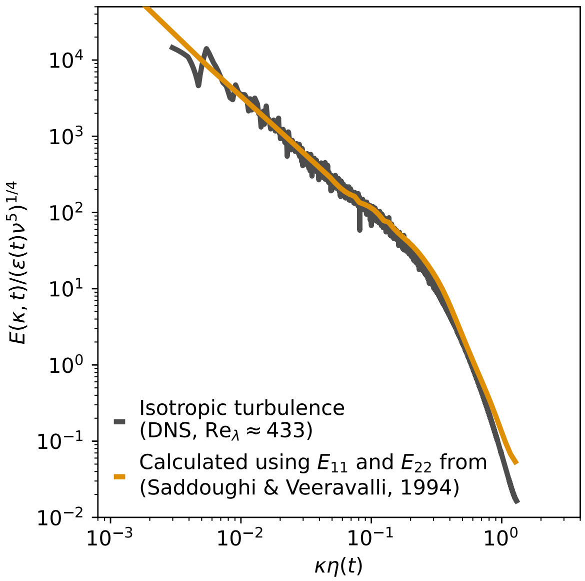


FIG. 13. **Comparison of 3D energy spectra of homogeneous isotropic turbulence between DNS ($Re_\lambda \approx 418$) and wind-tunnel experiments ($Re_\lambda = 23 - 3180$), adapted from [43].** The DNS data is taken from [44]. Experimental spectra are reconstructed using only the inertial and dissipation ranges of the original data.[a]

[a] The original data consist of a collection of rescaled 1D energy spectra $E_{11}/(\epsilon\nu^5)^{1/4}$ and $E_{22}/(\epsilon\nu^5)^{1/4}$. For a meaningful comparison, we compute $E(\kappa) = -\kappa\frac{d}{d\kappa}\left[\frac{1}{2}E_{11}(\kappa) + E_{22}(\kappa)\right]$.

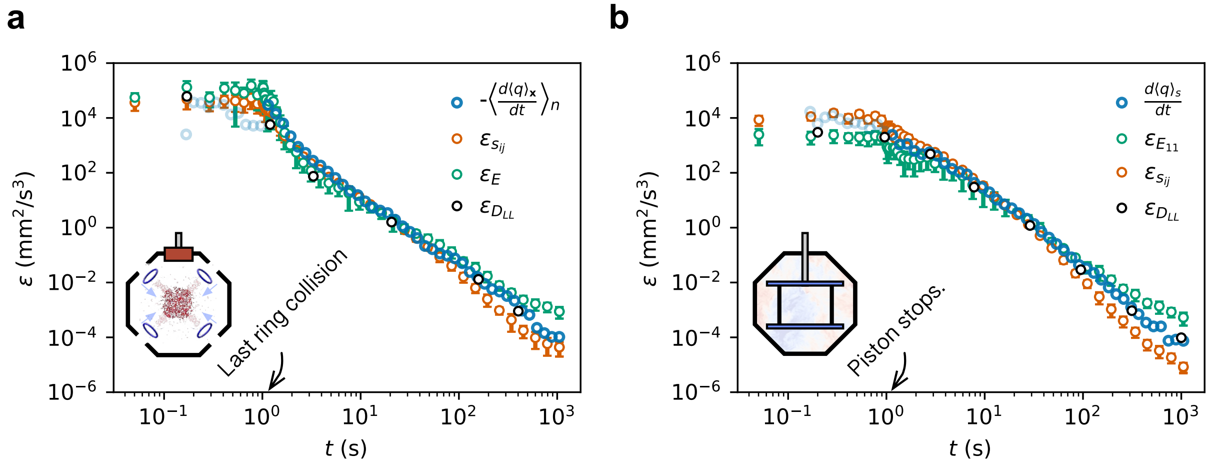


FIG. 14. **Comparison of multiple methods for estimating dissipation rate in turbulent flows.** (**a**) turbulence initiated by repeated vortex ring collisions, and (**b**) turbulence initiated by a double oscillating grid. Methods include the direct method using average turbulent energy density $-\left\langle \frac{d\langle q\rangle_{\mathbf{x}}(t)}{dt}\right\rangle_{\mathrm{n}}$, the rate-of-strain tensor method $\epsilon_{s_{ij}}$, the spectral method $\epsilon_E$, and the structure function method $\epsilon_{D_{LL}}$ ($n = 21$). The error bar represents SEM.

## V. NONLINEAR DIFFUSION OF A TURBULENT BLOB

In this section we supplement the discussion in the main text providing a more detailed comparison between experimental data and the Kolmogorov-Barenblatt turbulent energy balance equation:

$$\partial_t q(\mathbf{x}, t) = \frac{2}{3} c_0 \ell(t) \nabla^2 q^{3/2}(\mathbf{x}, t) - \epsilon_0 \frac{q^{3/2}(\mathbf{x}, t)}{\ell(t)}.$$

### A. Spatiotemporal evolution of the turbulent energy on a two-dimensional slice

Supplementary Figure 15 shows the spatiotemporal evolution of the turbulent energy in a blob, comparing experimental data with the result of the CDS simulation on a two-dimensional slice.

The CDS simulations were performed in 3D using the experimentally observed $\ell(t) = 0.1 L_{\text{box}}(t - t_0)^{0.38}$ (Supplementary Figure 16). A two dimensional slice through the center was then taken for comparison with the experimental 2D PIV measurements. The three-dimensional initial condition for the CDS simulation, is constructed by taking our single experimental 3D velocimetry measurement, and smoothing it with a Gaussian filter. As seen in the left column of Supplementary Figure 15, the spatial inhomogeneity in this distribution is quickly smoothed out by the nonlinear diffusion term, highlighting the effectiveness of the nonlinear diffusion term in smoothing initial asymmetries and providing a robust prediction of the average front dynamics.

The center and right columns of Figure 15 show the evolution of the turbulent energy field measured on a single two-dimensional slice. The energy distributions are reported for a single run (right) and an ensemble-average over $n = 10$ runs (center). The turbulent-energy fields from single experimental run, showed in the right column, remain strongly inhomogeneous and the blob expands in a branched, non-uniform manner. The ensemble-averaging yields a significantly smoother energy distribution, in closer agreement with the CDS prediction for the mean-field energy distribution.

The envelope of the energy distribution shows good agreement between CDS simulation and experiment. The experimental data shows stronger fluctuations within the blob, however the contrast between the single realization and the ensemble average (n=10) supports the notion that the additional granularity of the experimental energy distribution is a simple consequence of the limited ensemble averaging.

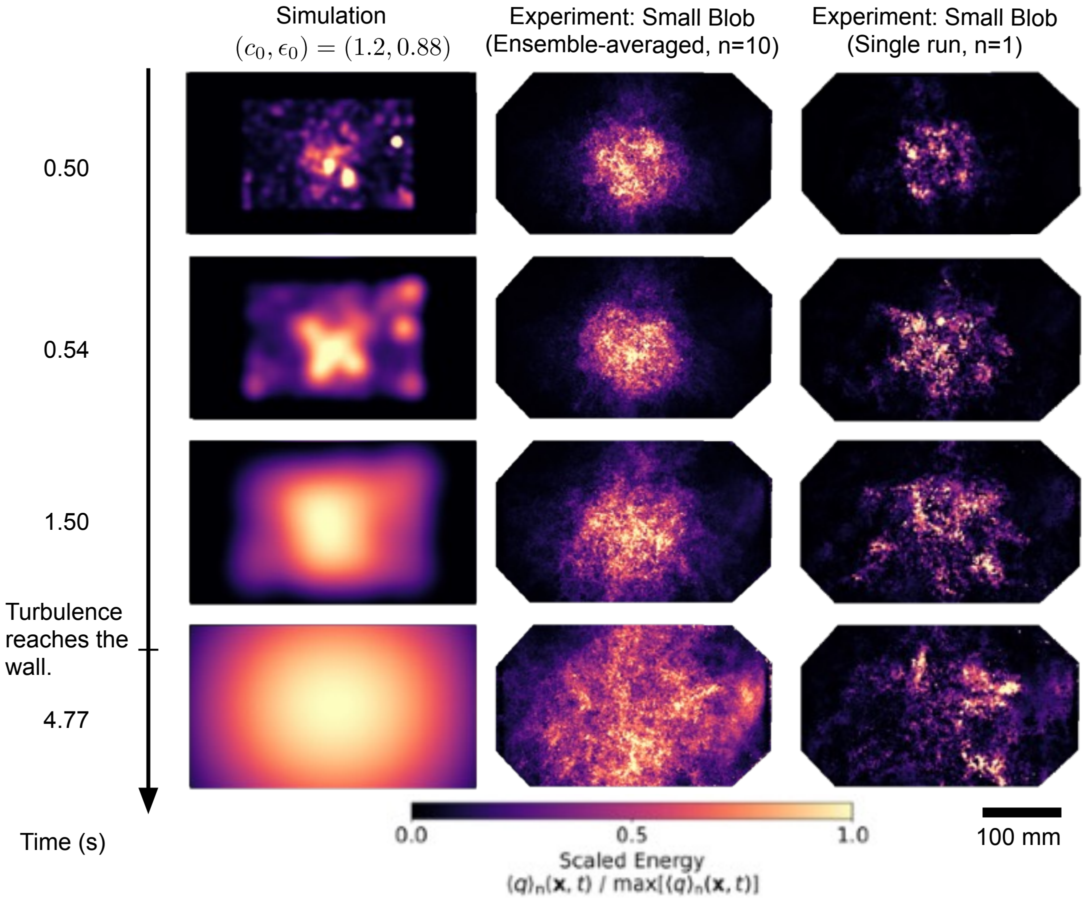


FIG. 15. **The proposed governing equation describes ensemble-averaged dynamics.** Left column: CDS simulation with $(c_0, \epsilon_0) = (1.2, 0.88)$ and $\ell(t) = 0.1(t-t_0)^{0.38}$. The turbulent energy field on the central slice in the simulation box ($L_{\text{box}} = 5$, spacing $dx = 0.05$). For the initial condition, we filter a 3D raw energy distribution, extracted using 3D PTV, padded with zero, and smoothed with a Gaussian filter to suppress numerical instability. The simulation starts with the experiment IC at $t = 0.5$ s and the time step is dt $= 0.0005$. Middle column: Ensemble-averaged turbulent energy field on the central slice, extracted using 2D PIV (Small blob, $\text{Re}_\lambda = 60$, $n = 10$) Right column: Turbulent-energy field on the central slice from a single experimental run, extracted using 2D PIV; unlike the ensemble average, its evolution is highly sensitive to initial condition and spreads in a branching pattern.

## B. Evolution of the second moment of the turbulent kinetic energy

Supplementary Figure 17 and main Figure 5b-c, shows the rate of expansion of the second moment of the turbulent fluctuation energy $\dot{R}_{\text{blob}}$ compared with the contribution to the predicted rate coming from each term in the Kolmogorov-Barenblatt turbulent energy balance equation. Details of how we measured the rate of expansion and computed the predictions of the turbulent energy balance equation are as follows.

We define the characteristic radius of a turbulent blob using the second moment of the turbulent kinetic energy $q(\mathbf{x}, t)$:

$$R^2_{\text{blob}}(t) = \frac{\int_{\mathcal{V}} r^2 q(\mathbf{x}, t) d\mathbf{x}}{\int_{\mathcal{V}} q(\mathbf{x}, t) d\mathbf{x}} = \frac{\int_{\mathcal{V}} r^4 q(r, t) dr}{\int_{\mathcal{V}} q(r, t) dr}.$$

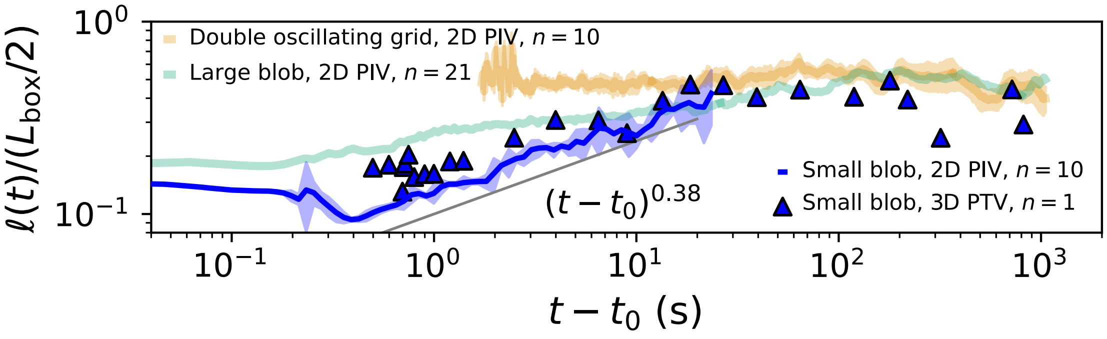


FIG. 16. **Evolution of the integral length scale (Small blob, $Re_\lambda = 60$) in comparison with the large blob and double oscillating grid experiments.** The integral length scale is computed using $\ell(t) = (3\pi/4)\int_0^\infty \kappa^{-1}E(\kappa,t)d\kappa \;/\; \int_0^\infty E(\kappa,t)d\kappa$, and then averaged over 10 realizations. Error bars indicate the standard error of the mean (SEM). For the small blob, $\ell(t)$ is approximated as $\ell(t) = 0.1(t-t_0)^{0.38}$ with $t_0 = 0.5$ s for $t - t_0 < 30$ s, and saturates at $0.23L_{\rm box}$. Triangles indicate values computed from the energy spectrum of the *raw* velocity field, serving as a reference for late-time behavior.

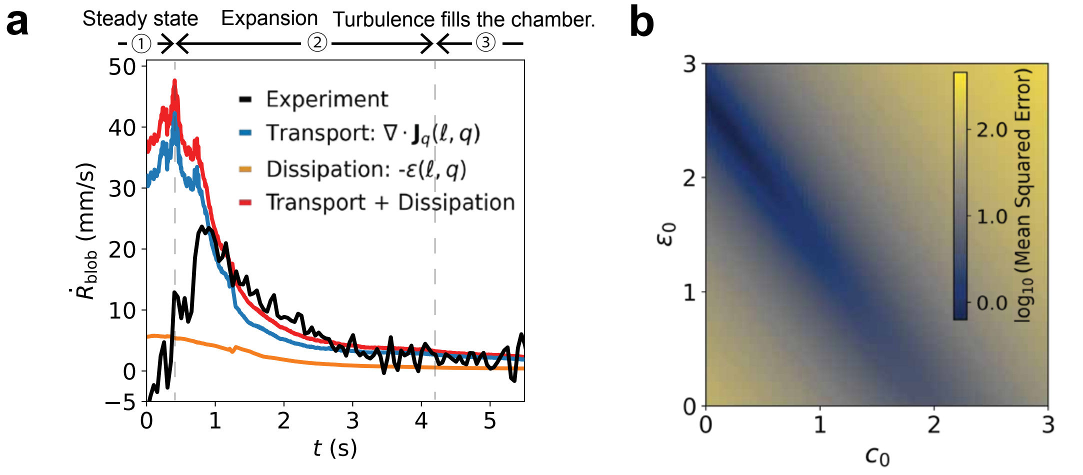


FIG. 17. **Front propagation and dynamic scaling during turbulence spreading. (Replicated from main Figure 5b-c)** (**a**) The growth rate of the blob's characteristic radius $\dot{R}_{\rm blob}$ is compared with the prediction from Eq. 16, using coefficients $c_0 = 1.2$ and $\epsilon_0 = 0.88$. The experimental curve is obtained from the ensemble-averaged turbulent energy field ($n = 10$). (**b**) Transport and dissipation coefficients are estimated by minimizing the mean-squared error of $\dot{R}_{\rm blob}(t)$ between the theoretical prediction and experimental data. We evaluate the logarithm of the mean-squared error over $1.2 \le t \le 5$ s and show it on the $c_0 - \epsilon_0$ plane.

Here, $q(r,t) = \langle q \rangle_{\theta\phi,{\rm n}}(r,t)$ represents the turbulent energy averaged over angles and realizations. We denote the numerator and denominator as $P(t)$ and $Q(t)$, respectively:

$$R^2_{\rm blob}(t) = \frac{P(t)}{Q(t)}$$

where

$$P(t) = 4\pi \int r^4 q(r,t)dr, \quad Q(t) = 4\pi \int r^2 q(r,t)dr.$$

By taking the derivative of $R^2_{\text{blob}}(t)$, we obtain

$$\frac{dR_{\text{blob}}}{dt} = \frac{1}{2R_{\text{blob}}} \frac{P'(t)Q(t) - P(t)Q'(t)}{Q^2(t)}.$$

We note that

$$P'(t) = 4\pi \int r^4 \partial_t q(r,t)\, dr, \quad Q'(t) = 4\pi \int r^2 \partial_t q(r,t)\, dr.$$

The incremental change in $R_{\text{blob}}(t)$ over a time interval $\Delta t$ is approximated as

$$\Delta R_{\text{blob}}(t) \approx \frac{\Delta t}{2R_{\text{blob}}} \frac{\int \left[Q(t)r^4 - P(t)r^2\right] \partial_t q(r,t)\, dr}{Q^2(t)}.$$

Using the Kolmogorov-Barenblatt turbulent energy balance equation:

$$\partial_t q(\mathbf{x},t) = \frac{2}{3} c_0 \ell(t) \nabla^2 q^{3/2}(\mathbf{x},t) - \epsilon_0 \frac{q^{3/2}(\mathbf{x},t)}{\ell(t)},$$

we can readily compute the contributions to $\partial_t q(x,t)$ from the nonlinear diffusive term and energy dissipation term as:

$$\delta q_1(\mathbf{x},t) = \Delta t \cdot \frac{2}{3} c_0 \ell(t) \nabla^2 q^{3/2}(\mathbf{x},t), \quad \delta q_2(\mathbf{x},t) = -\Delta t \cdot \frac{\epsilon_0 q^{3/2}(\mathbf{x},t)}{\ell(t)}.$$

The change in $R_{\text{blob}}(t)$ due to transport $\delta q_1$ and dissipation $\delta q_2$ are then:

$$\Delta R_{\text{blob},i}(t) = \frac{2\pi}{R_{\text{blob}}(t)} \frac{\int [Q(t)r^4 - P(t)r^2] \delta q_i(r,t) dr}{Q^2(t)}. \quad (61)$$

SI Figure 17 and main Figure 5c, show the mean squared error computed as the mean squared difference between the measured $\dot{R}(t)$ and the piecewise predicted $\dot{R}(t)$ as a function of the value of $c_0$ and $\epsilon_0$. There is a linear band of minima (dark blue) that correspond to combinations of $c_0$ and $\epsilon_0$ that minimize the error. Our experimentally determined value of $\epsilon_0 = 0.88$, as well as values of $\epsilon_0$ reported in the literature, summarized in Table IX, all fall well below the value $\epsilon_0 \lesssim 1.6$ corresponding to a value along the band of minima of $c_0 \gtrsim 1$. Thus nonlinear diffusion is both required and successful in capturing the growth of the turbulent region. For our experimentally determined value of $\epsilon_0 = 0.88$, the minimum square error occurs for $c_0 = 1.2$ making nonlinear diffusion the dominant contribution to $\dot{R}(t)$ throughout the spreading phase.

### C. Evolution of the azimuthally averaged turbulent kinetic energy front shape

In main Figure 5 c,d we report the evolution of the shape of the azimuthally averaged turbulent kinetic energy front for a small blob. In this subsection we describe the procedures used to process and rescale the data.

We use the first second of the recording, when the blob is in a steady state, to find the center of the blob. We compute the center using the ensemble-averaged turbulent energy field: $x_i^{\text{center}} = \int \langle q(\mathbf{x},t)\rangle_{n,t<1\text{ s}}\, x_i d\mathbf{x} \;/\; \int \langle q(\mathbf{x},t)\rangle_{n,t<1\text{ s}}\, d\mathbf{x}$. To examine the front shape, we start with ensemble-averaged turbulent kinetic energy $\langle q\rangle_n(\mathbf{x},t)$ and compute its azimuthal average $\langle q\rangle_{\phi,n}$ with the origin of the azimuthal coordinates at the estimated center of the blob. In the CDS simulation, for which there is three-dimensional data, we take an average over polar and azimuthal angles $\langle q\rangle_{\theta\phi}$.

We note that this one-dimensional profile is denoted in both cases as $\langle q \rangle_\Omega$ in figure 5 of the main text for notational coherence.

The raw profile of the turbulent kinetic energy at a collection of times is shown on the left in main Figure 5d and e. The center plots show the same curves, normalized by the average value in the central region ($r \leq 15$ mm). To find a value of $\vartheta'$ that collapses the experimental curves, we apply $r \to r/(t-t_0)^{\vartheta'}$ to all radial profiles recorded before $t - t_0 = 5.5$ s using an initial guess for $\vartheta'$, we then average the transformed curves and compute the residual sum of squares (RSS) on the difference between this average curve and each individual curve at a given time. Finally we sum these residuals to produce a metric that quantifies the degree of data collapse for a given exponent $\vartheta'$. We repeat this procedure for a range of $\vartheta'$, and determine $\vartheta'$ with the minimal sum of the RSS. We take this to be the optimal scaling exponent for $h$ (See Eq. 47, 50 and Section IIIC for details about the scaling derived from the theory and simulations) and plot the rescaled curves in the right column.

For the CDS simulations, we examine the scaling $h \sim t^{\vartheta}$ in the cases $\epsilon = 0$ and $\epsilon \neq 0$. See §IID for a discussion of the $\epsilon = 0$ case and §IIIC for the $\epsilon \neq 0$ case. The right plot in the main Figure 5e, is produced by transforming r as $r \to r/(t-t_0)^{\vartheta}$ where $\vartheta = 0.389$ as found in §IIIC.

### D. $\dot{R}_{\rm blob} - q$ scaling

Another way to test the predictions of the Kolmogorov-Barenblatt turbulent energy balance equation against our data is to consider the dependence of the expansion rate $\dot{R}_{\rm blob}$ and the energy at the center of the blob $q_0 = q(r = 0, t)$. Using Eq. 49, the Kolmogorov-Barenblatt turbulent energy balance equation for a spherical expanding blob, combined with an imposed $\ell \sim t^\gamma$ predicts:

$$\dot{h} \sim q_0^{\frac{5-2\gamma}{6(1+\gamma)}}.$$

We note that for spherically symmetric expanding blobs, one can relate $h$ to $R_{\rm blob}$ by $h = \sqrt{3}R_{\rm blob}$. Hence, the predicted scaling of $\dot{R}_{\rm blob}$ is the same as that for $\dot{h}$. For comparison, consider ordinary diffusion with a constant diffusion coefficient: $\partial_t q(\mathbf{x}, t) = c\nabla^2 q(\mathbf{x}, t)$. The spherically symmetric self-similar solution in this case is Gaussian, and its characteristic length scale can be defined through its second moment, which is equal to a standard deviation. The resulting scaling law would be $\dot{R}_{\rm blob} \sim q_0^{1/3}$. Our experimental data span less than a decade since turbulence quickly reaches the wall. Within this limited range we find that the scaling deviates from the ordinary constant diffusion scenario. Supplementary Figure 18 shows the result for Dataset 1, whose integral length scale grows as $t^{0.38}$ ($\gamma = 0.38$). The predicted exponent of the turbulent front propagation speed is

$$\frac{5 - 2\gamma}{6(1 + \gamma)} = 0.51,$$

aligning more closely with experimental observations, as shown in Supplementary Figure 18.

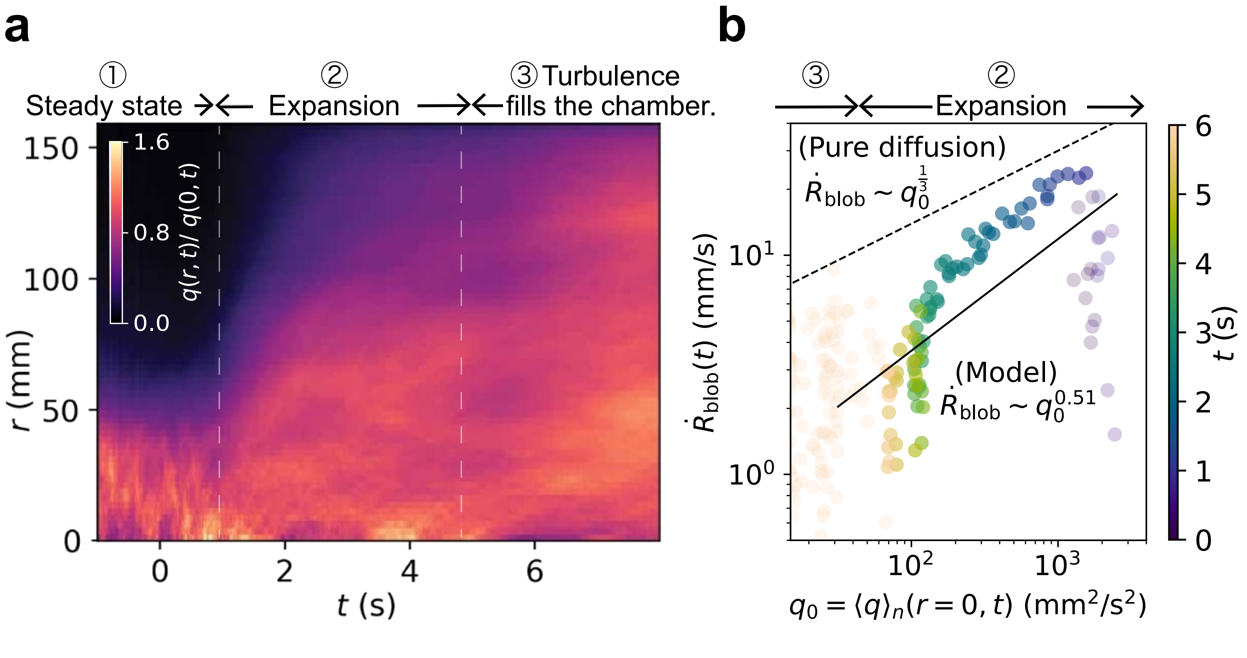


FIG. 18. **Nonlinear propagation of a turbulent blob (a)** Kymograph of an expanding turbulent blob, represented by the scaled turbulent energy. The field is ensemble-averaged ($n = 10$) and then averaged over azimuthal angle. **(b)** The propagation speed, plotted against the turbulent energy within the blob, agrees better with the scaling predicted by the nonlinear diffusion model than with that predicted for pure diffusion.

### E. Energy decay: capturing the effects of persistent inhomogeneity by decreasing the value of $c_0$

In the main text, we provide a possible range for the transport and dissipation coefficients, $c_0$ and $\epsilon_0$. Our measurements suggest $c_0 = 1.20 \pm 0.11$ (main Figure 5c) and $\epsilon_0 = 0.88 \pm 0.10$ (main Figure 4b). As we simulate the energy decay using the CDS method with these parameters and the experimentally obtained $\ell(t)$, the energy decay of the simulation differs substantially from the experiments (blue curve in main Figure 3c).

Furthermore, a contradiction between the late time predicted mean field energy distribution, which is inevitably smooth, and the experimentally observed distribution is also visible in Supplementary Movies 6 and 8. The dominant flow structure observed at late times resembles a chamber-filling vortex, that slowly churns the fluid, illustrated in Supplementary Figure 19. This late time structure is similar in all experimental runs as well as across forcing methods (e.g. Supplementary Movie 11), suggesting it arises from an interaction with the flow chamber after the turbulence hits the walls.

Capturing this type of interaction, which can bias ensemble averages by introducing a correlation between realizations, as well as feed energy into turbulent structures at late times, is beyond the scope of the Kolmogorov-Barenblatt turbulent energy balance equation. To account for the turbulence-chamber interaction additional modeling is required. Interestingly, we find that if we lower the value of $c_0$ after turbulence reaches the wall (red curve in main Figure 3c), much better agreement can be achieved. The rationale for this observation can be understood by inspection of the Kolmogorov-Barenblatt turbulent energy balance equation:

$$\partial_t q(\mathbf{x},t) = \frac{2}{3} c_0 \ell(t) \nabla^2 q^{3/2}(\mathbf{x},t) - \epsilon_0 \frac{q^{3/2}(\mathbf{x},t)}{\ell(t)}.$$

In the simulation, the transport term rapidly smooths the turbulent energy field, and once the field becomes uniform, the dissipation term dominates the dynamics, resulting in $q \sim t^{-2}$. Thus, the onset of dissipation-dominant dynamics is linked to the inhomogeneity of the flow. If the turbulent energy remains inhomogeneous, the crossover between propagation-dominant and dissipation-dominant dynamics is delayed.

Reducing the energy diffusion coefficient $c_0$ from 1.2 to 0.001 at $t - t_0 = 2.15$ s reduces the predicted homogeneity of the flow, allowing the turbulent energy field to remain inhomogeneous for longer, as illustrated in Supplementary Figure 20. This adjustment produces much improvement in the prediction of the crossover for the energy decay, as shown by the red curve in main Figure 2.

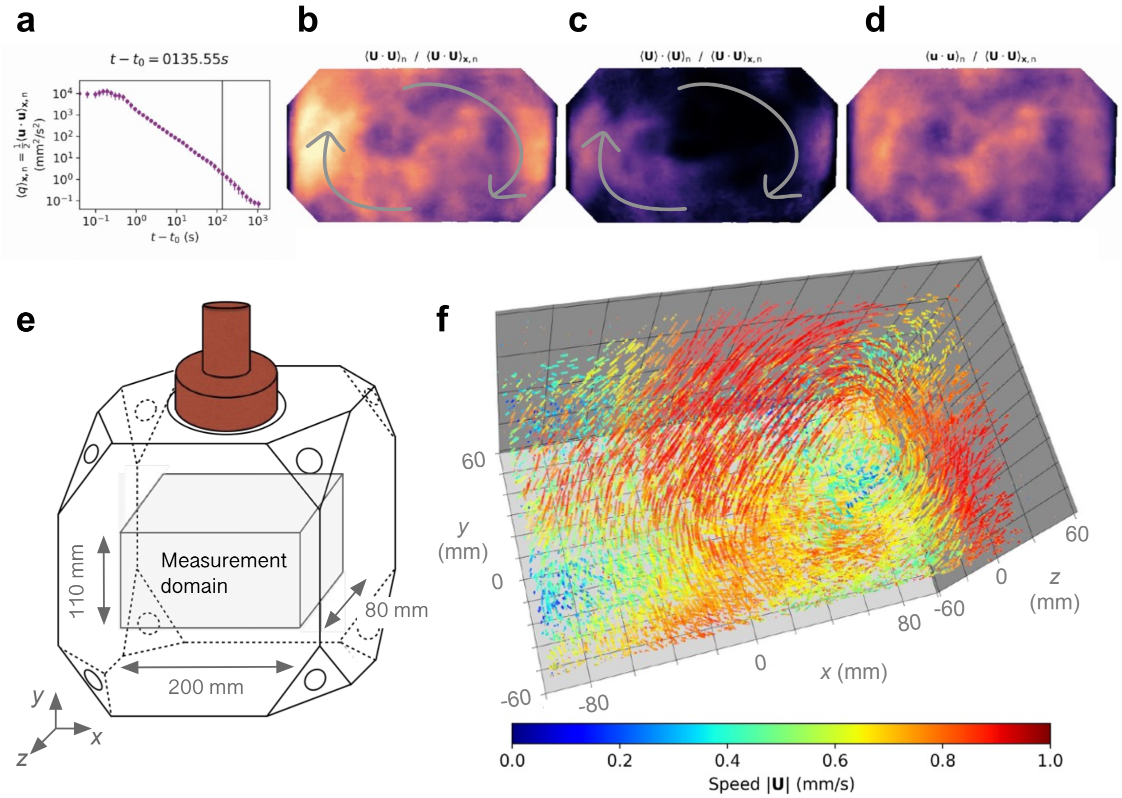


FIG. 19. **Eddy structure persists at late stages of decay (large blob, Re$_\lambda$ = 203, $n$ = 21, $t - t_0$ = 135.55 s).** **(a)** Spatial- and ensemble-averaged turbulent kinetic energy $\langle q \rangle_{\mathbf{x},\mathrm{n}}(t)$. **(b)** Normalized instantaneous kinetic energy field shows clockwise advection of energy by a large vortex. **(c)** Normalized mean flow kinetic energy field highlights the same vortex. **(d)** Turbulent energy remains inhomogeneous at late times. **(e)** A schematic of the 3D velocimetry measurement volume inside the flow chamber. **(f)** Pathlines from a single experimental realization are shown, revealing a large vortex at late stages of the decay.

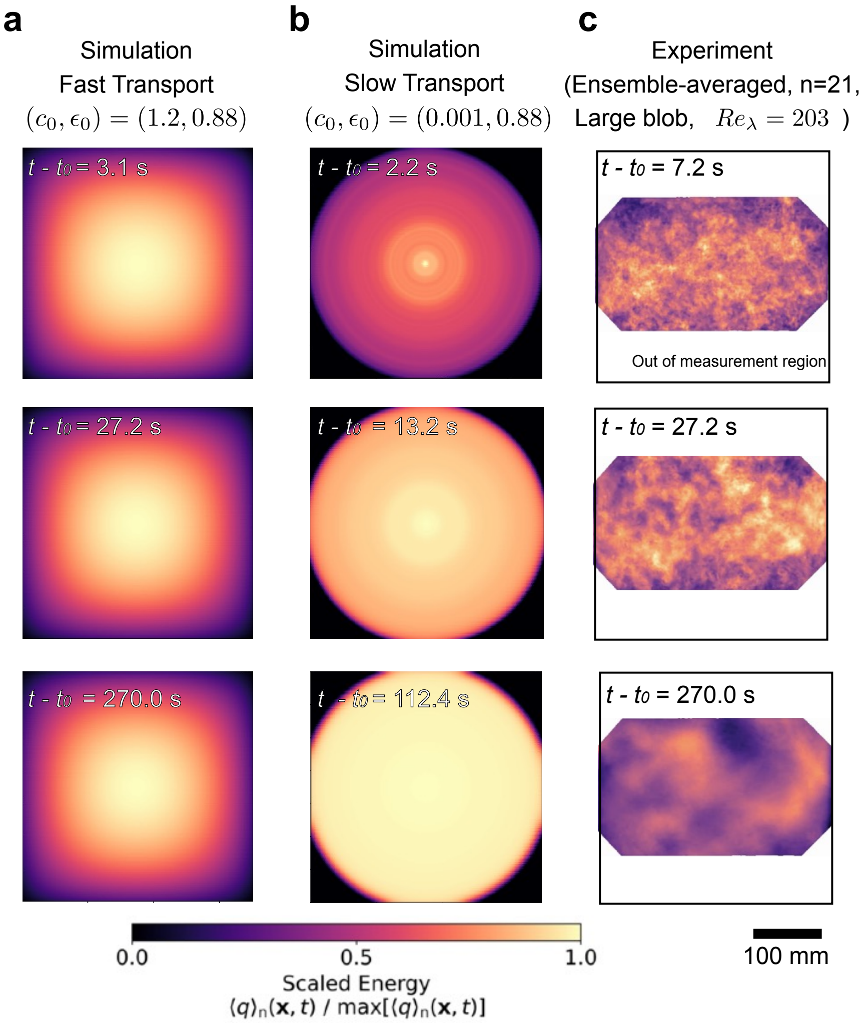


FIG. 20. **Reducing the value of $c_0$ preserves the inhomogeneity in the energy field longer. (a)** Normalized turbulent energy field on the 2D central slice, simulated with the transport and dissipation coefficients, $c_0 = 1.2$ and $\epsilon_0 = 0.88$. We construct the initial condition by smoothing the experimentally measured, 3D energy field with a Gaussian filter and padding zeros in the missing region. While the energy continues to decay, the spatial structure reaches an asymptotic state quickly after it reaches the wall at $t - t_0 = 1$ s. **(b)** Normalized turbulent energy field, simulated with the transport and dissipation coefficients $c_0 = 0.001$ and $\epsilon_0 = 0.88$. With reduced value of $c_0$ the spatial inhomogeneity is preserved longer. The black regions persist as the low value of $c_0 = 0.001$ significantly limits spreading of turbulent energy. **(c)** Normalized, ensemble-averaged turbulent energy field on the 2D central slice from the experiments. The field remains inhomogeneous throughout the decay. The box represents the dimensions of the flow chamber.

## VI. DIMENSIONLESS DISSIPATION RATE: COMPARISON WITH LITERATURE VALUES

In this section, we compare the dimensionless dissipation rate $\epsilon_0 = \epsilon\ell/q^{3/2}$—reported to be $0.88 \pm 0.10$ for a turbulent blob and $1.2 \pm 0.11$ for a double oscillating grid (Supplementary Figure 4b) in our paper—with values from the literature. Sreenivasan (1984) [45] compiled grid-turbulence results from multiple researchers, and found $\epsilon_0 \approx 1$, while later DNS results [46] reported lower values (0.27–0.41). Reported $\epsilon_0$ values vary due to inconsistent definitions of the integral length scale and $\epsilon_0$, complicating direct comparisons. Table IX summarizes values from the literature using our convention. The list is not exhaustive; studies lacking explicit $\epsilon_0$ estimates were excluded.

Chamber geometry and flow structure also affect $\epsilon_0$. Notably, despite using the same chamber, the measured values from our experiments differ by 25%. Table IX shows $\epsilon_0$ ranges from 0.36 to 3.8 across systems varying in medium (air, water, helium II) and chamber geometry. Our measurements fall within this reported range.

It is worthwhile to comment on the Reynolds number dependence of $\epsilon_0$ as it is central to the dissipation anomaly [47]. As summarized in the Table IX, the experimental evidence has shown little clear dependence on the Reynolds number, possibly due to the weak scaling predicted as $1/(\ln \mathrm{Re})^2$ [48].

TABLE IX. Reported Values of the Dimensionless Dissipation Rate in the Literature and This Study

| $\epsilon_0 = \epsilon\ell/q^{3/2}$ | $\mathrm{Re}_\lambda$ | Definition of Integral Length Scale | System | Medium | Literature |
|---|---|---|---|---|---|
| 0.8 - 1.6 | 7-15 | $\int_0^\infty f(r,t)dr$ [a] | Biplanar square grid | Air | [45, 49] |
| 1.2 - 1.4 | 10 | $\int_0^\infty f(r,t)dr$ | Biplanar square grid | Air | [45, 50] |
| 0.70 - 0.87 | 20 - 40 | $\int_0^\infty f(r,t)dr$ | Biplanar square grid | Air | [45, 51] |
| 0.76 - 0.87 | 30 | $\int_0^\infty f(r,t)dr$ | Biplanar square grid | Air | [45, 52] |
| 0.7 - 1.4 | 30 - 120 | $\int_0^\infty f(r,t)dr$ | Parallel rods and slats grid | Air | [45, 53] |
| 0.54 - 0.60 | 40 | $\int_0^\infty f(r,t)dr$ | Biplanar square grid | Air | [45, 54] |
| 0.8 | 40 | $\int_0^\infty f(r,t)dr$ | Biplanar square grid | Air | [45, 55] |
| 0.8 | 40 | $\int_0^\infty f(r,t)dr$ | Biplanar square grid | Air | [45] |
| 0.27 - 0.38 | 40 - 587 | $\int_0^\infty f(r,t)dr$ | Two facing jet arrays | Air | [56] |
| 0.6 | 40 - 500 | $\int_0^\infty f(r,t)dr$ | Biplanar square grid | Air | [45, 57] |
| 0.20 | 55[b] | $\int_0^\infty f(r,t)dr$ | Magnetic stirrers | Water | [58] |
| 0.6 | 150 | $\int_0^\infty f(r,t)dr$ | Biplanar square grid | Air | [45, 59] |
| 0.49 | 50 - 473 | Length at which $k_1 E_{11}$ peaks | Biplanar square grid | Air | [60] |
| 2.3 | 216 - 1054 | $2\pi \left[\frac{5}{11}\sqrt{\frac{A}{C^3}}(t+t_0)\right]$ [c] | Biplanar grid | He II | [61] |
| 0.54 - 0.65 | 500 | $\int_0^\infty f(r,t)dr$ | Biplanar square grid | Air | [62] |
| 3.8 | 634 | Full-width of a grid | Planar slotted grid | He II | [14] |
| 0.95 | 634 | A quarter of the grid width [d] | Planar slotted grid | He II | [14] |
| 0.7 - 1.3 | 99 - 130 | $\int_0^\infty f(r,t)dr$ | Array of jets | Air | [45, 63] |
| $0.88 \pm 0.10$ | 10 - 100 | $\frac{3\pi}{4q}\int_0^\infty \frac{E(\kappa)}{\kappa}d\kappa$ [e] | Vortex ring collision | Water | current work |
| $1.20 \pm 0.11$ | 10 - 185 | $\frac{3\pi}{4q}\int_0^\infty \frac{E(\kappa)}{\kappa}d\kappa$ | Double oscillating grid | Water | current work |

[a] $f(r,t)$ is the longitudinal velocity autocorrelation function: $f(r,t) = \langle u_1(\mathbf{x},t)u_1(\mathbf{x}+\mathbf{r})\rangle_{\mathbf{x}}/\langle u_1^2(\mathbf{x},t)\rangle_{\mathbf{x}}$.
[b] Only the Reynolds number is provided in this paper. For reference, we use $\mathrm{Re}^{1/2} = \sqrt{3000} \approx 55$, where $Re = u'\ell(t=0)/\nu$.
[c] $A$ and $C$ are coefficients in the energy spectrum function: $E(\kappa) = A\kappa^2$ in the energy-containing range, and $E(\kappa) = C\epsilon^{2/3}\kappa^{-5/3}$ in the inertial subrange.
[d] Here, we assume that $\ell$ saturates to a quarter of the system size as observed in our current work.
[e] In homogeneous, isotropic turbulence, this expression is identical to $\int_0^\infty f(r,t)dr$ [42].

## VII. TURBULENCE GENERATED BY A SINGLE OSCILLATING GRID

In the main text, we present two methods to generate turbulence in the *same flow chamber*, showing that they decay in different fashions. We argue that the essential difference comes from how the integral length scale grows throughout the decay. In this section, we present the third method of generating turbulence using a single oscillating grid. This method generates a strong, unidirectional mean flow, presenting a more complex decay dynamics compared to the double oscillating grid as it takes more time for the turbulence to establish homogeneity and isotropy. Nevertheless, our analysis suggests that this method produces turbulence whose decay behavior lies between that of the double oscillating grid case ($\ell = \text{const.}$) and the turbulent blob case ($\ell \sim t^{\gamma}$, then $\ell = \text{const.}$).

### A. Temporal evolution

Supplementary Figure 21 illustrates the evolution of energy, vorticity, and enstrophy over time. The primary difference between the single and double oscillating grids lies in the initial mean flow structure. The single oscillating grid generates a strong downward flow as it oscillates, as shown in Supplementary Figure 21c. This downward mean flow settles approximately 10 seconds after the grid stops moving. Turbulence develops as energy is transferred from the mean flow to the fluctuating field, peaking at $t = 30$ s and remaining dominant throughout the decay process. For $t > 10$ s, energy continues to decay, and the vortical structures coarsen over time, as shown in Supplementary Figure 21 d-e, resembling the behavior observed in the double oscillating grid and turbulent blobs.

### B. Energy decay and integral length scale

Supplementary Figure 22a shows the tubrulent energy decay in the single grid experiments as well as the resutls from the double oscillating grid and turbulent blob experiments. The single oscillating grid experiments show the decay somewhere intermediate between the double oscillating grid and turbulent grid. In early time ($t - t_0 < 5$ s), energy is still being converted from the mean flow to the turbulent field, while overall energy continues to decay. After this transient period, turbulence is established ($t - t_0 \approx 5$ s). Our analysis on the virtual origin suggests a power law of $t^{-2}$ between $t - t_0 = 5 - 660$ s. For $t - t_0 > 660$ s, turbulent energy reaches a plateau, suggesting that it reached a steady state.

During the $t^{-2}$ decay, integral length scale $\ell$ is approximately constant, as shown in Supplementary Figure 22b, which is expected behavior. In the early times (2 s $< t - t_0 <$ 5 s , the integral length scale grows. While we cannot fully determine if it is a power-law growth, turbulent energy does not clearly decay in $t^{-2}$ fashion.

### C. Turbulence statistics

In this section, we report the turbulence statistics observed in the single oscillating grid experiments, mirroring the discussion in the main text for the vortex-ring-generated blob and the double-grid experiments.

The dissipation rate $-d\langle q\rangle_{\mathbf{x},\mathrm{n}}(t)/dt$ remains consistent with the scaling $\langle q^{3/2}\rangle_{\mathbf{x},\mathrm{n}}(t)/\ell(t)$ between $5\,\mathrm{s} < t - t_0 < 660\,\mathrm{s}$, confirming that the flow remains turbulent during this period (Supplementary Figure 23a). The dimensionless dissipation rate $\epsilon_0$ remains approximately constant between 1.0

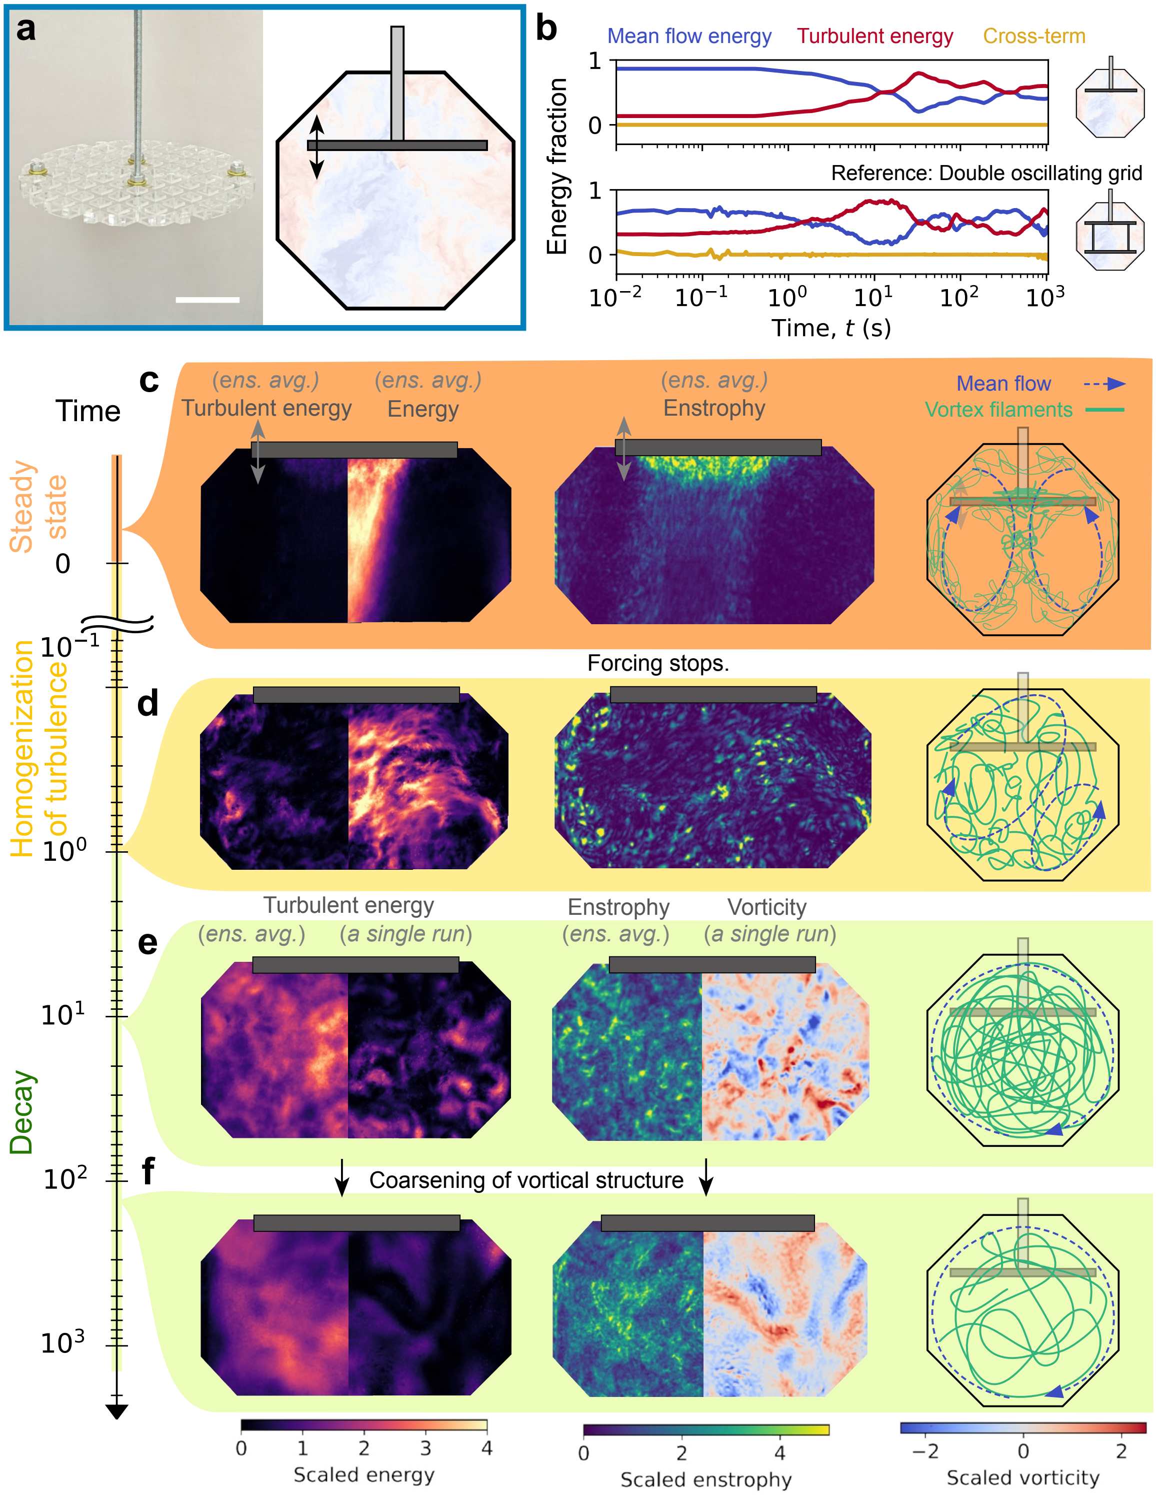


FIG. 21. **Temporal evolution of turbulence generated by a single oscillating grid.** (**a**) A single grid oscillates sinusoidally to agitate a fluid. The scale bar represents 50 mm. (**b**) The system's energy $\langle \mathbf{U}\cdot\mathbf{U}\rangle_n$ is divided into mean flow energy $\langle \mathbf{U}\rangle_n \cdot \langle \mathbf{U}\rangle$, turbulent energy $\langle \mathbf{u}\cdot\mathbf{u}\rangle_n$, and a cross-term $\langle \mathbf{U}\cdot\mathbf{u}\rangle_n$. The oscillation creates a substantial mean flow, whereas turbulence developing later. (**c-f**) The panels display how turbulence develops and decays. (**c**) Initially, energy is stored in a mean flow. (**d**) After the grid stops moving, turbulence develops as more mean flow energy converts into the fluctuating energy. Enstrophy becomes more homogeneous as it gets transported into the entire chamber. (**e-f**) Turbulence continues to decay, and its vortical structure coarsens over time.

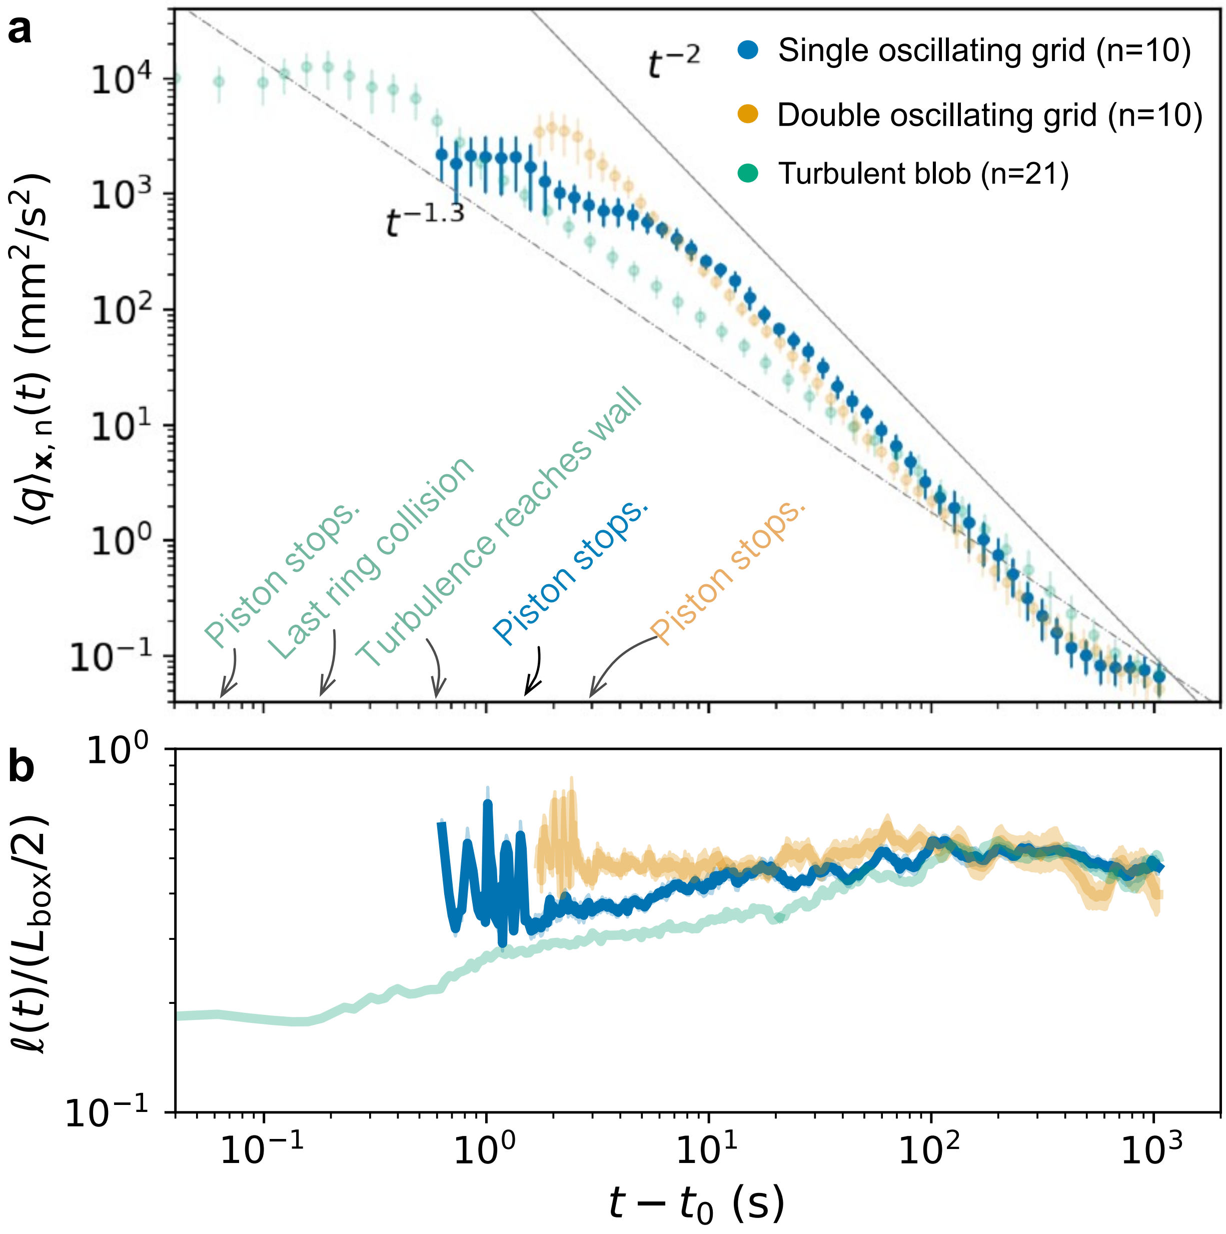


FIG. 22. **Turbulent energy decay and growth of integral length scale in single oscillating grid experiments.** **(a)** Turbulent energy exhibits a $t^{-2}$ power-law decay at late times ($t-t_0 > 10$ s; $t_0 = -1.63$ s), eventually reaching a steady state at $t - t_0 = 600$ s. Error bars represent the SEM ($n = 10$). **(b)** Evolution of the integral length scale demonstrates growth described by $\ell(t) = 0.33(t - t_0)^{0.10}$ for $1.5 < t - t_0 < 100$ s, saturating at $\ell \approx 0.26L_{\mathrm{box}}$.

and 1.2, and monotonically decreases as the Taylor Reynolds number drops to 10. These values are comparable to those extracted from the double oscillating grid and turbulent blob experiments (Supplementary Figure 23b).

Supplementary Figure 23c shows the dimensionless dissipation rate plotted against the Taylor Reynolds number, $Re_\lambda = u'\lambda/\nu$, where

$$\lambda = 15\frac{u'^3}{\epsilon} = -15u'^3\left(\frac{d\langle q\rangle_{\mathbf{x},\mathrm{n}}(t)}{dt}\right)^{-1}.$$

Figure 23d presents the rescaled three-dimensional energy spectra at different stages of decay, with the raw spectra shown in the inset. The energy spectra, $E(\kappa, t)$, and wavenumber, $\kappa$, are rescaled using the dissipation rate $\epsilon = -d\langle q\rangle_{\mathbf{x},\mathrm{n}}(t)/dt$ and Kolmogorov length scale $\eta = (\nu^3/\epsilon)^{1/4}$:

$$E(\kappa, t) \to \frac{E(\kappa, t)}{(\epsilon(t)\nu^5)^{1/4}}, \quad \kappa \to \kappa\eta.$$

The rescaled spectra follow the universal energy spectrum throughout the decay, as is the case for the double grid and turbulent blob experiments. The absence of the $-5/3$ law in the raw spectrum is attributed to the flow entering the dissipation range in the universal spectrum.

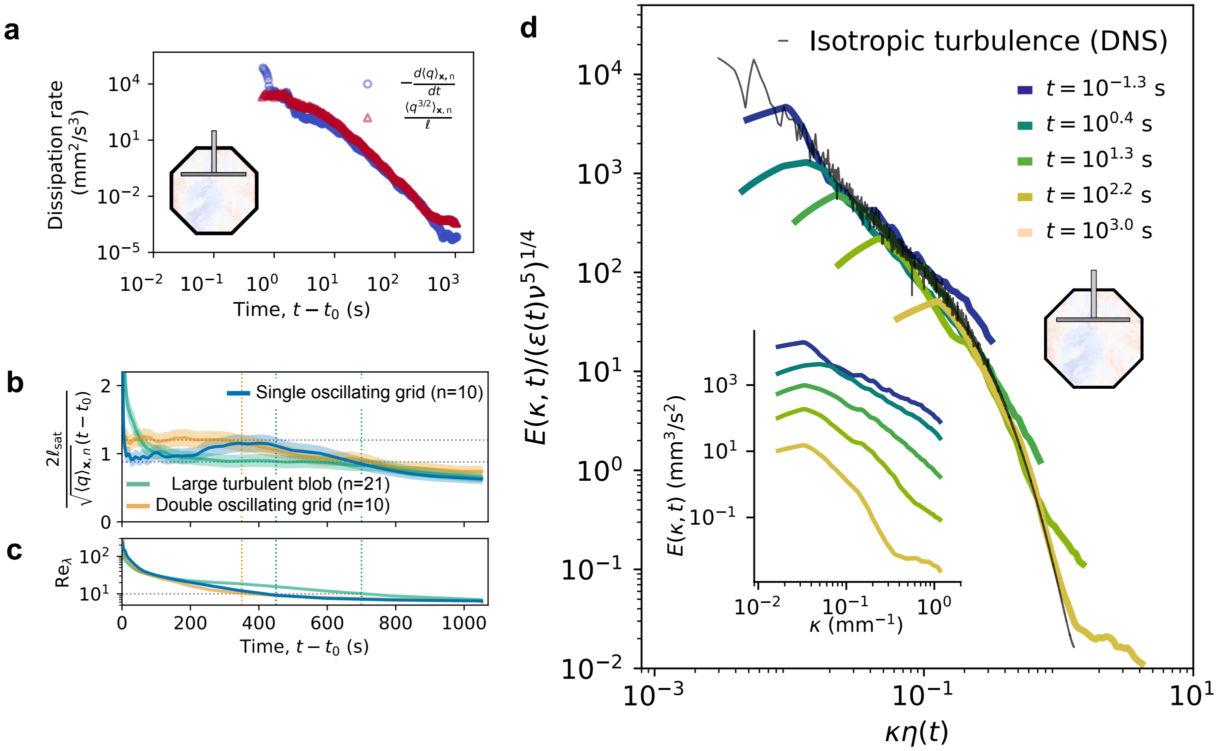


FIG. 23. **Dissipation rate and rescaled energy spectrum in the single oscillating grid experiments** (**a**) The dissipation rate $-d\langle q\rangle_{\mathbf{x}}/dt$ for turbulence initiated by the single oscillating grid confirms the scaling law $\langle q^{3/2}\rangle_{\mathbf{x},\mathrm{n}}/\ell$, consistent over an extensive duration over 500 seconds. (**b**) Estimate of dimensionless dissipation rate $\epsilon_0$ from the asymptotic form of $\langle q\rangle_{\mathbf{x},n}(t)$ and the saturated value of $\ell$ ($\ell_{\mathrm{sat}} = 0.25L_{\mathrm{Box}}$). (**c**) The Taylor Reynolds number drops below 10 when the estimated value of $\epsilon_0$ begins to decrease. The vertical lines indicate the times at which $\mathrm{Re}_\lambda$ reaches 10 for each experiment. (**d**) Rescaled three-dimensional energy spectra during decay; the inset shows spectra without rescaling, computed using the observed dissipation rate $\epsilon = -d\langle q\rangle_{\mathbf{x},\mathrm{n}}/dt$ and fluid viscosity $\nu$. The rescaled spectra align with the universal profile of isotropic turbulence (DNS) at $\mathrm{Re}_\lambda = 418$ [44]. Error bars in (b) represent the SEM.

## VIII. SUPPLEMENTARY MOVIES

Supplementary Movies are available at:
https://www.dropbox.com/scl/fo/c8ca8ysq6pp3fsiwr5gce/h?rlkey=ojtyw3t4squqmy5yuw1ck9mad&st=zx2l7z36&dl=0.

**Video 1: Expansion of a small turbulent blob ($Re_\lambda = 60$): energy**

This movie shows a two-dimensional slice of the measured turbulent kinetic energy field, ensemble-averaged (over 10 experimental runs), and scaled by its value in the central region:
$q/q_0 = \langle q(\mathbf{x}, t)\rangle_{n=10}/\langle q(r < 40 \text{ mm}, t)\rangle_{\mathbf{x},n=10}$. The top panel shows how the normalization factor, denoted as $q_0$, evolves over time. The shaded area marks the period during which vortex rings were injected to sustain the blob state. This movie shows that in the absence of forcing, the turbulent energy expands isotropically, transitioning to a more homogeneous turbulent state after the blob reaches the chamber walls $t = 6.5$ s. The initial Taylor Reynolds number within the blob is 60.

**Video 2: Expansion of a small turbulent blob ($Re_\lambda = 60$): enstrophy**

This movie shows a two-dimensional slice of the measured enstrophy field, ensemble-averaged (over 10 experimental runs), and scaled by its value in the central region:
$\omega_z^2/\omega_{z,0}^2 = \langle \omega_z^2(\mathbf{x}, t)\rangle_{n=10}/\langle \omega_{z,0}^2(r < 40 \text{ mm}, t)\rangle_{n=10}$. The top panel shows how the normalization factor, denoted as $\omega_{z,0}^2$, evolves over time. The shaded area marks the period during which vortex rings were injected to sustain the blob state. This movie shows that in the absence of forcing, the turbulent energy expands isotropically, transitioning to a more homogeneous turbulent state after the blob reaches the chamber walls $t = 6.5$ s. The initial Taylor Reynolds number within the blob is 60.

**Video 3: Evolution of rescaled energy spectrum during decay (Large blob, $Re_\lambda = 203$)**

This movie shows the temporal evolution of the three-dimensional energy spectrum during the decay of a large blob, supplementing main Figure 4d. It also shows the corresponding rescaled energy spectrum, computed using the dissipation rate $\epsilon(t) = -d\langle q\rangle_{\mathbf{x},\mathrm{n}}/dt$ from main Figure 2a, the kinematic viscosity of water $\nu = 1.002$ mm$^2$/s, and the Kolmogorov length scale $\eta(t) = (\nu^3/\epsilon(t))^{1/4}$. Remarkably, the rescaled spectra collapse onto a universal curve over an extended period, even as the Taylor-scale Reynolds number decreases to $\mathrm{Re}_\lambda \approx 10$ (main Figure 4b). This universal profile, derived from direct numerical simulations (DNS) of forced isotropic turbulence at $1024^3$ resolution ($\mathrm{Re}_\lambda \approx 418$) [44], is consistent with a range of experimental observations, including grid turbulence and turbulent boundary layers [43, 64]. At late times ($t - t_0 > 80$ s), the energy spectrum deviates from inertial scaling, $E(\kappa) \propto \kappa^{-5/3}$, as the turbulence enters the dissipation range.

**Video 4: Decay of a large turbulent blob ($Re_\lambda = 203$): energy**

This movie shows the evolution of ensemble-averaged, turbulent energy on the central slice during the decay of a large turbulent blob ($\mathrm{Re}_\lambda \approx 200$), supplementing main Figures 1 and 2 . The displayed field is normalized by the value of the energy averaged over ensembles and space $(1/2)\langle \mathbf{U} \cdot \mathbf{U}\rangle_{\mathbf{x},\mathrm{n}}$. The movie highlights that the blob rapidly expands within the first two seconds ($t - t_0 < 2$ s) and subsequently decays as approximately homogeneous turbulence over an extended

period ($t - t_0 > 2$ s). The spatially averaged turbulent energy is shown in parallel. Notably, the onset of the regime where the turbulent energy follows $q \sim t^{-2}$ scaling (around $t - t_0 \approx 100$ s) occurs well after the blob reaches the chamber wall ($t - t_0 \approx 2$ s).

**Video 5: Decay of a large turbulent blob ($Re_\lambda = 203$): enstrophy**

This movie shows the evolution of ensemble-averaged turbulent enstrophy on the central slice during the decay of a large turbulent blob ($\mathrm{Re}_\lambda = 203$) and supplements main text Figures 1 and 2. The field is normalized by the spatial and ensemble average, $\langle \omega_z^2 \rangle_{\mathbf{x},\mathrm{n}}$, where $\omega_z$ is the out-of-plane turbulent vorticity inferred from 2D velocity measurements. The spatial average is shown alongside. The turbulent enstrophy rapidly expands within the first two seconds ($t - t_0 < 2$ s), similar to turbulent energy, and then decays as approximately homogeneous turbulence ($t - t_0 > 2$ s). A horizontal band visible at late times ($t - t_0 > 80$ s) reflects inhomogeneous laser illumination, which reduces the signal-to-noise ratio outside the band and may lead to overestimated vorticity.

**Video 6: Decomposition of energy and enstrophy into mean and fluctuating components (Large blob, $Re_\lambda = 203$)**

This movie displays the spatiotemporal evolution of several flow components during the decay of a large blob ($Re_\lambda = 203$). Most of the energy resides in the fluctuating field up to $t - t_0 \leq 500$ s, while the enstrophy remains dominated by fluctuations throughout the decay. A large, irrotational vortex emerges at $t - t_0 \gtrsim 150$ s, most clearly visible in the mean-flow energy field. Each energy and enstrophy field (raw, mean-flow, and fluctuating) is normalized by the ensemble- and spatial-average of the raw (i.e., undecomposed) field. This normalization allows direct visual comparison of the relative strength of the mean and fluctuating components over time. To produce this movie, the velocity field in each of the $n = 21$ recordings was decomposed into mean and fluctuating components. From these, the raw, mean-flow, and fluctuating energy fields were computed; enstrophy fields were derived from the corresponding vorticity. All fields were then ensemble-averaged. This movie supplements main Figures 1, 2, and 3b, as well as Supplementary Videos 4 and 5.

**Video 7: Spatiotemporal evolution of mean flow energy (Large Blob, $Re_\lambda = 203$)**

This movie shows the evolution of the mean flow on the central slice of the large turbulent blob. Early on ($t - t_0 \leq 0.5$ s), a four-fold ejection pattern emerges from vortex ring collisions. During the intermediate period, the mean flow appears largely structureless. At later times ($t - t_0 \geq 150$ s), it transitions into a single chamber-filling vortex. The movie supplements Supplementary Video 7, where the fluctuating field dominates and obscures the mean flow pattern. The mean-flow energy in this movie is defined as $\mathcal{E}(\mathbf{x}, t) = (1/2)\langle \mathbf{U} \rangle_\mathrm{n} \cdot \langle \mathbf{U} \rangle_\mathrm{n}$. The field is shown on the central slice and scaled by its spatial average, $\mathcal{E}_s(t) = (1/2)\langle \langle \mathbf{U} \rangle_\mathrm{n} \cdot \langle \mathbf{U} \rangle_\mathrm{n} \rangle_\mathbf{x}$, to emphasize the evolving structure of the mean flow.

**Video 8: Pathline visualization of a decaying turbulent blob (Large blob, $Re_\lambda = 203$)**

This movie shows the decay of the large turbulent blob (initially of radius $R = 60$ mm), over a duration of 17 minutes. Fluorescent tracer particles ($R = 100$ $\mu$m) were suspended in the chamber, and each frame of the movie is generated by overlaying 20 consecutive frames from the "logarithmic" acquisition described in §IV A 4 in the Supplementary Information. The visualization displays the

2D pathlines of particles illuminated by a laser sheet. In the early stages ($t - t_0 < 5$ s), the high-speed, three-dimensional motions within the blob produce blurred regions with no visible streaks at the center. As the turbulence decays, vortical structures coarsen—visibly confirmed by the growth of average eddy size, making their structure readily identifiable through their pathlines in the illuminated plane. During the decay process, the eddy-turnover time $\ell/u'$ increases significantly from $O(10^{-1})$ s to $O(10^2)$ s. This dataset is one of the 21 recordings of large-blob decay used in the analysis presented in Figures 1 and 2.

**Video 9: Decay of turbulence initiated by a double oscillating grid ($Re_\lambda = 185$): energy**

This movie shows how the turbulent kientic energy, initiated by a double oscillating grid, evolves into a nearly homogeneous state after the grid stops at $t - t_0 \approx 2$ s. The turbulent energy field exhibits temporal oscillations, reflecting energy exchange between the mean flow and fluctuations, as shown in main Figure 3b. The spatially averaged turbulent energy follows the decay law $\langle q \rangle_{\mathbf{x},\mathrm{n}} \sim t^{-2}$. The movie supplements main Figures 2 and 3. and presents ensemble-averaged turbulent energy on the central slice during the decay. The field is normalized by the ensemble- and spatial-average value, $(1/2)\langle \mathbf{U} \cdot \mathbf{U} \rangle_{\mathbf{x},\mathrm{n}}$.

**Video 10: Decay of turbulence initiated by a double oscillating grid ($Re_\lambda = 185$): enstrophy**

This movie shows how the enstrophy of the turbulent flow, initiated by a double oscillating grid, evolves into a nearly homogeneous state after the grid stops at $t - t_0 \approx 2$ s. Turbulent enstrophy is initially generated near the boundaries of the moving grids and advected into the chamber by the mean flow, eventually becoming more uniformly distributed by $t - t_0 \approx 5$ s. In the late stages ($t - t_0 > 500$ s), most of the enstrophy is concentrated along a line near the left wall of the chamber due to a localized hot spot from the laser sheet illumination. This movie supplements main Figures 3c–f and presents ensemble-averaged turbulent enstrophy on the central slice during the decay. The field is normalized by the ensemble- and spatial-average value, $\langle \Omega_z^2 \rangle_{\mathbf{x},\mathrm{n}}$, where $\Omega_z$ is the out-of-plane vorticity $\Omega_z = (\nabla \times \mathbf{U})_z$ computed from the in-plane velocity field $\mathbf{U}(\mathbf{x})$. The spatially-averaged turbulent enstrophy is also shown to indicate the continued decay of enstrophy throughout the chamber.

**Video 11: Decomposition of energy and enstrophy fields into mean flow and fluctuations (Double oscillating grid, $Re_\lambda = 185$)**

This movie displays the spatiotemporal evolution of several flow components during the decay of the flow set up by a double oscillating grid. The turbulent energy, initially concentrated in the mean-flow field, gradually shifts to the fluctuating field during the decay of turbulence generated by a double oscillating grid. In contrast to the large blob case, the mean-flow energy dominates at early times. The energy partition oscillates over time (main Figure 3b), with fluctuating energy becoming dominant around $t - t_0 \approx 20$ s. A large clockwise vortex forms at $t - t_0 \approx 50$ s and gradually dissipates by $t - t_0 \approx 700$ s. Turbulent enstrophy, in contrast, becomes approximately homogeneous shortly after the grid stops moving and remains dominated by fluctuations throughout the decay. This movie supplements main Figures 3b–f and displays raw, mean-flow, and fluctuating energy and enstrophy fields on the central slice. Each field is computed from $n = 10$ recordings, with the velocity field in each decomposed into mean and fluctuating components. Vorticity was derived from the in-plane velocity field, and all fields were ensemble-averaged.

**Video 12: Evolution of rescaled energy spectrum during decay (Double oscillating grid, $Re_\lambda = 185$)**

This movie shows the temporal evolution of the three-dimensional energy spectrum from turbulence initiated by a double oscillating grid, supplementing main Figure 4e. It also shows the corresponding rescaled energy spectrum, computed using the dissipation rate $\epsilon(t) = -d\langle q\rangle_{\mathbf{x},\mathrm{n}}/dt$ from main Figure 2a, the kinematic viscosity of water $\nu = 1.002$ mm$^2$/s, and the Kolmogorov length scale $\eta(t) = (\nu^3/\epsilon(t))^{1/4}$. Remarkably, the rescaled spectra collapse onto a universal curve over an extended period, even as the Taylor-scale Reynolds number decreases to $\mathrm{Re}_\lambda \approx 10$, as shown in main Figure 4b. This universal profile, calculated from direct numerical simulations (DNS) of forced isotropic turbulence at $1024^3$ resolution ($\mathrm{Re}_\lambda \approx 418$) [44], is consistent with a range of experimental observations, including grid turbulence and turbulent boundary layers [43, 64]. At late times ($t - t_0 > 80$ s), the energy spectrum deviates from Kolmogorov scaling, $E(\kappa) \propto \kappa^{-5/3}$, as the rescaled energy spectrum indicates that the system enters the dissipation range.

**Video 13: Spatiotemporal evolution of mean flow energy (Double oscillating grid, $Re_\lambda = 185$)**

This movie shows the evolution of the mean flow on a central slice during the decay of turbulence from a double oscillating grid. Initially ($t - t_0 < 1.5$ s), the mean flow displays a quadrupolar structure due to vertical grid motion, with stronger circulation near the bottom (see main Figure 3c). After the forcing stops, it transitions to a dipole ($10 \lesssim t - t_0 \lesssim 30$ s), then to a single large vortex ($40 \lesssim t - t_0 \lesssim 700$ s). At late times, this vortex fades, and energy appears concentrated near the left wall due to a laser sheet illumination hot spot. The movie supplements Supplementary Video 11, where the mean-flow energy is less visible due to dominance by fluctuations. Here, the mean-flow energy $\mathcal{E} = (1/2)\langle \mathbf{U}\rangle_n \cdot \langle \mathbf{U}\rangle_n$ is shown on the central slice and scaled by its spatial average to highlight structural evolution.

**Video 14: Spatiotemporal evolution of mean flow energy (Single oscillating grid, $Re_\lambda = 95$)**

This movie shows the evolution of mean-flow energy on a central slice during the decay of turbulence from a single oscillating grid. The single oscillating grid generates a unidirectional mean flow, providing a third system to assess how initial flow structure influences the decay process. A detailed analysis of energy decay and integral length scale is provided in §VII of the Supplementary Information. Unlike the large blob and double-grid cases, asymmetric forcing from the single grid produces a strong downward flow that rapidly redistributes energy and enstrophy across the chamber ($t - t_0 \approx 5$ s). The system then evolves into a single vortex state ($100 \lesssim t - t_0 \lesssim 400$ s), which fades at later times. As in previous cases, an apparent energy concentration near the left wall arises from a localized hot spot in the laser sheet illumination.

**Video 15: 3D pathline visualization of an expanding and decaying turbulent blob (small blob, $Re_\lambda = 60$)**

This movie shows the expansion and decay of a small turbulent blob (initially of radius $R = 40$ mm) over a 17-minute duration. Fluorescent tracer particles ($R = 100$ $\mu$m) were suspended in the chamber and tracked using 3D Particle Tracking Velocimetry (PTV). During the recording, the frame rate was varied to account for the slowing motions, as illustrated by the plot at the top of the movie. The moving band indicates the time window corresponding to the displayed pathlines.

Abrupt changes in frame rate may result in trajectory loss, which appears as voids or sudden changes in color and pathline lengths. Each frame of the movie shows pathlines of 10,000–20,000 particles over 39 consecutive frames. The movie first shows turbulence confined by injected vortex loops, then its expansion ($1 < t - t_0 < 5$ s), and the coarsening of vortical structures. In the late stages ($300 < t - t_0 < 800$ s), a few large vortices stir the fluid in the flow chamber, slowly changing their axes of rotation.

---


[1] M. Gharib, E. Rambod, and K. Shariff, A universal time scale for vortex ring formation, Journal of Fluid Mechanics **360**, 121–140 (1998).

[2] T. Matsuzawa, N. P. Mitchell, S. Perrard, and W. T. Irvine, Creation of an isolated turbulent blob fed by vortex rings, Nature Physics , 1 (2023).

[3] A. N. Kolmogorov, Equations of motion of an incompressible turbulent fluid, Izv Akad Nauk SSSR Ser Phys **6**, 56 (1942).

[4] H. W. Emmons, Shear flow turbulence, in *Proceedings of the 2nd US Congress of Applied Mechanics, ASME* (1954).

[5] P. Bradshaw, D. H. Ferriss, and N. P. Atwell, Calculation of boundary-layer development using the turbulent energy equation, Journal of Fluid Mechanics **28**, 593 (1967).

[6] F. H. Harlow and P. I. Nakayama, Turbulence transport equations, Physics of Fluids **10**, 2323 (1967).

[7] P. Saffman, A model for inhomogeneous turbulent flow, Proceedings of the Royal Society of London Series A **317**, 417 (1970).

[8] W. Rodi and D. B. Spalding, A two-parameter model of turbulence, and its application to free jets, Waerme und Stoffuebertragung **3**, 85 (1970).

[9] G.-I. Barenblatt, Self-similar turbulence propagation from an instantaneous point source, in *Non-Linear Dynamics and Turbulence*, Vol. 48, edited by G. I. Barenblatt, G. Iooss, and D. D. Joseph (Pitman, 1983).

[10] G. Barenblatt, N. Galerkina, and M. Luneva, Evolution of a turbulent burst, Journal of engineering physics **53**, 1246 (1987).

[11] G. I. Barenblatt, *Scaling, self-similarity, and intermediate asymptotics* (Cambridge University Press, 1996).

[12] L.-Y. Chen and N. Goldenfeld, Renormalization-group theory for the propagation of a turbulent burst, Physical Review A **45**, 5572 (1992).

[13] P. A. Davidson, *Turbulence: an introduction for scientists and engineers* (Oxford university press, 2015).

[14] M. R. Smith, R. J. Donnelly, N. Goldenfeld, and W. Vinen, Decay of vorticity in homogeneous turbulence, Physical review letters **71**, 2583 (1993).

[15] S. Kamin and J. L. Vazquez, The propagation of turbulent bursts, European Journal of Applied Mathematics **3**, 263 (1992).

[16] S. Hastings, On a self-similar solution for the decay of turbulent bursts, European Journal of Applied Mathematics **3**, 319 (1992).

[17] F. Q. Gracián and J. L. Vázquez, Self-similar turbulent bursts: existence and analytic dependence, Differential and Integral Equations **8**, 1677 (1995).

[18] N. Goldenfeld, O. Martin, Y. Oono, and F. Liu, Anomalous dimensions and the renormalization group in a nonlinear diffusion process, Physical Review Letters **64**, 1361 (1990).

[19] N. Goldenfeld, *Lectures on phase transitions and the renormalization group* (CRC Press, 2018).

[20] M. R. Smith, A study of homogeneous turbulence using superfluid helium, Physica B: Condensed Matter **197**, 297 (1994).

[21] T. P. Witelski and A. J. Bernoff, Self-similar asymptotics for linear and nonlinear diffusion equations, Studies in Applied Mathematics **100**, 153 (1998).

[22] J. L. Vázquez, *The porous medium equation: mathematical theory* (Oxford University Press, 2006).

[23] Y. Oono and S. Puri, Study of phase-separation dynamics by use of cell dynamical systems. i. modeling, Physical Review A **38**, 434 (1988).

[24] Y. Oono and S. Puri, Computationally efficient modeling of ordering of quenched phases, Physical review letters **58**, 836 (1987).
[25] A. Shinozaki and Y. Oono, Spinodal decomposition in 3-space, Physical Review E **48**, 2622 (1993).
[26] M. Mondello and N. Goldenfeld, Scaling and vortex dynamics after the quench of a system with a continuous symmetry, Physical Review A **42**, 5865 (1990).
[27] M. Mondello and N. Goldenfeld, Scaling and vortex-string dynamics in a three-dimensional system with a continuous symmetry, Physical Review A **45**, 657 (1992).
[28] F. Liu, M. Mondello, and N. Goldenfeld, Kinetics of the superconducting transition, Physical Review Letters **66**, 3071 (1991).
[29] M. Zapotocky, P. M. Goldbart, and N. Goldenfeld, Kinetics of phase ordering in uniaxial and biaxial nematic films, Physical Review E **51**, 1216 (1995).
[30] N. Goldenfeld, P. Chan, and J. Veysey, Dynamics of precipitation pattern formation at geothermal hot springs., Physical Review Letters **96**, 254501 (2006).
[31] P. Y. Chan and N. Goldenfeld, Steady states and linear stability analysis of precipitation pattern formation at geothermal hot springs, Physical Review E **76**, 046104 (2007).
[32] J. Veysey II and N. Goldenfeld, Watching rocks grow, Nature physics **4**, 310 (2008).
[33] H. Tomita, Preservation of isotropy at the mesoscopic stage of phase separation processes, Progress of theoretical physics **85**, 47 (1991).
[34] S. P. Thampi, S. Ansumali, R. Adhikari, and S. Succi, Isotropic discrete laplacian operators from lattice hydrodynamics, Journal of Computational Physics **234**, 1 (2013).
[35] R. J. LeVeque, *Finite volume methods for hyperbolic problems*, Vol. 31 (Cambridge university press, 2002).
[36] M. J. Berger and J. Oliger, Adaptive mesh refinement for hyperbolic partial differential equations, Journal of computational Physics **53**, 484 (1984).
[37] M. Raffel, C. E. Willert, F. Scarano, C. J. Kähler, S. T. Wereley, and J. Kompenhans, *Particle Image Velocimetry: A Practical Guide* (springer, 2018) oCLC: 1035110003.
[38] J. Panickacheril John, D. A. Donzis, and K. R. Sreenivasan, Laws of turbulence decay from direct numerical simulations, Philosophical Transactions of the Royal Society A **380**, 20210089 (2022).
[39] W. K. George, The decay of homogeneous isotropic turbulence, Physics of Fluids A: Fluid Dynamics **4**, 1492 (1992).
[40] D. Schanz, S. Gesemann, and A. Schröder, Shake-The-Box: Lagrangian particle tracking at high particle image densities, Experiments in Fluids **57**, 70 (2016).
[41] J. de Jong, L. Cao, S. H. Woodward, J. P. L. C. Salazar, L. R. Collins, and H. Meng, Dissipation rate estimation from PIV in zero-mean isotropic turbulence, Experiments in Fluids **46**, 499 (2008).
[42] S. B. Pope, *Turbulent flows* (Cambridge University Press, Cambridge ; New York, 2000).
[43] S. G. Saddoughi and S. V. Veeravalli, Local isotropy in turbulent boundary layers at high reynolds number, Journal of Fluid Mechanics **268**, 333–372 (1994).
[44] Y. Li, E. Perlman, M. Wan, Y. Yang, C. Meneveau, R. Burns, S. Chen, A. Szalay, and G. Eyink, A public turbulence database cluster and applications to study lagrangian evolution of velocity increments in turbulence, Journal of Turbulence , N31 (2008).
[45] K. R. Sreenivasan, On the scaling of the turbulence energy dissipation rate, The Physics of fluids **27**, 1048 (1984).
[46] K. R. Sreenivasan, An update on the energy dissipation rate in isotropic turbulence, Physics of Fluids **10**, 528 (1998).
[47] J. C. Vassilicos, Dissipation in turbulent flows, Annual review of fluid mechanics **47**, 95 (2015).
[48] G. Barenblatt and N. Goldenfeld, Does fully developed turbulence exist? reynolds number independence versus asymptotic covariance, Physics of fluids **7**, 3078 (1995).
[49] W. Baines and E. Peterson, An investigation of flow through screens, Transactions of the American Society of Mechanical Engineers **73**, 467 (1951).
[50] J. Bennett and S. Corrsin, Small reynolds number nearly isotropic turbulence in a straight duct and a contraction, The Physics of Fluids **21**, 2129 (1978).
[51] G. K. Batchelor and A. A. Townsend, Decay of turbulence in the final period, Proceedings of the Royal Society of London. Series A. Mathematical and Physical Sciences **194**, 527 (1948).
[52] S. Corrsin, *Decay of turbulence behind three similar grids*, Ph.D. thesis, California Institute of Technology (1942).

[53] R. W. Stewart and A. A. Townsend, Similarity and self-preservation in isotropic turbulence, Philosophical Transactions of the Royal Society of London. Series A, Mathematical and Physical Sciences **243**, 359 (1951).

[54] R. Mills Jr, A. Kistler, V. O'brien, and S. Corrsin, *Turbulence and temperature fluctuations behind a heated grid*, Tech. Rep. (National Advisory Committee for Aeronautics, 1958).

[55] T. Yeh and C. Atta, Spectral transfer of scalar and velocity fields in heated-grid turbulence, Journal of Fluid Mechanics **58**, 233 (1973).

[56] L. B. Esteban, J. Shrimpton, and B. Ganapathisubramani, Laboratory experiments on the temporal decay of homogeneous anisotropic turbulence, Journal of Fluid Mechanics **862**, 99 (2019).

[57] G. Comte-Bellot and S. Corrsin, Simple eulerian time correlation of full-and narrow-band velocity signals in grid-generated,'isotropic'turbulence, Journal of fluid mechanics **48**, 273 (1971).

[58] J.-B. Gorce and E. Falcon, Freely decaying saffman turbulence experimentally generated by magnetic stirrers, Physical Review Letters **132**, 264001 (2024).

[59] S.-C. Lin and S.-C. Lin, Study of strong temperature mixing in subsonic grid turbulence, The Physics of Fluids **16**, 1587 (1973).

[60] L. Mydlarski and Z. Warhaft, On the onset of high-reynolds-number grid-generated wind tunnel turbulence, Journal of Fluid Mechanics **320**, 331 (1996).

[61] S. R. Stalp, L. Skrbek, and R. J. Donnelly, Decay of grid turbulence in a finite channel, Physical review letters **82**, 4831 (1999).

[62] A. Kistler and T. Vrebalovich, Grid turbulence at large reynolds numbers, Journal of Fluid Mechanics **26**, 37 (1966).

[63] M. Gad-el Hak and S. Corrsin, Measurements of the nearly isotropic turbulence behind a uniform jet grid, Journal of Fluid Mechanics **62**, 115 (1974).

[64] N. D. Katopodes, Chapter 8 - turbulent flow, in *Free-Surface Flow*, edited by N. D. Katopodes (Butterworth-Heinemann, 2019) pp. 566–650.
